# Supplementary material for: Partial Synchrony for Free? New Upper Bounds for Byzantine Agreement
Source: arXiv:2402.10059 source file (2024-10-23)
Supplement: Supplementary file 1 [file asynchronous_in_synchrony.tex]

\section{Asynchronous Algorithms in Synchrony: Translating Time Complexity}

In this section, we show how the time complexity of asynchronous algorithms translates when those algorithms are run in a synchronous environment (e.g., after GST).
We fix an asynchronous algorithm $\mathcal{A}$; let $\mathit{execs}(\mathcal{A})$ denote the set of all executions of $\mathcal{A}$.
% which allows processes to start and stop executing it by invoking the $\mathsf{start}()$ and $\mathsf{stop}()$ operations.
First, we define the time complexity of $\mathcal{A}$.

\begin{definition} [Time complexity of $\mathcal{A}$]
Let $\mathcal{E}$ be any execution of $\mathcal{A}$.
The time complexity of $\mathcal{E}$ is defined as the length $x$ of the longest sequence of messages $m_1, ..., m_x$ sent by correct processes whose sending events are causally related, i.e., for each $i \in [2, x]$, the reception of $m_{i - 1}$ is a requirement for sending of $m_i$.
Then, the \emph{time complexity} of $\mathcal{A}$ is defined as 
\begin{equation*}
    \max_{\mathcal{E} \in \mathit{execs}(\mathcal{A})}\bigg\{\text{the time complexity of } \mathcal{E} \bigg\}.
\end{equation*}
\end{definition}
We denote by $\mathcal{T}$ the time complexity of $\mathcal{A}$.

For each execution $\mathcal{E} \in \mathit{execs}(\mathcal{A})$ and each message $m$ sent by a correct process in $\mathcal{E}$, we define the \emph{rank} of $m$ in $\mathcal{E}$ (in short, $\mathit{rank}(m, \mathcal{E})$) in the following way:
\begin{compactitem}
    \item If the sender of $m$ receives no messages sent by correct processes before sending $m$, $\mathit{rank}(m, \mathcal{E}) = 1$.

    \item Otherwise, let $\mathcal{M}$ denote the set of all messages sent by correct processes that are received before sending $m$, and let $r$ denote the greatest rank among messages in $\mathcal{M}$.
    Then, $\mathit{rank}(m, \mathcal{E}) = r + 1$.
\end{compactitem}
Observe that, for any execution $\mathcal{E} \in \mathit{execs}(\mathcal{A})$, if a correct process receives any message $m$ sent by a correct process, then $\mathit{rank}(m, \mathcal{E}) \leq \mathcal{T}$.
(Recall that $\mathcal{T}$ denotes the time complexity of $\mathcal{A}$.)

The following definition introduces the concept of a quasi-synchronous execution of $\mathcal{A}$.
Quasi-synchronous executions play a major role in ensuring the termination property of \name.

\begin{definition} [Quasi-synchronous execution of $\mathcal{A}$]
An execution $\mathcal{E}$ of $\mathcal{A}$ is said to be \emph{quasi-synchronous} if and only if the following conditions are satisfied:
\begin{compactitem}
    \item The first correct process to start executing $\mathcal{A}$ in $\mathcal{E}$ does so at some time $t \geq \text{GST}$.

    \item All correct processes start executing $\mathcal{A}$ by time $t + 4\delta$.
\end{compactitem}
\end{definition}

Finally, we are ready to introduce the main result this section aims to prove.

\begin{lemma} \label{lemma:quasi_synchronous_time}
In any quasi-synchronous execution $\mathcal{E}$ of $\mathcal{A}$, every correct process terminates by time $t + 4\delta + \mathcal{T}$, where $t$ denotes the first time a correct process starts executing $\mathcal{A}$ in $\mathcal{E}$.
\end{lemma}

\paragraph{Proof of \Cref{lemma:quasi_synchronous_time}.}
Let us fix any quasi-synchronous execution $\mathcal{E}$; we denote by $t$ the first time a correct process starts executing $\mathcal{A}$ in $\mathcal{E}$.
We start by proving that every message $m$ with $rank(m, \mathcal{E}) = 1$ is sent in $\mathcal{E}$ by time $t + 4\delta$.

\begin{lemma}
Let $m$ be any message sent by a correct process in $\mathcal{E}$ such that $\mathit{rank}(m, \mathcal{E}) = 1$.
Then, $m$ is sent by time $t + 4\delta$.
\end{lemma}
\begin{proof}
To prove the lemma, we prove that any correct process $p_i$ sends every its message $m$ with $\mathit{rank}(m, \mathcal{E}) = 1$ immediately upon starting its execution of $\mathcal{A}$ in $\mathcal{A}$.
By contradiction, let there exists a message $m$ sent by $p_i$ in $\mathcal{E}$ such that (1) $\mathit{rank}(m, \mathcal{E}) = 1$, and (2) $m$ is \emph{not} sent upon starting $\mathcal{A}$.
As $m$ is not sent upon starting $\mathcal{A}$, $p_i$ has previously received a message 

suppose that $p_i$ sends some message $m$ in $\mathcal{E}$ with $\mathit{rank}$
\end{proof}
