# Supplementary material for: Partial Synchrony for Free? New Upper Bounds for Byzantine Agreement
Source: arXiv:2402.10059 source file (2024-10-23)
Supplement: Supplementary file 2 [file classification_extended.tex]

\section{Extended Formalism: Classification \& Triviality if $n \leq 3t$} \label{section:classification_extended}

This section classifies all validity properties (expressed using the extended formalism) in solvable and unsolvable ones.
Moreover, we show that any solvable validity property with $n \leq 3t$ is trivial.
We underline that this section restates the results presented in the main body of the paper; however, we now consider the extended formalism.
Wherever suitable, we will reuse the (intermediate) results of the main body of the paper.

We start this section by proving that the canonical similarity result, which is a critical intermediate result, holds in the extended formalism (\Cref{subsection:intermediate_results_extended_formalism}). 
Then, we introduce the similarity condition, and show its necessity for solvable validity properties (\Cref{subsection:necessary_condition_extended}).
Next, we prove that all solvable validity properties with $n \leq 3t$ are trivial (\Cref{subsection:triviality_extended}).
Finally, we prove that the similarity condition is sufficient for solvable validity properties if $n > 3t$ (\Cref{subsection:sufficient_extended}).

\subsection{Canonical Similarity} \label{subsection:intermediate_results_extended_formalism}

This subsection shows that the canonical similarity result is satisfied even in the extended formalism.
Recall that this result holds in the original formalism (see \Cref{subsection:intermediate_results}).
We emphasize that the original proof (with minor modifications) suffices for proving the result in the extended formalism.
However, for the sake of completeness, we restate the lemma and the proof below.

\begin{lemma_helper} [restated in the extended formalism]
Let $\mathit{val}$ be any solvable validity property and let $\mathcal{A}$ be any algorithm which solves the Byzantine consensus problem with $\mathit{val}$.
% Byzantine consensus algorithm with $\mathit{val}$.
Let $\mathcal{E} \in \mathit{execs}(\mathcal{A})$ be any infinite canonical execution and let $\mathsf{corresponding}(\mathcal{E}) = c$, for some input configuration $c \in \mathcal{I}$.
If a value $v' \in \mathcal{V}_O$ is decided by a correct process in $\mathcal{E}$, then $v' \in \bigcap\limits_{c' \in \mathit{sim}(c)} \mathit{val}(c')$.
\end{lemma_helper}
\begin{proof}
By contradiction, suppose that $v' \notin \bigcap\limits_{c' \in \mathit{sim}(c)} \mathit{val}(c')$.
Hence, there exists an input configuration $c' \in \mathcal{I}$ such that (1) $c \leftsquigarrow c'$, and (2) $v' \notin \mathit{val}(c')$.
Let $P$ be any process such that $P \in \processes{c'} \cap \processes{c}$; such a process exists as $c \leftsquigarrow c'$.
As $\mathcal{A}$ satisfies \emph{Termination} and \emph{Agreement}, $\mathcal{E}$ is an infinite execution, and $P$ is correct in $\mathcal{E}$, $P$ decides $v'$ in $\mathcal{E}$.

We construct another execution $\mathcal{E}' \in \mathit{execs}(\mathcal{A})$ such that $\mathsf{corresponding}(\mathcal{E}') = c'$:
\begin{compactenum}
    \item The adversary pool in $\mathcal{E}'$ is $\mathsf{pool}(c')$.

    \item $\mathcal{E}'$ is identical to $\mathcal{E}$ until process $P$ decides $v'$.
    
    \item After $P$ has decided, all processes which are faulty according to $c'$ (processes in $\Pi \setminus{\processes{c'}}$) crash.
    
    \item All processes which are correct according to $c'$ and faulty according to $c$ (processes in $\processes{c'} \setminus{\processes{c}}$) ``wake up'' with the proposals specified in $c'$.
    
    \item GST is set to after all processes in $\processes{c'}$ have taken a computational step.
\end{compactenum}
For every process $P_i \in \processes{c'} \cap \processes{c}$, the proposal of $P_i$ in $\mathcal{E}'$ is $\mathsf{proposal}(c'[i])$; recall that $c'[i] = c[i]$ as $c \leftsquigarrow c'$.
Moreover, for every process $P_j \in \processes{c'} \setminus{\processes{c}}$, the proposal of $P_j$ in $\mathcal{E}'$ is $\mathsf{proposal}(c'[j])$ (step 4 of the construction).
Finally, the adversary pool in $\mathcal{E}'$ is $\mathsf{pool}(c')$ (step 1 of the construction); recall that, for every $P_j \in \processes{c} \setminus{\processes{c'}}$, $\mathsf{proposal}(c[j]) \in \mathsf{pool}(c')$ (as $c \leftsquigarrow c'$).
Hence, $\mathsf{corresponding}(\mathcal{E}') = c'$.
Furthermore, process $P$, which is correct in $\mathcal{E}'$, decides a value $v' \notin \mathit{val}(c')$ (step 2 of the construction).
Thus, we reach a contradiction with the fact that $\mathcal{A}$ satisfies $\mathit{val}$.
% , which proves the lemma.
\end{proof}

\subsection{Similarity Condition: Necessary Condition for Solvable Validity Properties} \label{subsection:necessary_condition_extended}

In this subsection, we (re)introduce the similarity condition (we define it in the extended formalism).\footnote{Recall that the similarity condition was previously introduced in the original formalism (see \Cref{subsection:necessary_condition}).}
We show that the similarity condition must be satisfied by all solvable validity properties.
Let us start by formally defining the similarity condition.

\begin{definition} [Similarity condition in the extended formalism] \label{definition:similarity_condition_extended}
A validity property $\mathit{val}$ satisfies the \emph{similarity condition} ($\mathcal{C}_S$, in short) if and only if there exists a computable function $\Lambda: \mathcal{I}_{n - t} \to \mathcal{V}$ such that:
\begin{equation*}
 \forall c \in \mathcal{I}_{n - t}: \Lambda(c) \in \mathsf{discover}\big( \mathsf{correct\_proposals}(c) \big) \cap \bigcap\limits_{c' \in \mathit{sim}(c)} \mathit{val}(c').
\end{equation*}
\end{definition}

$\mathcal{C}_S$ states that, for every input configuration $c$ with \emph{exactly} $n - t$ correct processes, there exists a computable function which retrieves a value $v$ such that (1) $v$ is discoverable using only the proposals of correct processes (according to $c$), and (2) $v$ is a common admissible decision among all input configurations which are similar to $c$.
\Cref{lemma:helper_main} plays the crucial role in proving the necessity of $\mathcal{C}_S$.
The proof of the theorem below is extremely similar to the proof from the main body of the paper.

\begin{theorem_necessity} (restated in the extended formalism)
\label{theorem:similarity_necessary_extended}
Any solvable validity property satisfies $\mathcal{C}_S$.
\end{theorem_necessity}
\begin{proof}
Let, by contradiction, there exist a validity property $\mathit{val}$ such that (1) $\mathit{val}$ does not satisfy $\mathcal{C}_S$, and (2) $\mathit{val}$ is solvable.
Let $\mathcal{A}$ be any Byzantine consensus algorithm with $\mathit{val}$.
As $\mathit{val}$ does not satisfy $\mathcal{C}_S$, there does not exist a computable function $\Lambda: \mathcal{I}_{n - t} \to \mathcal{V}_O$ such that, for every input configuration $c \in \mathcal{I}_{n - t}$, $\Lambda(c) \in \mathsf{discover}\big( \mathsf{correct\_proposals}(c) \big) \cap \bigcap\limits_{c' \in \mathit{sim}(c)} \mathit{val}(c')$ (by \Cref{definition:similarity_condition_extended}).

Fix any input configuration $\mathit{base} \in \mathcal{I}_{n - t}$ for which $\Lambda(\mathit{base})$ is not defined or not computable; such an input configuration exists as $\mathit{val}$ does not satisfy $\mathcal{C}_S$.
Let $\mathcal{E} \in \mathit{execs}(\mathcal{A})$ be any infinite canonical execution such that $\mathsf{corresponding}(\mathcal{E}) = \mathit{base}$.
As $\mathcal{A}$ satisfies \emph{Termination} and $\mathcal{E}$ is an infinite execution, some value $v \in \mathcal{V}_O$ is decided by a correct process in $\mathcal{E}$.
By \Cref{lemma:helper_main} and \Cref{assumption:extended}, $v \in \mathsf{discover}\big( \mathsf{correct\_proposals}(\mathit{base}) \big) \cap \bigcap\limits_{c' \in \similar{\mathit{base}}} \mathit{val}(c')$.
Hence, $\Lambda(\mathit{base})$ is defined as $\Lambda(\mathit{base}) = v$ and computable (as $\mathcal{E}$ is \emph{any} execution).
Thus, we reach a contradiction with the fact that $\Lambda(\mathit{base})$ is not defined or not computable, which concludes the proof.
\end{proof}

\subsection{Triviality of Solvable Validity Properties if $n \leq 3t$} \label{subsection:triviality_extended}

In this subsection, we prove that if a validity property is solvable with $n \leq 3t$, then the validity property is trivial.
We prove this result for the original formalism in \Cref{subsection:triviality_main}; in this subsection, we prove the result for the extended formalism.
Let us start by (re)defining trivial validity properties (for the extended formalism).

\begin{definition} [Trivial validity property] \label{definition:trivial_validity_extended}
A validity property $\mathit{val}$ is \emph{trivial} if and only if there exists a value $v' \in \mathcal{V}_O$ such that (1a) $v' \in \mathsf{discover}(\emptyset)$, or (1b) for every $v \in \mathcal{V}_I$, $v' \in \mathsf{discover}(\{v\})$, and (2) $v' \in \bigcap\limits_{c \in \mathcal{I}} \mathit{val}(c)$.
\end{definition}

Let us fix any solvable validity property $\mathit{val}$, and any Byzantine consensus algorithm $\mathcal{A}$ with $\mathit{val}$.
Recall that $n \leq 3t$.
In the main body of the paper, we have shown that there exists a value $v_{\mathit{base}} \in \bigcap\limits_{c \in \mathcal{I}} \mathit{val}(c)$.
This result holds even for the extended formalism as the approach presented in \Cref{subsection:triviality_main} can be reused.
Hence, it is left for us to show that, for every $v \in \mathcal{V}_I$, $v_{\mathit{base}} \in \mathsf{discover}(\{v\})$.
This holds due to \Cref{lemma:triviality_compatible}.

\begin{lemma} \label{lemma:triviality_extended}
For every $v \in \mathcal{V}_I$, $v_{\mathit{base}} \in \mathsf{discover}(\{v\})$.
\end{lemma}
\begin{proof}
Due to \Cref{lemma:triviality_compatible}, for every $v \in \mathcal{V}_I$, there exists a canonical execution $\mathcal{E} \in \mathit{execs}(\mathcal{A})$ such that (1) $v_{\mathit{base}}$ is decided in $\mathcal{E}$, and (2) all correct processes propose the same value $v$ in $\mathcal{E}$.
Therefore, by \Cref{assumption:extended}, $v_{\mathit{base}} \in \mathsf{discover}(\{v\})$.
\end{proof}

Therefore, $\mathit{val}$ is indeed a trivial validity property (according to \Cref{definition:trivial_validity_extended}), which concludes the subsection.

% \begin{theorem} [All solvable validity properties with $n \leq 3t$ are trivial]
% The validity property $\mathit{val}$ is trivial.
% \end{theorem}

\subsection{Similarity Condition: Sufficient Condition for Solvable Validity Properties if $n > 3t$} \label{subsection:sufficient_extended}

Finally, we show that the similarity condition is sufficient for solvable validity properties if $n > 3t$.
Namely, we show that \Cref{algorithm:general} solves any validity property (expressed using the external formalism) which satisfies $\mathcal{C}_S$.

\begin{theorem}
Let $\mathit{val}$ be any validity property which satisfies $\mathcal{C}_S$.
\general (\Cref{algorithm:general}) is a Byzantine consensus algorithm with $\mathit{val}$.
\end{theorem}
\begin{proof}
\emph{Termination} and \emph{Agreement} of \general follow from \emph{Termination} and \emph{Agreement} of \textsc{Icon}, respectively.
% Moreover, the message (resp., communication) complexity of \textsc{Complete} follows from the message (resp., communication) complexity of \textsc{Icon}.
Finally, we prove that \general satisfies $\mathit{val}$.
Consider any execution $\mathcal{E}$ of \general such that $\mathsf{corresponding}(\mathcal{E}) = c^*$, for some input configuration $c^* \in \mathcal{I}$.
Let $c \in \mathcal{I}_{n - t}$ be the input configuration correct processes decide from \textsc{Icon} in $\mathcal{E}$ (line~\ref{line:decide_ic}).
As \textsc{Icon} satisfies \emph{Vector Validity}, we have that, for every process $P \in \processes{c^*} \cap \processes{c}$, $P$'s proposals in $c^*$ and $c$ are identical.
Moreover, for every process $Q \in \processes{c} \setminus{\processes{c^*}}$, $Q's$ proposal according to $c$ belongs to $\mathsf{pool}(c^*)$.
Hence, $c \leftsquigarrow c^*$.
Therefore, $\Lambda(c) \in \mathit{val}(c^*)$ (by the definition of the $\Lambda$ function).
Thus, $\mathit{val}$ is satisfied by \general.
% , which concludes the proof.
\end{proof}
