# Supplementary material for: Partial Synchrony for Free? New Upper Bounds for Byzantine Agreement
Source: arXiv:2402.10059 source file (2024-10-23)
Supplement: Supplementary file 3 [file external.tex]

\section{Extended Formalism} \label{section:extended_formalim_appendix}

In this section, we give intuition behind an extension of our formalism which is suitable for the analysis of blockchain-specific validity properties, such as \emph{External Validity}~\cite{Cachin2001,BKM19,yin2019hotstuff}.
\emph{External Validity} stipulates that any decided value must satisfy a predetermined logical predicate.
However, the ``difficulty'' of this property is that the logical predicate (usually) verifies a cryptographic proof, which processes might not know a priori (see \Cref{subsection:intution_extended}).

In a nutshell, we make our original formalism more expressive by (1) making the input ($\mathcal{V}_I$) and output ($\mathcal{V}_O$) spaces ``unknown'' to the processes, and (2) taking into account ``proposals'' of faulty processes.
In the rest of the paper:
\begin{compactitem}
    \item We refer to the formalism introduced in the main body of the paper as the ``original formalism''.
    
    \item We refer to the formalism we introduce below as the ``extended formalism''.
\end{compactitem}
We start by giving an intuition behind our extended formalism (\Cref{subsection:intution_extended}).
Then, we introduce some preliminaries (\Cref{subsection:preliminaries_extended}).
Finally, we (incompletely) define our extended formalism (\Cref{subsection:validity_extended}).
% , and show how it can be used to define \emph{External Validity} (\Cref{subsection:validity_extended}).

% For the sake of completeness, we define the extended formalism from the ground up.
% We underline that the extended formalism is similar to the original one.
% In the rest of the paper, we show that the results presented in the main body of the paper hold for the extended formalism, as well.

\subsection{Intuition} \label{subsection:intution_extended}

In the original formalism, processes know the entire input space $\mathcal{V}_I$ and the entire output space $\mathcal{V}_O$.
That is, processes are able to ``produce'' any value which belongs to $\mathcal{V}_I$ or $\mathcal{V}_O$.
However, this assumption limits the expressiveness of our formalism as it is impossible to describe a Byzantine consensus problem in which input or output spaces are not a priori known.
Let us give an example.

Imagine a committee-based blockchain which establishes two roles:
\begin{compactitem}
    \item \emph{Clients} are the users of the blockchain.
    They issue \emph{signed} transactions to the blockchain.
    
    \item \emph{Servers} are the operating nodes of the blockchain.
    Servers receive signed transactions issued by the clients, and solve the Byzantine consensus problem to agree on the exact order the transactions are processed.
\end{compactitem}
As the servers propose transactions \emph{signed by the clients} and they do not have access to the private keys of the clients, the servers do not know the input space $\mathcal{V}_I$ nor the output space $\mathcal{V}_O$ of the Byzantine consensus problem.
Hence, our original formalism cannot describe the Byzantine consensus problem in the core of the aforementioned blockchain.

\paragraph{Extended vs. original formalism.}
As highlighted above, the main difference between the two formalisms is that the extended one allows us to specify the ``knowledge level'' of the input and output spaces.
In the extended formalism, a process is able to ``learn'' output values by observing input values.
That is, we define a \emph{discovery function} that defines which output values are learned given observed input values.
In the committee-based blockchain example, once a server observes signed (by the issuing clients) transactions $\mathit{tx}_1$ and $\mathit{tx}_2$, it learns the following output values: (1) $\mathit{tx}_1$, (2) $\mathit{tx}_2$, (3) $\mathit{tx}_1 || \mathit{tx}_2$, and (4) $\mathit{tx}_2 || \mathit{tx}_1$.\footnote{We denote by ``$||$'' the concatenation operation.} 

The second difference between the original and the extended formalism is that the extended formalism takes into account ``proposals'' of the faulty processes.
Indeed, the original formalism does not enable us to define which values are admissible given the adversary's knowledge of the input space.
Think of the aforementioned example with a blockchain system.
If no process (correct or faulty) obtains a transaction $\mathit{tx}$, $\mathit{tx}$ cannot be decided.
However, even if \emph{only} a faulty process obtains a transaction $\mathit{tx}$, $\mathit{tx}$ could still be an admissible decision.
This scenario can be described by the extended formalism, and not by the original one.

\subsection{Preliminaries} \label{subsection:preliminaries_extended}

We denote by $\mathcal{V}_I$ the input space of Byzantine consensus.
% , i.e., processes propose values contained in $\mathcal{V}_I$.
Similarly, $\mathcal{V}_O$ denotes the output space.
% , i.e., processes decide values which belong to $\mathcal{V}_O$.
% Recall that processes might not (fully) know $\mathcal{V}_I$ or $\mathcal{V}_O$.
% For the sake of simplicity, throughout the rest of the paper, we assume that $\mathcal{V}_I \cap \mathcal{V}_O = \emptyset$.\footnote{Observe that this is not a restring assumption as, for any value $v \in \mathcal{V}_I \cap \mathcal{V}_O$, we can (1) map $v$ into some value $v'$ such that $v' \notin \mathcal{V}_I$, and (2) ``swap'' $v$ with $v'$ in $\mathcal{V}_O$.}

\paragraph{Membership functions.}
We define two \emph{membership functions}:
\begin{compactitem}
    \item $\mathsf{valid\_input} : \{ 0, 1\}^* \to \{ \mathit{true}, \mathit{false} \}$: Intuitively, the $\mathsf{valid\_input}(\cdot)$ function specifies whether a bit-sequence belongs to the input space $\mathcal{V}_I$.
    
    \item $\mathsf{valid\_output} : \{ 0, 1 \}^* \to \{ \mathit{true}, \mathit{false} \}$: Intuitively, the $\mathsf{valid\_output}(\cdot)$ function specifies whether a bit-sequence belongs to the output space $\mathcal{V}_O$.
\end{compactitem}
We assume that each process has access to these two functions.
That is, each process can verify whether an arbitrary sequence of bits belongs to the input ($\mathcal{V}_I$) or output ($\mathcal{V}_O$) space.
In the case of a committee-based blockchain (\Cref{subsection:intution_extended}), the membership functions are signature-verification functions.

% We assume that these two functions behave as an oracle: any process is able to query the oracle (via the aforementioned two function), and it eventually receives an (honest) answer.

\paragraph{Discovery function.}
We define a function $\mathsf{discover}$: $2^{\mathcal{V}_I} \to 2^{\mathcal{V}_O}$.
Given a set of proposals $V_I \subseteq \mathcal{V}_I$, $\mathsf{discover}(V_I) \subseteq \mathcal{V}_O$ specifies the set of decisions which are ``discoverable'' by $V_I$.
% Moreover, for every value $v \in \mathcal{V}_I \cap \mathcal{V}_O$, $\{v\} \subseteq \mathsf{discover}(v)$.
We assume that each process has access to the $\mathsf{discover}(\cdot)$ function.
% , and the function behaves as an oracle.
Moreover, for any two sets $V_I^1, V_I^2$ with $V_I^1 \subseteq V_I^2$, $\mathsf{discover}(V_I^1) \subseteq \mathsf{discover}(V_I^2)$; in other words, ``knowledge'' of the output space can only be improved upon learning more input values.

Let us take a look at the committee-based blockchain example again (\Cref{subsection:intution_extended}).
If a server obtains a proposal $\mathit{tx}$, it learns $\mathit{tx}$ as a potential decision.
We model this ``deduction'' concept using the $\mathsf{discover}(\cdot)$ function: $\mathsf{discover}\big( \{\mathit{tx}\} \big) = \{\mathit{tx}\}$.

% \paragraph{Executions.}
% Given an algorithm $\mathcal{A}$, $\mathit{execs}(\mathcal{A})$ denotes the set of all executions of $\mathcal{A}$.
% Furthermore, $\mathit{Corr}_{\mathcal{A}}(\mathcal{E})$ denotes the set of correct processes in $\mathcal{E} \in \mathit{execs}(\mathcal{A})$.
% Lastly, an execution $\mathcal{E} \in \mathit{execs}(\mathcal{A})$ is \emph{canonical} if and only if no faulty process takes any computational step in $\mathcal{E}$; note that faulty processes do not send any message in a canonical execution.

\paragraph{Adversary pool.}
Given an execution $\mathcal{E}$, $\mathcal{P}(\mathcal{E}) \subseteq \mathcal{V}_I$ defines the \emph{adversary pool} in $\mathcal{E}$.
Informally, the adversary pool represents the input values the adversary ``knows''.
% In the case of an algorithm which supports the $\mathsf{propose}(\cdot)$ request, we assume that the adversary pool contains the proposals of correct processes.
% That is, the adversary knows the proposals of correct processes (and, potentially, something more).
In the example of a committee-based blockchain (\Cref{subsection:intution_extended}), the adversary pool is a set of signed transactions which the adversary ``learns'' from the clients.

We underline that the adversary pool is an abstract concept.
Specifically, the adversary pool represents the ``starting knowledge'' the adversary has.
However, the notion of the ``starting knowledge'' must be precisely defined once all particularities of the exact considered system are taken into account.
Due to sophisticated details (such as the aforementioned one), we believe that a formalism suitable for blockchain-specific validity properties deserves its own standalone paper.

\subsection{Validity} \label{subsection:validity_extended}

We start by restating the definition of process-proposal pairs.
% (The definition remains identical to the one introduced in the original formalism.)
A \emph{process-proposal} pair is a pair $(P, v)$, where (1) $P \in \allprocesses$ is a process, and (2) $v \in \mathcal{V}_I$ is a proposal.
Given a process-proposal pair $\mathit{pp} = (P, v)$, $\mathsf{proposal}(\mathit{pp}) = v$ denotes the proposal associated with $\mathit{pp}$.

An \emph{input configuration} is a tuple $\big[ \mathit{pp}_1, \mathit{pp}_2, ..., \mathit{pp}_x, \rho \big]$ of $x$ process-proposal pairs and a set $\rho \subseteq \mathcal{V}_I$, where (1) $n - t \leq x \leq n$, (2) every process-proposal pair is associated with a distinct process, and (3) if $x = n$, $\rho = \emptyset$.
% , and (4) if there exists a process-proposal pair $(\cdot, v)$.
% $ in the tuple and $x \neq n$, then $v \in \rho$.
Intuitively, an input configuration represents an assignment of proposals to correct processes, as well as a ``part'' of the input space known to the adversary.
% ; we assume that the adversary knows the input values which are known to the correct processes.
For example, an input configuration $\big[ (P_1, v), (P_2, v), (P_3, v), \{v, v', v''\} \big]$ describes an execution in which (1) only processes $P_1$, $P_2$, and $P_3$ are correct, (2) processes $P_1$, $P_2$, and $P_3$ propose the same value $v$, and (3) faulty processes know only $v$, $v'$, and $v''$.
% $\{v''\}$.

We denote by $\mathcal{I}$ the set of all input configurations.
% Furthermore, for every $x \in [n - t, n]$, $\mathcal{I}_x \subset \mathcal{I}$ denotes the set of input configurations with \emph{exactly} $x$ process-proposal pairs.
For every input configuration $c \in \mathcal{I}$, we denote by $c[i]$ the process-proposal pair associated with process $P_i$; if such a process-proposal pair does not exist, $c[i] = \bot$.
Moreover, we define by $\mathsf{pool}(c)$ the set of input values associated with $c$ (the ``$\rho$'' field of $c$).
Next, $\process{c} = \{ P_i \in \Pi \,|\, c[i] \neq \bot\}$ denotes the set of all processes included in $c$.
Finally, $\mathsf{correct\_proposals}(c) = \{ v \in \mathcal{V}_I \,|\, \exists i \in [1, n]: c[i] \neq \bot \land \mathsf{proposal}(c[i]) = v \}$ denotes the set of all proposals of correct processes (as specified by $c$).

Given (1) an execution $\mathcal{E} \in \mathit{execs}(\mathcal{A})$, where $\mathcal{A}$ is an algorithm with the $\mathsf{propose}(\cdot)/\mathsf{decide}(\cdot)$ interface, and (2) an input configuration $c \in \mathcal{I}$, we say that $\mathcal{E}$ \emph{corresponds} to $c$ ($\mathsf{input\_conf}(\mathcal{E}) = c$) if and only if (1) $\process{c} = \mathit{Corr}_{\mathcal{A}}(\mathcal{E})$, (2) for every process $P_i \in \mathit{Corr}_{\mathcal{A}}(\mathcal{E})$, $P_i$'s proposal in $\mathcal{E}$ is $\mathsf{proposal}(c[i])$, and (3) $\mathcal{P}(\mathcal{E}) = \mathsf{pool}(c)$.
% faulty processes know $\mathsf{pool}(c)$ at the beginning of $\mathcal{E}$.
% We denote by $\mathsf{input\_conf}(\mathcal{E}) = c$ the input configuration to which $\mathcal{E}$ corresponds.

A validity property $\mathit{val}$ is a function $\mathit{val}: \allconfigurations \to 2^{\mathcal{V}_O}$ such that, for every input configuration $c \in \allconfigurations$, $\mathit{val}(\mathit{c}) \neq \emptyset$.
Algorithm $\mathcal{A}$, where $\mathcal{A}$ exposes the $\mathsf{propose}(\cdot)/\mathsf{decide}(\cdot)$ interface, \emph{satisfies} a validity property $\mathit{val}$ if and only if, in every execution $\mathcal{E} \in \mathit{execs}(\mathcal{A})$, no correct process decides a value $v' \notin \mathit{val}\big( \mathsf{input\_conf}(\mathcal{E}) \big)$.
That is, an algorithm satisfies a validity property if and only if correct processes decide only admissible values.

% \paragraph{Consensus algorithms.}
% An algorithm $\mathcal{A}$ solves the consensus problem with a validity property $\mathit{val}$ if and only if:
% \begin{compactitem}
%     \item $\mathcal{A}$ exposes the $\mathsf{propose}(\cdot)/\mathsf{decide}(\cdot)$ interface, and
    
%     % \item $\mathcal{A}$ tolerates up to $t$ Byzantine failures, and
    
%     \item $\mathcal{A}$ satisfies \emph{Termination}, \emph{Agreement} and the validity property $\mathit{val}$.
% \end{compactitem}

\paragraph{Assumptions on executions.}
Lastly, we introduce two assumptions that conclude our proposal for the extended formalism.

\begin{assumption} \label{assumption:all_executions}
For every execution $\mathcal{E}$ of any algorithm $\mathcal{A}$ which solves the Byzantine consensus problem with some validity property, if a correct process $P$ decides a value $v' \in \mathcal{V}_O$ in $\mathcal{E}$, then $v' \in \mathsf{discover}\big( \mathsf{correct\_proposals}(c) \cup \mathsf{pool}(c) \big)$, where $\mathsf{input\_conf}(\mathcal{E}) = c$.
\end{assumption}

\Cref{assumption:all_executions} states that correct processes can only decide values which are ``discoverable'' using all the proposals of correct processes and the knowledge of the adversary.
For example, if every correct process proposes the same value $v \in \mathcal{V}_I$ and the adversary pool contains only $v' \in \mathcal{V}_I$, then a correct process can only decide a value from $\mathsf{discover}(\{v, v'\})$.

Next, we introduce an assumption concerned only with the canonical executions (executions in which faulty processes do not take any computational step).

\begin{assumption} \label{assumption:extended}
For every canonical execution $\mathcal{E}$ of any algorithm $\mathcal{A}$ which solves the Byzantine consensus problem with some validity property, if a correct process $P$ decides a value $v' \in \mathcal{V}_O$ in $\mathcal{E}$, then $v' \in \mathsf{discover}\big( \mathsf{correct\_proposals}(c) \big)$, where $\mathsf{input\_conf}(\mathcal{E}) = c$.
\end{assumption}

Intuitively, \Cref{assumption:extended} states that, if faulty processes are silent, correct processes can only decide values which can be discovered using their own proposals.
In other words, correct processes cannot use ``hidden'' proposals (possessed by the silent adversary) to discover a decision.

Finally, we underline that these two assumptions do not completely prevent ``unreasonable'' executions.
For example, given these two assumptions, a (correct or faulty) process is still able to send a message with a value which cannot be discovered using the proposals of correct processes and the adversary pool.
Hence, an assumption that prevents such an execution should be introduced.
Thus, due to the complexity of the extended formalism, we leave it out of this paper.
In the future, we will focus on this interesting and important problem.
