# Supplementary material for: Partial Synchrony for Free? New Upper Bounds for Byzantine Agreement
Source: arXiv:2402.10059 source file (2024-10-23)
Supplement: Supplementary file 4 [file external_validity_sync.tex]

\section{Synchronous Byzantine Agreement with $O(\log(n)L + n\log(n))$ Bits Per-Process} \label{section:external_validity_sync_consensus}

In this section, we design a synchronous Byzantine agreement algorithm \sync that (1) satisfies both strong and external validity, (2) tolerates up to $t < n / 3$ faulty processes, (3) requires no cryptography or trusted setup, and (4) where each correct process sends at most $O(L\log n + n\log n)$ bits.
We use this synchronous algorithm in \name to obtain a few partially synchronous algorithms (see \Cref{subsection:concrete_algorithms}).
To construct \sync, we employ the structure proposed by Momose and Ren~\cite{Momose2021} that recursively constructs Byzantine agreement using synchronous graded consensus.

\subsection{Synchronous Graded Consensus with External Validity}

This subsection shows how graded consensus with external validity (see \Cref{subsection:graded_consensus_building_blocks}) can be solved in synchrony such that its per-process bit complexity is $O(L + n\log n)$.
Our solution (\Cref{algorithm:synchronous_graded_consensus_external_validity}) (1) tolerates up to $t < n / 3$ faulty processes, (2) uses no cryptography, and (3) employs \textsc{COOL}~\cite{chen2021optimal}, a cryptography-free synchronous Byzantine agreement protocol with \emph{only} strong validity that achieves $O(L + n\log n)$ per-process bit complexity.

\begin{algorithm}
\caption{Synchronous Graded Consensus with External Validity: Pseudocode (for process $p_i$)}
\label{algorithm:synchronous_graded_consensus_external_validity}
\footnotesize
\begin{algorithmic} [1] 
\State \textbf{Uses:}
\State \hskip2em \textsc{COOL}~\cite{chen2021optimal}, \textbf{instance} $\mathcal{BA}$

\medskip
\State \textbf{Local variables:}
\State \hskip2em $\mathsf{Value}$ $\mathit{pro}_i \gets \bot$

\medskip
\State \textbf{upon} $\mathsf{propose}(v \in \mathsf{Value})$:
\State \hskip2em $\mathit{pro}_i \gets v$
\State \hskip2em \textbf{invoke} $\mathcal{BA}.\mathsf{propose}(v)$

\medskip
\State \textbf{upon} $\mathcal{BA}.\mathsf{decide}(v' \in \mathsf{Value})$: \label{line:gce_decide_from_ba}
\State \hskip2em \textbf{if} $\mathsf{valid}(v') = \mathit{true}$: \label{line:gce_check_decide_grade_1}
\State \hskip4em \textbf{trigger} $\mathsf{decide}(v', 1)$ \label{line:gce_decide_grade_1}
\State \hskip2em \textbf{else:}
\State \hskip4em \textbf{trigger} $\mathsf{decide}(\mathit{pro}_i, 0)$ \label{line:gce_decide_grade_2}
\end{algorithmic} 
\end{algorithm}

\paragraph{Proof of correctness.}
We now prove that \Cref{algorithm:synchronous_graded_consensus_external_validity} is correct.

\begin{theorem} [Correctness]
\Cref{algorithm:synchronous_graded_consensus_external_validity} is correct.
\end{theorem}
\begin{proof}
Integrity and termination hold trivially.
Consistency holds as, if a correct process decides a pair $(v' \in \mathsf{Value}, 1)$ (line~\ref{line:gce_decide_grade_1}), then every correct process decides $(v', 1)$ (line~\ref{line:gce_decide_grade_1}) due to the agreement property of \textsc{COOL}.
External validity holds as (1) correct processes only decide valid values at line~\ref{line:gce_decide_grade_1} (due to the check at line~\ref{line:gce_check_decide_grade_1}), and (2) correct processes only decide valid values at line~\ref{line:gce_decide_grade_2} as no correct process proposes an invalid value.

Finally, suppose that all correct processes propose the same value $v$.
Note that, as no correct process proposes an invalid value, as $v$ is a valid value.
Due to the strong validity property of \textsc{COOL}, every correct process eventually decides $v$ from it (line~\ref{line:gce_decide_from_ba}).
As $v$ is a valid value, the check at line~\ref{line:gce_check_decide_grade_1} passes, which implies that every correct process decides $(v, 1)$.
\end{proof}

\paragraph{Proof of complexity.}
We now prove the complexity of \Cref{algorithm:synchronous_graded_consensus_external_validity}.

\begin{theorem} [Complexity]
Every correct process sends $O(L + n\log n)$ bits in \Cref{algorithm:synchronous_graded_consensus_external_validity}.
\end{theorem}
\begin{proof}
This follows directly from the fact that every correct process sends at most $O(L + n\log n)$ bits in \textsc{COOL}.
\end{proof}

\subsection{\sync: Synchronous Byzantine Agreement with $O(L \log n + n \log n)$ Bits Per-Process}

Before presenting \sync, we introduce our \textsc{expander} primitive.

\paragraph{\textsc{expander} primitive.}
Consider a system $\mathcal{S}$ of $n$ processes, and a subsystem $\mathcal{S}' \subset \mathcal{S}$ of $n' = n / 2$ processes, such that
at most $t' < n' / 3 = n / 6$ faulty processes belong to $\mathcal{S}'$.
The \textsc{expander} primitive guarantees the following:
Let $M$ be a value that is the input of every correct process that belongs to $\mathcal{S}'$.
% The remaining correct processes that belong to $\mathcal{S}'$ input $\bot$.
After 2 synchronous rounds, every correct process that belongs to $\mathcal{S}$ outputs $M$.
The \textsc{expander} primitive is heavily inspired by the ADD primitive introduced in~\cite{das2021asynchronous}.

\begin{algorithm}
\caption{\textsc{expander}: Pseudocode (for process $p_i$)}
\label{algorithm:expander}
\footnotesize
\begin{algorithmic} [1]
\State Let $p_i \in \mathcal{S}$. If $p_i \in \mathcal{S}'$, let $M_i$ be the \textbf{input} of $p_i$ ($M_i = M$).

\medskip
\State \textbf{Round 1:} \BlueComment{execute only if $p_i \in \mathcal{S}'$}
% \State \hskip2em \textbf{if} $M_i \neq \bot$:
\State \hskip2em Let $[m_1, m_2, ..., m_{n'}] \gets \mathsf{RSEnc}(M_i, n', t' + 1)$
\State \hskip2em \textbf{broadcast} $\langle \textsc{reconstruct}, m_i \rangle$ to every process $p_j \in \mathcal{S}$
% \State \hskip2em Let $m_i^* \gets m_i$

% \medskip
% \State \textbf{Round 2:} \BlueComment{execute only if $p_i \in \mathcal{S}'$}
% \State \hskip2em \textbf{if} $M_i = \bot$:
% \State \hskip4em Let $m_i^* \gets $ an RS symbol received at least $t' + 1$ times in \textsc{disperse} messages
% \State \hskip2em \textbf{broadcast} $\langle \textsc{reconstruct}, m_i^* \rangle$ to every process in $\mathcal{S}$

\medskip
\State \textbf{Round 2:} \BlueComment{execute always (i.e., if $p_i \in \mathcal{S}$)}
\State \hskip2em Let $x$ denote the number of received \textsc{reconstruct} messages
\State \hskip2em \textbf{if} $x \geq n' - t'$:
\State \hskip4em \textbf{output} $\mathsf{RSDec}(t' + 1, x - (n' - t'), \text{received RS symbols})$
\end{algorithmic} 
\end{algorithm}

We now prove the correctness of \textsc{expander} (\Cref{algorithm:expander}).

\begin{theorem} [Correctness]
\textsc{expander} is correct.
\end{theorem}
\begin{proof}
% Consider any correct process $p_i \in \mathcal{S}'$.
% Eventually, $p_i$ sets $m_i^*$ to a correctly-encoded RS symbol as all correct processes from $\mathcal{S}'$ with non-$\bot$ input have the same input $M$.
Every correct process from $\mathcal{S}'$ eventually sends a \textsc{reconstruct} message with a correctly-encoded RS symbol of $M$.
Hence, every correct process from $\mathcal{S}$ eventually receives at least $n' - t'$ correctly-encoded RS symbols, and successfully reconstructs $M$.
\end{proof}

Next, we prove the per-process cost of \textsc{expander}.

\begin{theorem} [Complexity]
Every correct process $p_i \in \mathcal{S}'$ sends $O(L + n\log n)$ bits.
Moreover, every correct process $p_j \in \mathcal{S} \setminus{\mathcal{S}'}$ sends $0$ bits.
\end{theorem}
\begin{proof}
Each correct process $p_j \in \mathcal{S} \setminus{\mathcal{S}'}$ indeed sends 0 bits.
Moreover, every correct process $p_i \in \mathcal{S}'$ broadcasts an RS symbol once.
Therefore, $p_i$ sends $n \cdot O(\frac{L}{n / 2} + \log(n / 2)) = n \cdot O(L / n + \log(n)) = O(L + n\log n)$ bits.
\end{proof}

\paragraph{\sync's description.}
As previously mentioned, \sync follows the structure proposed by Momose and Ren~\cite{momose2021multi}.
Namely, \sync partitions all $n$ processes into two halves, where each half runs \sync (among $n / 2$ processes).
The partition continues until an instance of \sync with only a single process is reached.
When such an instance is reached, the single operating process decides its proposal.
For completeness, we present this construction below.
We denote by $\mathcal{S} = \{p_1, p_2, ..., p_n\}$ the entire system of the processes.
Moreover, $\mathcal{S}_1 = \{p_1, p_2, ..., p_{n / 2}\}$ denotes the first half of the processes, whereas $\mathcal{S}_2 = \{p_{n / 2 + 1}, ..., p_n\}$ denotes the second half of the processes. 

\smallskip
\begin{mdframed} [frametitle={\sync among $n$ processes}, frametitlealignment=\centering]
Let $p_i$ be a process, and let $v_i$ be $p_i$'s variable which is initialized to $p_i$'s proposal.

\smallskip
\noindent If $n = 1$, $p_i$ decides $v_i$ (i.e., $p_i$'s proposal).
Otherwise, $p_i$ executes the following steps and outputs $v_i$.

\noindent (1) Run the first graded consensus algorithm $\mathcal{GC}_1(\mathcal{S})$ among $\mathcal{S}$ with proposal $v_i$.
Let $(\mathit{val}_1, g_1)$ be the pair decided from $\mathcal{GC}_1(\mathcal{S})$.
Set $v_i$ to $\mathit{val}_1$.

\noindent (2) If $p_i \in \mathcal{S}_{1}$, run \sync among $\mathcal{S}_1$ with input $v_i$, and input the decision of the algorithm to \textsc{expander} for $\mathcal{S}$ and $\mathcal{S}_1$.
Otherwise, wait for the step to finish.

\noindent (3) If $p_i$ outputs a valid value $v$  from \textsc{expander} and $g_1 = 0$, set $v_i$ to $v$.

\noindent (4) Run the second graded consensus algorithm $\mathcal{GC}_2(\mathcal{S})$ among $\mathcal{S}$ with proposal $v_i$.
Let $(\mathit{val}_2, g_2)$ be the pair decided from $\mathcal{GC}_2(\mathcal{S})$.
Set $v_i$ to $\mathit{val}_2$.

\noindent (5) If $p_i \in \mathcal{S}_{2}$, run \sync among $\mathcal{S}_2$ with input $v_i$, and input the decision of the algorithm to \textsc{expander} for $\mathcal{S}$ and $\mathcal{S}_2$.
Otherwise, wait for the step to finish.

\noindent (6) If $p_i$ outputs a valid value $v$  from \textsc{expander} and $g_2 = 0$, set $v_i$ to $v$.
\end{mdframed}

\paragraph{Proof of correctness.}
To prove the correctness, we start by proving termination.

\begin{theorem} [Termination]
\sync satisfies termination.
\end{theorem}
\begin{proof}
Termination holds as every step eventually finishes.
\end{proof}

% Next, we prove integrity.

% \begin{theorem} [Integrity]
% \sync satisfies integrity.
% \end{theorem}
% \begin{proof}
% Integrity holds as every correct process decides at most once.
% \end{proof}
% \ayaz{we don't have integrity property in byzantine agreement}

Next, we prove strong validity.
\begin{theorem} [Strong validity]
\sync satisfies strong validity.
\end{theorem}
\begin{proof}
Suppose that all correct processes propose the same value $v$.
Hence, all correct processes decide $(v, 1)$ from $\mathcal{GC}_1(\mathcal{S})$ (Step 1).
Therefore, all correct processes propose $v$ to $\mathcal{GC}_2(\mathcal{S})$ and decide $(v, 1)$ from $\mathcal{GC}_2(\mathcal{S})$ (Step 4).
Thus, every correct process decides $v$.
\end{proof}

Next, we prove external validity.

\begin{theorem} [External validity]
\sync satisfies external validity.
\end{theorem}
\begin{proof}
The theorem holds as any correct process $p_i$ updates its $v_i$ variable only to valid values.
\end{proof}

Finally, we prove agreement.

\begin{theorem} [Agreement]
\sync satisfies agreement.
\end{theorem}
\begin{proof}
Importantly, $\mathcal{S}_1$ or $\mathcal{S}_2$ contain less than one-third of faulty processes.
Hence, one of these two halves is ``correct'', in the sense that it contains less than one-third faulty processes.
We consider two possibilities:
\begin{compactitem}
    \item Let $\mathcal{S}_1$ be correct.
    In this case, all correct processes propose the same value to $\mathcal{GC}_2(\mathcal{S})$. To show this,
    let us study two possibilities:
    \begin{compactitem}
        \item There exists a correct process that decides $(v, 1)$ from $\mathcal{GC}_1(\mathcal{S})$.
        In this case, every correct process that decides from $\mathcal{GC}_1(\mathcal{S})$ with grade $1$ must decide $v$ (due to the consistency property of $\mathcal{GC}_1(\mathcal{S})$).
        Moreover, all correct processes propose $v$ to \sync among $\mathcal{S}_1$ (due to the consistency property of $\mathcal{GC}_1(\mathcal{S})$).
        As $\mathcal{S}_1$ is a correct half and \sync satisfies strong and external validity, every correct process in $\mathcal{S}_1$ decides the valid value $v$.
        Hence, every correct member of $\mathcal{S}_1$ inputs the valid value $v$ to \textsc{expander} and the precondition of \textsc{expander} is satisfied (as $\mathcal{S}_1$ is a correct half).
        Therefore, every correct process from $\mathcal{S}$ outputs $v$ from \textsc{expander}, and proposes $v$ to $\mathcal{GC}_2(\mathcal{S})$.

        \item No correct process decides with grade $1$ from $\mathcal{GC}_1(\mathcal{S})$.
        In this case, as $\mathcal{S}_1$ is a correct half and \sync satisfies agreement and external validity, all correct processes in $\mathcal{S}_1$ decide the same valid value $v$ from \sync among $\mathcal{S}_1$.
        Hence, every correct member of $\mathcal{S}_1$ inputs the same valid value $v$ to \textsc{expander} and the precondition of \textsc{expander} is satisfied (as $\mathcal{S}_1$ is a correct half).
        Therefore, every correct process from $\mathcal{S}$ outputs $v$ from \textsc{expander}, and proposes $v$ to $\mathcal{GC}_2(\mathcal{S})$.
    \end{compactitem}
    Therefore, all correct processes will decide $(v, 1)$ from $\mathcal{GC}_2(\mathcal{S})$ (due to the strong validity property), for some value $v$, which concludes the proof.

    \item Let $\mathcal{S}_2$ be correct. 
    Note that any value output by $\mathcal{GC}_2(\mathcal{S})$ is necessarily valid due to the external validity property and the fact that all correct processes only input valid values to $\mathcal{GC}_2(\mathcal{S})$.
    Let us study two possibilities:
    \begin{compactitem}
        \item There exists a correct process that decides $(v, 1)$ from $\mathcal{GC}_2(\mathcal{S})$.
        In this case, every correct process that decides from $\mathcal{GC}_2(\mathcal{S})$ with grade $1$ must decide $v$ (due to the consistency property of $\mathcal{GC}_2(\mathcal{S})$).
        Moreover, all correct processes propose $v$ to \sync among $\mathcal{S}_2$ (due to the consistency property of $\mathcal{GC}_2(\mathcal{S})$).
        As $\mathcal{S}_2$ is a correct half and \sync satisfies strong and external validity, every correct process in $\mathcal{S}_2$ decides the valid value $v$.
        Hence, every correct member of $\mathcal{S}_2$ inputs the valid value $v$ to \textsc{expander} and the precondition of \textsc{expander} is satisfied (as $\mathcal{S}_2$ is a correct half).
        Therefore, every correct process $p_i$ from $\mathcal{S}$ outputs $v$ from \textsc{expander}, and has $v_i = v$ at the end of step 6.

        \item No correct process decides with grade $1$ from $\mathcal{GC}_2(\mathcal{S})$.
        In this case, as $\mathcal{S}_2$ is a correct half and \sync satisfies agreement and external validity, all correct processes in $\mathcal{S}_2$ decide the same valid value $v$ from \sync among $\mathcal{S}_2$.
        Hence, every correct member of $\mathcal{S}_2$ inputs the valid value $v$ to \textsc{expander} and the precondition of \textsc{expander} is satisfied (as $\mathcal{S}_2$ is a correct half).
        Therefore, every correct process $p_i$ from $\mathcal{S}$ outputs $v$ from \textsc{expander}, and has $v_i = v$ at the end of step 6.
    \end{compactitem}
    Therefore, all correct processes decide the same value even in this case.
\end{compactitem}
Thus, the agreement property is satisfied.
\end{proof}

\paragraph{Proof of complexity.}
Finally, we prove that every process sends $O(L\log(n) + n\log n)$ bits.

\begin{theorem} [Complexity]
Every correct process sends $O(L\log n + n \log n)$ bits.
\end{theorem}
\begin{proof}
Consider any correct process $p_i$.
The number of bits $b_i(n)$ process $p_i$ sends while executing \sync among $n$ processes can be expressed by the following recurrence:
\begin{equation*}
    b_i(n) = 2 \cdot O(L + n\log n) + O(L + n\log n) + b_i(n / 2) = O(L \log n + n\log n).
\end{equation*}
\end{proof}

% \ayaz{I tried leaving some comments using the review feature}
