# Supplementary material for: Partial Synchrony for Free? New Upper Bounds for Byzantine Agreement
Source: arXiv:2402.10059 source file (2024-10-23)
Supplement: Supplementary file 5 [file general_algorithm.tex]

\section{Vector Consensus: Formal Proofs \& Omitted Algorithms} \label{section:algorithm_appendix}

In \Cref{subsection:authenticated_vector_proof}, we prove the correctness and complexity of our authenticated implementation of vector consensus (\Cref{algorithm:interactive_consistency}).
We dedicate \Cref{subsection:nonauthenticated_vector} to a non-authenticated implementation of vector consensus.
Finally, in \Cref{subsection:better_communication}, we give an implementation of vector consensus with $O(n^2 \log n)$ communication complexity.
Throughout the entire section, we assume that $n > 3t$.

% In this section, we prove the correctness and complexity of our authenticated implementation of vector consensus (\Cref{algorithm:interactive_consistency}).
% Moreover, we give another implementation (\Cref{algorithm:non_authenticated}) of vector consensus; this implementation does not rely on authentication (i.e., on digital signatures).
% Recall that \general (\Cref{algorithm:general}) is amenable to the actual implementation of vector consensus.
% Therefore, by utilizing a non-authenticated implementation of vector consensus in \general, one can obtain a non-authenticated general Byzantine consensus algorithm.
% This implies that solvability of validity properties is \emph{independent} of the existence of cryptographic primitives.

\subsection{Authenticated Implementation (\Cref{algorithm:interactive_consistency}): Formal Proofs} \label{subsection:authenticated_vector_proof}

We start this subsection with some clarifications about \textsc{Quad}~\cite{civit2022byzantine}, a Byzantine consensus algorithm utilized in \Cref{algorithm:interactive_consistency}.
Then, we prove the correctness and complexity of \Cref{algorithm:interactive_consistency}.

\paragraph{A note on \textsc{Quad}.}
In \Cref{subsubsection:interactive_consistency}, we claim that \textsc{Quad} satisfies the following validity property: if a correct process decides a pair $(v, \Sigma)$, then $\mathsf{verify}(v, \Sigma) = \mathit{true}$.
Technically speaking, the authors of \textsc{Quad} only consider \emph{Weak Validity}, i.e., they do not claim that the their protocol satisfies the aforementioned validity property.
However, modifying their protocol to accommodate for the aforementioned property is trivial: each correct process simply discards each message which contains a pair $(v, \Sigma)$ for which $\mathsf{verify}(v, \Sigma) = \mathit{false}$.

Another subtle remark is that the authors of \textsc{Quad} prove its message and latency complexity assuming that all correct processes start executing \textsc{Quad} by GST.
In \Cref{algorithm:interactive_consistency}, this might not be the case: correct processes might receive $n - t$ \textsc{proposal} messages at $\text{GST} + \delta$ (line~\ref{line:received_n_t_proposals}), and thus start executing \textsc{Quad} at $\text{GST} + \delta$  (line~\ref{line:propose_quad}).
Nevertheless, it is easy to show that \textsc{Quad} ensures the stated complexity even if all correct processes start executing the algorithm by time $\text{GST} + O(\delta)$.
Not only that, even if correct processes do not start executing \textsc{Quad} within constant time after GST, but they all start executing the algorithm within $O(\delta)$ time within each other (after GST), the message complexity remains quadratic and the latency remains linear (measured from the time the first correct process starts executing \textsc{Quad}).

\paragraph{Correctness \& complexity of \Cref{algorithm:interactive_consistency}.}

The following theorem proves the correctness.

\begin{theorem}
\Cref{algorithm:interactive_consistency} is correct.
\end{theorem}
\begin{proof}
\emph{Agreement} follows directly from the fact that \textsc{Quad} satisfies \emph{Agreement}.
\emph{Termination} follows from (1) \emph{Termination} of \textsc{Quad}, and (2) the fact that, eventually, all correct processes receive $n - t$ \textsc{proposal} messages (as there are at least $n - t$ correct processes; line~\ref{line:received_n_t_proposals}).

We now prove that \Cref{algorithm:interactive_consistency} satisfies \emph{Vector Validity}.
Let a correct process $P$ decide $\mathit{vector}' \in \mathcal{I}_{n - t}$ from vector consensus (line~\ref{line:decide}).
Hence, $P$ has decided $(\mathit{vector}', \Sigma')$ from \textsc{Quad}, where (1) $\Sigma'$ is some proof, and (2) $\mathsf{verify}(\mathit{vector}', \Sigma') = \mathit{true}$ (due to the specification of \textsc{Quad}).
Furthermore, if there exists a process-proposal pair $(P, v \in \mathcal{V}_I)$ in $\mathit{vector}'$, where $P$ is a correct process, a properly signed \textsc{proposal} message belongs to $\Sigma'$.
As correct processes send \textsc{proposal} messages only for their proposals (line~\ref{line:broadcast_proposal}), $v$ was indeed proposed by $P$.
Thus, the theorem.
\end{proof}

Finally, we prove the complexity.

\begin{theorem}
The message complexity of \Cref{algorithm:interactive_consistency} is $O(n^2)$.
% , whereas its communication complexity is $O(n^3)$.
\end{theorem}
\begin{proof}
The message complexity of the specific instance of \textsc{Quad} utilized in \Cref{algorithm:interactive_consistency} is $O(n^2)$.
% message complexity, and $O(n^3)$ communication complexity (as proofs are of size $O(n)$).
Additionally, correct processes exchange $O(n^2)$ \textsc{proposal} messages.
% , each with a single signature.
Thus, the message complexity is $O(n^2) + O(n^2) = O(n^2)$.
% Its communication complexity is $O(n^3)$.
% Thus, the theorem.
\end{proof}

\subsection{Non-Authenticated Implementation: Pseudocode \& Formal Proofs} \label{subsection:nonauthenticated_vector}

We now present a non-authenticated implementation (\Cref{algorithm:non_authenticated}) of vector consensus.
% , a non-authenticated implementation of the Byzantine consensus problem with \emph{Vector Validity}.
The design of \Cref{algorithm:non_authenticated} follows the reduction from binary consensus to multivalued consensus (e.g.,~\cite{CGL18}).
Namely, we use the following two building blocks in \Cref{algorithm:non_authenticated}:
\begin{compactenum}
    \item Byzantine Reliable Broadcast~\cite{cachin2011introduction, B87}:
    This primitive allows processes to disseminate information in a reliable manner.
    Formally, Byzantine reliable broadcast exposes the following interface: (1) \textbf{request} $\mathsf{broadcast}(m)$, and (2) \textbf{indication} $\mathsf{deliver}(m')$.
    The primitive satisfies the following properties:
    \begin{compactitem}
        \item \emph{Validity:} If a correct process $P$ broadcasts a message $m$, $P$ eventually delivers $m$.
        
        \item \emph{Consistency:} No two correct processes deliver different messages.
        
        \item \emph{Integrity:} Every correct process delivers at most one message.
        Moreover, if a correct process delivers a message $m$ from a process $P$ and $P$ is correct, then $P$ broadcast $m$.
        
        \item \emph{Totality:} If a correct process delivers a message, every correct process delivers a message.
    \end{compactitem}
    In \Cref{algorithm:non_authenticated}, we use a non-authenticated implementation~\cite{B87} of the Byzantine reliable broadcast primitive.
    
    \item Binary DBFT~\cite{CGL18}, a non-authenticated algorithm which solves the Byzantine consensus problem with $\emph{Strong Validity}$.
\end{compactenum}
% We assume that $n > 3t$.

Let us briefly explain how \Cref{algorithm:non_authenticated} works; we focus on a correct process $P_i$.
First, $P_i$ reliably broadcasts its proposal (line~\ref{line:broadcast_proposal_nowic}).
Once $P_i$ delivers a proposal of some process $P_j$ (line~\ref{line:receive_proposal_nowic}), $P_i$ proposes $1$ to the corresponding DBFT instance (line~\ref{line:propose_dbft_nowic}).
Eventually, $n - t$ DBFT instances decide $1$ (line~\ref{line:dbft_decided_nowic}).
Once that happens, $P_i$ proposes $0$ to all DBFT instances to which $P_i$ has not proposed (line~\ref{line:propose_0_dbft_nowic}).
When all DBFT instances have decided (line~\ref{line:nowic_decide_rule}), $P_i$ decides an input configuration associated with the first $n - t$ processes whose DBFT instances decided $1$ (constructed at line~\ref{line:input_configuration_nowic}).

\begin{algorithm}
\caption{Non-Authenticated Vector Consensus: Pseudocode (for process $P_i$)}
\label{algorithm:non_authenticated}
\footnotesize
\begin{algorithmic} [1]
\State \textbf{Uses:}
\State \hskip2em Non-Authenticated Byzantine Reliable Broadcast~\cite{B87}, \textbf{instance} $\mathit{brb}$
\State \hskip2em Binary DBFT~\cite{CGL18}, \textbf{instances} $\mathit{dbft}[1]$, ..., $\mathit{dbft}[n]$ \BlueComment{one instance of the binary DBFT algorithm per process}

\medskip
\State \textbf{upon} $\mathsf{init}$:
\State \hskip2em $\mathsf{Map}(\mathsf{Process} \to \mathcal{V}_I)$ $\mathit{proposals}_i \gets \text{empty}$ \BlueComment{received proposals}
% \State \hskip2em $\mathsf{Map}(\mathsf{Process} \to \mathsf{Message})$ $\mathit{messages}_i \gets \text{empty}$ \BlueComment{received \textsc{proposal} messages}

\State \hskip2em $\mathsf{Boolean}$ $\mathit{dbft\_proposing}_i = \mathit{true}$ \BlueComment{is $P_i$ still proposing to the DBFT instances}
\State \hskip2em $\mathsf{Map}(\mathsf{Process} \to \mathsf{Boolean})$ $\mathit{dbft\_proposed}_i \gets \{\mathit{false}, \text{for every } \mathsf{Process}\}$ 
\State \hskip2em $\mathsf{Integer}$ $\mathit{dbft\_decisions}_i \gets 0$ \BlueComment{the number of the DBFT instances which have decided}

\medskip
\State \textbf{upon} $\mathsf{propose}(v \in \mathcal{V}_I)$: \label{line:propose_nowic}
\State \hskip2em \textbf{invoke} $\mathit{brb}.\mathsf{broadcast}\big( \langle \textsc{proposal}, v \rangle \big)$ \BlueComment{broadcast a proposal} \label{line:broadcast_proposal_nowic}

\medskip
\State \textbf{upon} reception of $\mathsf{Message}$ $m = \langle \textsc{proposal}, v_j \in \mathcal{V}_I \rangle$ from process $P_j$: \label{line:receive_proposal_nowic} \BlueComment{delivered from $\mathit{brb}$}
\State \hskip2em $\mathit{proposals}_i[P_j] \gets v_j$
% \State \hskip2em $\mathit{messages}_i[P_j] \gets m$

\State \hskip2em \textbf{if} $\mathit{dbft\_proposing}_i = \mathit{true}$:
\State \hskip4em $\mathit{dbft\_proposed}_i[P_j] \gets \mathit{true}$
\State \hskip4em \textbf{invoke} $\mathit{dbft}[j].\mathsf{propose}(1)$ \label{line:propose_dbft_nowic}

\medskip
\State \textbf{upon} $n - t$ DBFT instances have decided 1 (for the first time): \label{line:dbft_decided_nowic}
\State \hskip2em $\mathit{dbft\_proposing}_i \gets \mathit{false}$
\State \hskip2em \textbf{for} every $\mathsf{Process}$ $P_j$ such that $\mathit{dbft\_proposed}_i[P_j] = \mathit{false}$:
\State \hskip4em $\mathit{dbft\_proposed}_i[P_j] \gets \mathit{true}$
\State \hskip4em \textbf{invoke} $\mathit{dbft}[j].\mathsf{propose}(0)$ \label{line:propose_0_dbft_nowic}

\medskip
\State \textbf{upon} all DBFT instances decided, and, for the first $n - t$ processes $P_j$ such that $\mathit{dbft}[j]$ decided $1$, $\mathit{proposals}_i[P_j] \neq \bot$: \label{line:nowic_decide_rule}
\State \hskip2em $\mathsf{Input\_Configuration}$ $\mathit{vector} \gets $ input configuration with $n - t$ process-proposal pairs corresponding to the first $n - t$ DBFT instances which decided 1 \label{line:input_configuration_nowic} 
\State \hskip2em \textbf{trigger} $\mathsf{decide}(\mathit{vector})$ \label{line:decide_nowic}
\end{algorithmic}
\end{algorithm}

\begin{theorem}
\Cref{algorithm:non_authenticated} is correct.
\end{theorem}
\begin{proof}
% We start by proving \emph{Agreement} of \nowic.
% \emph{Agreement} follows from (1) \emph{Agreement} of DBFT, and (2) \emph{Consistency} of the reliable broadcast primitive.

We start by proving \emph{Termination} of \Cref{algorithm:non_authenticated}.
Eventually, at least $n - t$ DBFT instances decide $1$ due to the fact that (1) no correct process proposes $0$ to any DBFT instance unless $n - t$ DBFT instances have decided $1$ (line~\ref{line:dbft_decided_nowic}), and (2) all correct processes eventually propose $1$ to the DBFT instances which correspond to the correct processes (unless $n - t$ DBFT instances have already decided $1$).
When $n - t$ DBFT instances decide $1$ (line~\ref{line:dbft_decided_nowic}), each correct process proposes to all instances to which it has not yet proposed (line~\ref{line:propose_0_dbft_nowic}).
Hence, eventually all DBFT instances decide, and (at least) $n - t$ DBFT instances decide $1$.
Therefore, the rule at line~\ref{line:nowic_decide_rule} eventually activates at every correct process, which implies that every correct process eventually decides (line~\ref{line:decide_nowic}).

Next, we prove \emph{Vector Validity}.
If a correct process $P$ decides an input configuration with a process-proposal pair $(Q, v)$, $P$ has delivered a \textsc{proposal} message from $Q$ (line~\ref{line:receive_proposal_nowic}).
If $Q$ is correct, due to integrity of the reliable broadcast primitive, $Q$'s proposal was indeed $v$.

Finally, \emph{Agreement} follows from (1) \emph{Agreement} of DBFT, and (2) consistency of the reliable broadcast primitive.
Therefore, \Cref{algorithm:non_authenticated} is correct.
\end{proof}

% As \nowic solves, without authentication, the Byzantine consensus problem with \emph{Vector Validity}, any validity property which satisfies $\mathcal{C}_S$ can be solved without authentication (when $n > 3t$).
% Indeed, we can swap \wic with \nowic in the design of \general (\Cref{algorithm:general}).
The main downside of \Cref{algorithm:non_authenticated} is that its message complexity is $O(n^4)$.
Therefore, non-authenticated version of \general has $O(n^4)$ message complexity, which is not optimal according to our lower bound (\Cref{subsection:lower_bound}).

\subsection{Implementation with $O(n^2 \log n)$ Communication: Pseudocode \& Formal Proofs} \label{subsection:better_communication}

In this subsection, we give an implementation of vector consensus with $O(n^2 \log n)$ communication complexity, which comes within a logarithmic factor of the lower bound (\Cref{subsection:lower_bound}).
This implementation represents a near-linear communication improvement over \Cref{algorithm:interactive_consistency} (\Cref{subsection:general_algorithm}), which achieves $O(n^3)$ communication complexity.
We note that the following solution is highly impractical due to its exponential latency.
However, our solution does represent a step towards closing the existing gap in the communication complexity of consensus with non-trivial (and solvable) validity properties.
% We leave the problem of obtaining a vector consensus algorithm with subcubic communication complexity and polynomial latency for future work.

\subsubsection{Vector Dissemination} \label{subsubsection:vector_dissemination}
First, we formally define the \emph{vector dissemination} problem, which plays the crucial role in our vector consensus algorithm with improved communication complexity.
In this problem, each correct process \emph{disseminates} a vector of exactly $n - t$ values, and all correct processes eventually obtain (1) a hash of some disseminated vector, and (2) a storage proof.
For every hash value $H$ and every storage proof $\mathit{sp}$, we define $\mathsf{valid\_SP}(H, \mathit{sp}) \in \{\mathit{true}, \mathit{false}\}$.
% We say that a storage proof $\mathit{sp}$ is for a vector $\mathit{vec}$ if and only if $\mathsf{valid\_storage\_proof}(\mathit{vec}, \mathit{sp}) = \mathit{true}$.
Formally, the vector dissemination problem exposes the following interface:
\begin{compactitem}
    \item \textbf{request} $\mathsf{disseminate}(\mathsf{Vector} \text{ } \mathit{vec})$: a process disseminates a vector $\mathit{vec}$. 
    
    \item \textbf{indication} $\mathsf{obtain}(\mathsf{Hash\_Value} \text{ } H', \mathsf{Storage\_Proof} \text{ } \mathit{sp}')$: a process obtains a hash value $H'$ and a storage proof $\mathit{sp}'$.
\end{compactitem}
The following properties are required:
\begin{compactitem}
    \item \emph{Termination:} Every correct process eventually obtains a hash value and a storage proof.
    % such that $\mathsf{valid\_SP}(H', \mathit{sp}') = \mathit{true}$.
    
    \item \emph{$\delta$-Closeness:} Let $t_{\mathit{first}}$ denote the first time a correct process obtains a hash value and a storage proof.
    Then, every correct process obtains a hash value and a storage proof by time $\max(\text{GST}, t_{\mathit{first}}) + \delta$.
    
    \item \emph{Redundancy:} Let a (faulty or correct) process store in its local memory a storage proof $\mathit{sp}'$ such that, for some hash value $H'$, $\mathsf{valid\_SP}(H', \mathit{sp'}) = \mathit{true}$.
    Then, (at least) $t + 1$ correct processes have cached a vector $\mathit{vec}'$ such that $\mathsf{hash}(\mathit{vec}') = H'$.
    
    \item \emph{Integrity:} If a correct process obtains a hash value $H'$ and a storage proof $\mathit{sp}'$, the following holds: $\mathsf{valid\_SP}(H', \mathit{sp}') = \mathit{true}$.
\end{compactitem}

\paragraph{Slow broadcast.}
In order to solve the vector dissemination problem, we present a simple algorithm (\Cref{algorithm:slow_1}) which implements \emph{slow broadcast}.
In slow broadcast, each process disseminates its vector in ``one-by-one'' fashion, with a ``waiting step'' between any two sending events.
Specifically, process $P_1$ broadcasts its vector by (1) sending the vector to $P_1$ (line~\ref{line:slow_send}), and then waiting $\delta$ time (line~\ref{line:slow_wait}), (2) sending the vector to $P_2$ (line~\ref{line:slow_send}), and then waiting $\delta$ time (line~\ref{line:slow_wait}), etc.
Process $P_2$ broadcasts its vector in the same manner, but it waits $\delta \cdot n$ time (line~\ref{line:slow_wait}).
Crucially, if the system is synchronous, the waiting time of $P_2$ is (roughly) sufficient for $P_1$ to \emph{completely} disseminate its vector.
This holds for any two processes $P_i$ and $P_j$ with $i < j$.

\begin{algorithm}[h]
\caption{Slow Broadcast: Pseudocode (for process $P_i$)}
\label{algorithm:slow_1}
\footnotesize
\begin{algorithmic} [1]

\State \textbf{upon} $\mathsf{broadcast}( \mathsf{Vector}~\mathit{vec} )$:
\State \hskip2em \textbf{for each} $\mathsf{Process}$ $P_j$:
\State \hskip4em \textbf{send} $\langle \textsc{slow\_broadcast}, \mathit{vec} \rangle~\textbf{to}~P_j$ \label{line:slow_send}
\State \hskip4em \textbf{wait for} $\delta \cdot n^{(i-1)}$ time \label{line:slow_wait}

\medskip
\State \textbf{upon} reception of $\langle \textsc{slow\_broadcast}, \mathsf{Vector} \text{ } \mathit{vec}' \rangle$ from process $P_j$:
\State \hskip2em \textbf{trigger} $\mathsf{deliver}(\mathit{vec}', P_j)$

\end{algorithmic}
\end{algorithm}

% \begin{comment}
% \begin{algorithm}
% \caption{Parsimonious Broadcast: Pseudocode (for process $P_i$)}
% \label{algorithm:slow_1}
% \footnotesize
% \begin{algorithmic} [1]

% \medskip
% \State \textbf{Uses:}
% \State \hskip2em Slow Broadcast, \textbf{instance} $\mathit{slow}$
% \State \hskip2em Clock, \textbf{instance} $\mathit{clock}$

% \medskip
% \State \textbf{upon} $\mathsf{init}$:
% \State \hskip2em $\mathit{clock}.\mathsf{start}(0)$
% \State \hskip2em \textbf{send} $\langle \textsc{speak}, 1 \rangle~\textbf{to}~P_1$

% \medskip
% \State \textbf{function} $\mathsf{speaker}(k)$:
% \State \hskip2em \textbf{return} $(k~\mathbf{mod}~n) + 1$

% \medskip
% \State \textbf{upon} $\mathit{clock}.\mathsf{reached}(T = j\cdot n\Delta), j\in \mathbb{N}^+$:
% \State \hskip2em $\mathit{last} \gets \mathsf{speaker}(j-1)$
% \State \hskip2em $\mathit{next} \gets \mathsf{speaker}(j)$
% \State \hskip2em \textbf{send} $\langle \textsc{silence}, j-1 \rangle~\textbf{to}~P_{\mathit{last}}$
% \State \hskip2em \textbf{send} $\langle \textsc{speak}, j \rangle~\textbf{to}~P_{\mathit{next}}$

% \medskip
% \State \textbf{upon} $\mathsf{broadcast}\big( \mathsf{Message}~\mathit{m} \big)$:
% \State \hskip2em \textbf{for} each $P_j \in \Pi$:
% \State \hskip4em \textbf{send} $\langle \textsc{broadcast}, m \rangle~\textbf{to}~P_j$
% \State \hskip4em \textbf{wait} $\Delta^i$ seconds

% \medskip
% \State \textbf{upon} $\mathit{slow}.\mathsf{deliver}(P_j, m)$:
% \State \hskip2em \textbf{trigger} deliver($P_j, m$)

% \end{algorithmic}
% \end{algorithm}
% \end{comment}

\paragraph{Vector dissemination algorithm.}
Our solution is given in \Cref{algorithm:prep}.
% We underline that we assume that every correct process starts executing \Cref{algorithm:prep} by time $\text{GST} + \delta$.
First, we give a concrete implementation of the $\mathsf{valid\_SP}(\cdot, \cdot)$ function.
Given a hash value $H$ and a storage proof $\mathit{sp}$, $\mathsf{valid\_SP}(H, \mathit{sp}) = \mathit{true}$ if and only if $\mathit{sp}$ is a valid $(n - t)$-threshold signature of $\langle \textsc{stored}, H \rangle$.

Let us explain \Cref{algorithm:prep} from the perspective of a correct process $P_i$.
When $P_i$ starts disseminating its vector $\mathit{vec}$ (line~\ref{line:disseminate_vector}), $P_i$ stores its hash (line~\ref{line:compute_hash}) and slow-broadcasts the vector (line~\ref{line:slow_broadcast}).
Once $P_i$ receives \textsc{stored} messages from $n - t$ distinct processes (line~\ref{line:receive_acknowledgements_vector_dissemination}), $P_i$ combines the received partial signatures into a storage proof (line~\ref{line:create_storage_proof}).
Then, $P_i$ broadcasts (using the best-effort broadcast primitive) the constructed storage proof (line~\ref{line:broadcast_storage_proof}).

Whenever $P_i$ receives a storage proof (line~\ref{line:receive_storage_proof}), $P_i$ checks whether the storage proof is valid (line~\ref{line:check_storage_proof}).
If it is, $P_i$ rebroadcasts the storage proof (line~\ref{line:forward_storage_proof}), obtains a hash value and the storage proof (line~\ref{line:obtain_hash}), and stops participating (i.e., sending and processing messages) in vector dissemination (line~\ref{line:stop_participating}).
Observe that, once $P_i$ stops participating in vector dissemination (line~\ref{line:stop_participating}), it stops participating in slow broadcast, as well.

\begin{algorithm} [h]
\caption{Vector Dissemination: Pseudocode (for process $P_i$)}
\label{algorithm:prep}
\footnotesize
\begin{algorithmic} [1]
\State \textbf{Uses:}
%\State \hskip2em Perfect Links~\cite{cachin2011introduction}, \textbf{instance} $\mathit{pl}$ \BlueComment{one to one links with no guarantees if the sender is faulty}
\State \hskip2em Best-Effort Broadcast~\cite{cachin2011introduction}, \textbf{instance} $\mathit{beb}$ \BlueComment{broadcast with no guarantees if the sender is faulty}
\State \hskip2em Slow Broadcast, \textbf{instance} $\mathit{slow}$ \BlueComment{see \Cref{algorithm:slow_1}}

\medskip
\State \textbf{upon} $\mathsf{init}$:
\State \hskip2em $\mathsf{Hash\_Value} \text{ } H_i \gets \bot$ \BlueComment{hash of the message $P_i$ slow-broadcasts}
\State \hskip2em $\mathsf{Map}(\mathsf{Hash\_Value} \to \mathsf{Vector})$ $\mathit{vectors}_i \gets \text{empty}$ \BlueComment{received vectors}
\State \hskip2em $\mathsf{Set}(\mathsf{Process})$ $\mathit{disseminated}_i \gets \text{empty}$ \BlueComment{processes who have disseminated a vector}

\medskip
\State \textbf{upon} $\mathsf{disseminate}( \mathsf{Vector}~\mathit{vec})$: \label{line:disseminate_vector}
\State \hskip2em $H_i \gets \mathsf{hash}(\mathit{vec})$ \label{line:compute_hash}
\State \hskip2em \textbf{invoke} $\mathit{slow}.\mathsf{broadcast}(\mathit{vec})$ \label{line:slow_broadcast}

\medskip
\State \textbf{upon} $\mathit{slow}.\mathsf{deliver}( \mathsf{Vector}~\mathit{vec}', \mathsf{Process} \text{ } P_j)$: \label{line:deliver_slow_bcast}
\State \hskip2em \textbf{if} $P_j \notin \mathit{disseminated}_i$: \label{line:verify_vector_signature}
\State \hskip4em $\mathit{disseminated}_i \gets \mathit{disseminated}_i \cup \{P_j\}$
\State \hskip4em $\mathit{vectors}_i[\mathsf{hash}(\mathit{vec}')] \gets \mathit{vec}'$ \label{line:store_preimage} \BlueComment{cache $\mathit{vec}'$}
\State \hskip4em \textbf{send} $\langle \textsc{stored}, \mathsf{hash}(\mathit{vec}') \rangle_{\sigma_i}~\textbf{to}~P_j$ \label{line:send_stored} \BlueComment{acknowledge the reception by sending a signature to $P_j$}

\medskip
\State \textcolor{blue}{\(\triangleright\) acknowledgements are received}
\State \textbf{upon} reception of $\mathsf{Message}$ $m_j = \langle \textsc{stored}, \mathsf{Hash\_Value} \text{ } H' \rangle_{\sigma_j}$ such that $H' = H_i$ from $n - t$ distinct processes: \label{line:receive_acknowledgements_vector_dissemination} \label{line:received_n-t_stored}
\State \hskip2em $\mathsf{Storage\_Proof}~\mathit{sp} \gets \mathit{Combine}\big(\{ \sigma \,|\, \sigma \text{ is a signature of a received \textsc{stored} message} \}\big)$ \label{line:create_storage_proof}
\State \hskip2em \textbf{invoke} $\mathit{beb}.\mathsf{broadcast}\big( \langle \textsc{storage\_proof}, H_i, \mathit{sp}\rangle \big)$ \label{line:bcast_storage_proof} \BlueComment{disseminate the storage proof} \label{line:broadcast_storage_proof}

\medskip
\State \textcolor{blue}{\(\triangleright\) a storage proof is received}
\State \textbf{upon} reception of $\mathsf{Message}$ $m = \langle \textsc{storage\_proof}, \mathsf{Hash\_Value} \text{ } H', \mathsf{Storage\_Proof} \text{ } \mathit{sp}'\rangle$: \label{line:receive_storage_proof}
\State \hskip2em \textbf{if} $\mathit{sp}'$ is a valid $(n-t)$-threshold signature of $\langle \textsc{stored}, H' \rangle$: \label{line:check_storage_proof} \BlueComment{check that the storage proof is valid}
\State \hskip4em \textbf{invoke} $\mathit{beb}.\mathsf{broadcast}\big( \langle \textsc{storage\_proof}, H', \mathit{sp}'\rangle \big)$ \label{line:forward_storage_proof} \BlueComment{rebroadcast the storage proof}
\State \hskip4em \textbf{trigger} $\mathsf{obtain}(H', \mathit{sp}')$ \label{line:obtain_hash}
\State \hskip4em \textbf{stop participating} in vector dissemination (and slow broadcast) \label{line:stop_participating}

\end{algorithmic}
\end{algorithm}

\paragraph{Correctness \& complexity of \Cref{algorithm:prep}.}
We start by proving redundancy.

\begin{lemma} \label{lemma:redundancy}
\Cref{algorithm:prep} satisfies redundancy.
\end{lemma}
\begin{proof}
Let a (correct or faulty) process store in its local memory a storage proof $\mathit{sp}'$ such that $\mathsf{valid\_SP}(H', \mathit{sp}') = \mathit{true}$, for some hash value $H'$.
% We know that $\mathsf{valid\_SP}(H', \mathit{sp}') = \mathit{true}$ (by the check at line~\ref{line:check_storage_proof}).
Hence, $n - t$ processes have (partially) signed a \textsc{stored} message for $H'$ (as $\mathsf{valid\_SP}(H', \mathit{sp}') = \mathit{true}$).
Among these $n - t$ processes, at least $t + 1$ are correct (as $n > 3t$).
Before sending (and signing) a \textsc{stored} message for $H'$ (line~\ref{line:send_stored}), all these correct processes have cached a vector $\mathit{vec}'$ (line~\ref{line:store_preimage}), where $\mathsf{hash}(\mathit{vec}') = H'$.
Thus, the lemma.
\end{proof}

Next, we prove $\delta$-closeness.

\begin{lemma} \label{lemma:closeness}
\Cref{algorithm:prep} satisfies $\delta$-closeness.
\end{lemma}
\begin{proof}
Let $P_{\mathit{first}}$ be a correct process which obtains a hash value and a storage proof at time $t_{\mathit{first}}$; this is done at line~\ref{line:obtain_hash}.
Before the aforementioned attainment, $P_{\mathit{first}}$ rebroadcasts the hash value and the storage proof (line~\ref{line:forward_storage_proof}).
Hence, every correct process receives a hash value and storage proof by time $\max(\text{GST}, t_{\mathit{first}}) + \delta$ (line~\ref{line:receive_storage_proof}), which proves the lemma.
\end{proof}

The following lemma proves that, if a correct process $P_i$ starts the dissemination of its vector at time $t_i$, then every correct process obtains a hash value and a storage proof by time $\max(\text{GST}, t_i) + \delta \cdot n^i + 3\delta$.
We emphasize that the $\max(\text{GST}, t_i) + \delta \cdot n^i + 3\delta$ time is not tight; we choose it for simplicity of presentation.

\begin{lemma} \label{lemma:timely_termination}
If a correct process $P_i$ starts the dissemination of its vector at time $t_i$, every correct process obtains a hash value and a storage proof by time $\max(\text{GST}, t_i) + \delta \cdot n^i + 3\delta$.
\end{lemma}
\begin{proof}
We separate the proof into two cases:
\begin{compactitem}
    \item There exists a correct process which obtains a hash value and a storage proof by time $\max(\text{GST}, t_i) + \delta \cdot n^i + 2\delta$.
    In this case, the statement of the lemma holds as every correct process obtains a hash value and a storage proof by time $\max(\text{GST}, t_i) + \delta \cdot n^i + 3\delta$ due to the ``rebroadcasting step'' (line~\ref{line:forward_storage_proof}).
    
    \item There does not exist a correct process which obtains a hash value and a storage proof by time $T = \max(\text{GST}, t_i) + \delta \cdot n^i + 2\delta$.
    Hence, no process stops participating in vector dissemination by time $T$, i.e., no process executes line~\ref{line:stop_participating} by time $T$.
    Every correct process receives a \textsc{slow\_broadcast} message from process $P_i$ by time $\max(\text{GST}, t_i) + \delta \cdot n^i + \delta$.

    Thus, by time $\max(\text{GST}, t_i) + \delta \cdot n^i + 2\delta$, $P_i$ receives $n - t$ partial signatures (line~\ref{line:receive_acknowledgements_vector_dissemination}).
    Finally, by time $\max(\text{GST}, t_i) + \delta \cdot n^i + 3\delta$, every correct process receives a \textsc{storage\_proof} message from $P_i$ (line~\ref{line:receive_storage_proof}), and obtains a hash value and a storage proof (line~\ref{line:obtain_hash}).
    In this case, the statement of the lemma holds.
\end{compactitem}
As the statement of the lemma holds in both cases, the proof is concluded.
\end{proof}

The next lemma proves that \Cref{algorithm:prep} satisfies termination.

\begin{lemma} \label{lemma:termination_prep}
\Cref{algorithm:prep} satisfies termination.
\end{lemma}
\begin{proof}
Follows directly from \Cref{lemma:timely_termination}.
\end{proof}

Next, we prove integrity.

\begin{lemma} \label{lemma:integrity}
\Cref{algorithm:prep} satisfies integrity.
\end{lemma}
\begin{proof}
Follows from the check at line~\ref{line:check_storage_proof}.
\end{proof}

Therefore, \Cref{algorithm:prep} solves the vector dissemination problem.

\begin{theorem}
\Cref{algorithm:prep} is correct.
\end{theorem}

Lastly, we prove that the communication complexity of \Cref{algorithm:prep} is $O(n^2)$.
Recall that the communication complexity denotes the number of bits sent by correct processes at and after GST.

\begin{theorem}\label{theorem:quadratic_dissemination}
Let no correct process start the dissemination of its vector after time $\text{GST} +  \delta$.
Then, the communication complexity of \Cref{algorithm:prep} is $O(n^2)$. 
\end{theorem}
\begin{proof}
Let $i$ be the minimum index such that (1) process $P_i$ is correct, and (2) $P_i$ sends a \textsc{slow\_broadcast} message at some time $\geq \text{GST}$.
If $i$ does not exist, the lemma trivially holds.

Let $t_i$ denote the time at which $P_i$ starts the dissemination of its vector (line~\ref{line:disseminate_vector}).
By assumption, $t_i \leq \text{GST} + \delta$.
Every correct process obtains a hash value and a storage proof by time $\max(\text{GST}, t_i) + \delta \cdot n^i + 3\delta$ (by \Cref{lemma:timely_termination}).
Thus, as $t_i \leq \text{GST} + \delta$, every correct process obtains a hash value and a storage proof by time $\text{GST} + \delta \cdot n^i + 4\delta$.
Moreover, by time $\text{GST} + \delta \cdot n^i + 4\delta$, all correct processes stop sending \textsc{slow\_broadcast} messages (due to line~\ref{line:stop_participating}).

Let $P_j$ be a correct process such that $j > i$.
Due to the slow broadcast primitive (\Cref{algorithm:slow_1}), $P_j$ has a ``waiting step'' of (at least) $\delta \cdot n^i $ time (after GST).
Therefore, during the $[\text{GST}, \text{GST} + \delta \cdot n^i + 4\delta]$ period, $P_j$ can send only $O(1)$ \textsc{slow\_broadcast} messages.
Thus, at most one correct process (i.e., $P_i$) sends more than $O(1)$ \textsc{slow\_broadcast} messages during the $[\text{GST}, \text{GST} + \delta \cdot n^i + 4\delta]$ period; that process sends at most $n$ \textsc{slow\_broadcast} messages.
As each message is of size $O(n)$ (since it carries a vector of $n - t$ values), the communication complexity of \Cref{algorithm:prep} is $O(n) \cdot O(1) \cdot O(n) + 1 \cdot O(n) \cdot O(n) = O(n^2)$.
% Thus, the lemma.
\end{proof}

\subsubsection{Vector Consensus with $O(n^2\log n)$ Communication Complexity}
Finally, we are ready to present our vector consensus algorithm (\Cref{algorithm:better_interactive_consistency}) with subcubic communication complexity.
Our algorithm consists of three building blocks: (1) vector dissemination (\Cref{subsubsection:vector_dissemination}), (2) \textsc{Quad} (\Cref{subsubsection:interactive_consistency}), and (3) \textsc{add}~\cite{das2021asynchronous}, an algorithm for asynchronous data dissemination.
In \Cref{algorithm:better_interactive_consistency}, we rely on a specific instance of \textsc{Quad} in which (1) each proposal value is a hash value, and (2) given a hash value $H$ and a (\textsc{Quad}'s) proof $\Sigma$,\footnote{Do not confuse \textsc{Quad}'s proofs with storage proofs of the vector dissemination problem (\Cref{subsubsection:vector_dissemination}).}  $\mathsf{verify}(H, \Sigma) = \mathit{true}$ if and only if $\mathsf{valid\_SP}(H, \Sigma) = \mathit{true}$ (recall the vector dissemination problem; \Cref{subsubsection:vector_dissemination}).
Below, we briefly explain \textsc{add}.

\paragraph{\textsc{add}.}
This algorithm solves the \emph{data dissemination}~\cite{das2021asynchronous} problem defined in the following way.
Let $M$ be a data blob which is an input of (at least) $t + 1$ correct processes; other correct processes have $\bot$ as their input.
The data dissemination problem requires every correct process to eventually output $M$, and no other message.
The key feature of \textsc{add} is that it solves the problem with $O(n^2 \log n)$ communication complexity.
% In our case, we will use \textsc{add} to ``reconstruct'' a disseminated vector of $n - t$ values.
(For full details on \textsc{add}, refer to~\cite{das2021asynchronous}.)

\paragraph{Description of vector consensus.}
We give the description of \Cref{algorithm:better_interactive_consistency} from the perspective of a correct process $P_i$.
When $P_i$ proposes its value (line~\ref{line:propose_log}), it disseminates the value (using the best-effort broadcast primitive) to all processes (line~\ref{line:bcast_proposal}).
Once $P_i$ receives proposals of $n - t$ distinct processes (line~\ref{line:received_n-t_proposals_before_dissemination}), it constructs an input configuration (line~\ref{line:construct_vector_before_dissemination}), and starts disseminating it (line~\ref{line:disseminate}).\footnote{Recall that this input configuration is actually a vector of $n - t$ values.}

When $P_i$ obtains a hash value $H$ and a storage proof $\mathit{sp}$ (line~\ref{line:prep_store}), $P_i$ proposes $(H, \mathit{sp})$ to \textsc{Quad} (line~\ref{line:quad_propose}).
Observe that $\mathsf{verify}(H, \mathit{sp}) = \mathit{true}$ (due to the integrity property of vector dissemination).
Once $P_i$ decides from \textsc{Quad} (line~\ref{line:quad_decide}), it starts \textsc{add} (line~\ref{line:add_input}).
Specifically, $P_i$ checks whether it has cached an input configuration whose hash value is $H'$ (line~\ref{line:check_cache}).
If so, $P_i$ inputs the input configuration to \textsc{add}; otherwise, $P_i$ inputs $\bot$.
Once $P_i$ outputs an input configuration from \textsc{add} (line~\ref{line:add_output}), it decides it (line~\ref{line:decide_better}).

\begin{algorithm}
\caption{$O(n^2 \log n)$ Vector Consensus: Pseudocode (for process $P_i$)}
\label{algorithm:better_interactive_consistency}
\footnotesize
\begin{algorithmic} [1]
\State \textbf{Uses:}
\State \hskip2em Best-Effort Broadcast~\cite{cachin2011introduction}, \textbf{instance} $\mathit{beb}$ \BlueComment{broadcast with no guarantees if the sender is faulty}
\State \hskip2em Vector Dissemination, \textbf{instance} $\mathit{disseminator}$ \BlueComment{see \Cref{algorithm:prep}}
\State \hskip2em \textsc{Quad}~\cite{civit2022byzantine}, \textbf{instance} $\mathit{quad}$
\State \hskip2em \textsc{add}~\cite{das2021asynchronous}, \textbf{instance} $\mathit{add}$

\medskip
\State \textbf{upon} $\mathsf{init}$:
\State \hskip2em $\mathsf{Integer}$ $\mathit{received\_proposals}_i \gets 0$ \BlueComment{the number of received proposals}
\State \hskip2em $\mathsf{Map}(\mathsf{Process} \to \mathcal{V}_I)$ $\mathit{proposals}_i \gets \text{empty}$ \BlueComment{received proposals}
\State \hskip2em $\mathsf{Map}(\mathsf{Process} \to \mathsf{Message})$ $\mathit{messages}_i \gets \text{empty}$ \BlueComment{received \textsc{proposal} messages}
% \State \hskip2em $\mathsf{Map}(\mathsf{Hash\_Value} \to \mathsf{Input\_Configuration})$ $\mathit{vectors}_i \gets \text{empty}$ \BlueComment{received vectors}

\medskip
\State \textbf{upon} $\mathsf{propose}(v \in \mathcal{V}_I)$: \label{line:propose_log}
\State \hskip2em \textbf{invoke} $\mathit{beb}.\mathsf{broadcast}\big( \langle \textsc{proposal}, v \rangle_{\sigma_i} \big)$ \label{line:bcast_proposal} \BlueComment{broadcast a signed proposal}

\medskip
\State \textbf{upon} reception of $\mathsf{Message}$ $m = \langle \textsc{proposal}, v_j \in \mathcal{V}_I \rangle_{\sigma_j}$ from process $P_j$ and $\mathit{received\_proposals}_i < n - t$:
\State \hskip2em $\mathit{received\_proposals}_i \gets \mathit{received\_proposals}_i + 1$
\State \hskip2em $\mathit{proposals}_i[P_j] \gets v_j$
\State \hskip2em $\mathit{messages}_i[P_j] \gets m$

\State \hskip2em \textbf{if} $\mathit{received\_proposals}_i = n - t$: \label{line:received_n-t_proposals_before_dissemination} \BlueComment{received $n - t$ proposals; can start disseminating}
\State \hskip4em $\mathsf{Input\_Configuration}$ $\mathit{vector} \gets $ input configuration constructed from $\mathit{proposals}_i$ \label{line:construct_vector_before_dissemination}
% \State \hskip4em $\mathsf{Proof}$ $\Sigma \gets $ set of messages containing all \textsc{proposal} messages from $\mathit{messages}_i$
\State \hskip4em \textbf{invoke} $\mathit{disseminator}.\mathsf{disseminate}(\mathit{vector})$ \label{line:disseminate}

\medskip
\State \textbf{upon} $\mathit{disseminator}.\mathsf{obtain}\big( (\mathsf{Hash\_Value}~\mathit{H}, \mathsf{Storage\_Proof}~\mathit{sp}) \big)$: \label{line:prep_store}
% \State \hskip2em $\mathit{vectors}_i[H] \gets \mathit{vector}$
\State \hskip2em \textbf{if} have not yet proposed to \textsc{Quad}:
% \BlueComment{vector is prepared for \textsc{ADD}; can propose its hash to \textsc{Quad}}
\State \hskip4em \textbf{invoke} $\mathit{quad}.\mathsf{propose}\big( (\mathit{H}, \mathit{sp}) \big)$ \label{line:quad_propose}

\medskip
\State \textbf{upon} $\mathit{quad}.\mathsf{decide}\big( (\mathsf{Hash\_Value}~\mathit{H}', \mathsf{Storage\_Proof}~\mathit{sp}') \big)$: \label{line:quad_decide}
\State \hskip2em $\mathsf{Input\_Configuration}$ $\mathit{vector}' \gets$ a cached vector whose hash value is $H'$ \BlueComment{can be $\bot$} \label{line:check_cache}
\State \hskip2em \textbf{invoke} $\mathit{add}.\mathsf{input}( \mathit{vector}' )$ \label{line:add_input}

\medskip
\State \textbf{upon} $\mathit{add}.\mathsf{output}\big(\mathsf{Input\_Configuration} \text{ } \mathit{vector}'' \big)$: \label{line:add_output}
\State \hskip2em \textbf{trigger} $\mathsf{decide}(\mathit{vector}'')$ \label{line:decide_better}

\end{algorithmic}
\end{algorithm}

\paragraph{Correctness \& complexity of \Cref{algorithm:better_interactive_consistency}.}

We start by proving that (1) all correct processes eventually output a non-$\bot$ value from \textsc{add}, and (2) no two correct processes output different values from \textsc{add}.

\begin{lemma} \label{lemma:eventually_add}
The following holds:
\begin{compactitem}
    \item Every correct process eventually outputs a non-$\bot$ value from \textsc{add} (line~\ref{line:add_output}); moreover, the output value was an input (to \textsc{add}) of a correct process.

    \item No two correct processes output different input configurations from \textsc{add} (line~\ref{line:add_output}).
\end{compactitem}
\end{lemma}
\begin{proof}
First, every correct process broadcasts its proposal (line \ref{line:bcast_proposal}).
Thus, every correct process eventually receives $n-t$ proposals (line \ref{line:received_n-t_proposals_before_dissemination}), and starts the dissemination of an input configuration (line~\ref{line:disseminate}).
Due to the termination property of vector dissemination (\Cref{lemma:termination_prep}), every correct process eventually obtains a hash value and a storage proof (line~\ref{line:prep_store}).
Hence, every correct process eventually proposes to \textsc{Quad} (line~\ref{line:quad_propose}).
Due to \emph{Termination} of \textsc{Quad}, every correct process eventually decides from \textsc{Quad} (line~\ref{line:quad_decide}), and starts executing \textsc{add} (line~\ref{line:add_input}).

As the pair decided from \textsc{Quad} (recall that \textsc{Quad} satisfies \emph{Agreement}) includes a storage proof, at least $t + 1$ correct processes have cached an input configuration whose hash value is decided from \textsc{Quad} (by redundancy of vector dissemination).
Therefore, all of these correct processes input the same non-$\bot$ value to \textsc{add} (line~\ref{line:add_input}); let that value be $\mathit{vec}$.
Moreover, no correct process inputs a different non-$\bot$ value to \textsc{add}.
Therefore, the conditions required by \textsc{add} are preserved, which implies that all correct processes eventually output $\mathit{vec} \neq \bot$ from \textsc{add} (line~\ref{line:add_output}).
\end{proof}

The following theorem proves that \Cref{algorithm:better_interactive_consistency} is correct.

\begin{theorem}
\Cref{algorithm:better_interactive_consistency} is correct.
\end{theorem}
\begin{proof}
Let us prove that \Cref{algorithm:better_interactive_consistency} satisfies all properties of vector consensus.
\emph{Agreement} and \emph{Termination} follow directly from \Cref{lemma:eventually_add}.

It is left to prove \emph{Vector Validity}.
Let $\mathit{vec}'$ be an input configuration of $n - t$ proposals decided by a correct process (line~\ref{line:decide_better}).
Hence, $\mathit{vec}'$ is an input (to \textsc{add}) of a correct process (by \Cref{lemma:eventually_add}), which implies that some correct process has previously cached $\mathit{vec}'$.
% Hence, a storage proof $\mathit{sp}'$, where $\mathsf{valid\_SP}(\mathsf{hash}(\mathit{vec}'), \mathit{sp}') = \mathit{true}$, is locally stored by a correct process at line~\ref{line:quad_decide} (by \Cref{lemma:eventually_add}).
    % Therefore, $\mathit{vec}'$ is cached by (at least) $t + 1$ correct processes (due to the redundancy property of vector dissemination).
Before a correct process caches a vector (\Cref{algorithm:prep}), it verifies that it is associated with corresponding \textsc{proposal} messages; we omit this check for brevity.
As correct processes only send \textsc{proposal} messages for their proposals (line~\ref{line:bcast_proposal}), \emph{Vector Validity} is satisfied.
\end{proof}

Lastly, we show the communication complexity of \Cref{algorithm:better_interactive_consistency}.

\begin{theorem}
The communication complexity of \Cref{algorithm:better_interactive_consistency} is $O(n^2 \log n)$.
\end{theorem}
\begin{proof}
The communication complexity of a single best-effort broadcast instance is $O(n)$.
Every correct process starts the dissemination of its vector by time $\text{GST} + \delta$ (as every correct process receives $n - t$ proposals by this time).
Thus, the communication complexity of vector dissemination is $O(n^2)$ (by \Cref{theorem:quadratic_dissemination}).
The communication complexity of \textsc{Quad} is $O(n^2)$ as correct processes start executing it either (1) by $\text{GST} + \delta$, or (2) within $\delta$ time from each other (due to the $\delta$-closeness property of vector dissemination); see paragraph ``A note on \textsc{Quad}'' in \Cref{subsection:authenticated_vector_proof}.
Moreover, the communication complexity of \textsc{add} is $O(n^2 \log n)$ (see~\cite{das2021asynchronous}).
As \Cref{algorithm:better_interactive_consistency} is a composition of the aforementioned building blocks, its communication complexity is $n \cdot O(n) + O(n^2) + O(n^2) + O(n^2 \log n) = O(n^2 \log n)$.
\end{proof}
