# Supplementary material for: Partial Synchrony for Free? New Upper Bounds for Byzantine Agreement
Source: arXiv:2402.10059 source file (2024-10-23)
Supplement: Supplementary file 6 [file graded_consensus_correctness.tex]

\section{AW Graded Consensus: Proof of Correctness \& Complexity} \label{subsection:aw_correctness}

In this section, we prove that the AW graded consensus algorithm, introduced in~\cite{AttiyaWelch23}, satisfies the validity, consistency, and termination properties of graded consensus.
As underlined in \Cref{subsection:graded_consensus}, the AW algorithm is designed for a slightly different notion of graded consensus than the one we consider.

\paragraph{The graded consensus problem of~\cite{AttiyaWelch23}.}
The graded consensus problem defined in~\cite{AttiyaWelch23} exposes the same interface as the one we introduced in \Cref{subsection:graded_consensus}, except that it does not incorporate the $\mathsf{abandon}()$ operation.
Hence, no correct process ever abandons the graded consensus problem of~\cite{AttiyaWelch23}.
Moreover, the graded consensus problem of~\cite{AttiyaWelch23} assumes that all correct processes eventually propose; recall that this might not be the case with our notion of the graded consensus problem.
Finally, graded consensus of~\cite{AttiyaWelch23} needs to satisfy the following properties:
\begin{compactitem}
    \item \emph{AW-Validity:} If all correct processes propose the same value $\mathit{val}$ and a correct process decides a pair $(\mathit{val}', g')$, then $\mathit{val}' = \mathit{val}$ and $g' = 1$. 

    \item \emph{AW-Consistency:} If a correct process decides a pair $(\mathit{val}, 1)$, no correct process decides a pair $(\mathit{val}' \neq \mathit{val}, *)$.

    \item \emph{AW-Termination:} Every correct process eventually decides.
\end{compactitem}

% \paragraph{Executions of the AW algorithm.}
% Any execution of the AW algorithm is a totally ordered sequence of (1) message-sending events, (2) message-reception events, and (3) internal events (e.g., invoking the $\mathsf{propose}(\cdot)$ operation, updating a local variable, etc.)

% Any execution of the AW algorithm is a totally ordered sequence of events $\mathcal{E}_{\text{AW}}$ such that the following properties are satisfied:
% \begin{compactitem}
%     \item \emph{Message safety:} If a (correct or faulty) process $p_i$ receives a message $m$ in $\mathcal{E}_{\text{AW}}$, then $m$ was previously sent in $\mathcal{E}_{\text{AW}}$.

%     \item \emph{Message liveness:} If $\mathcal{E}_{\text{AW}}$ is infinite, then any message $m$ that is sent in $\mathcal{E}_{\text{AW}}$ is received in $\mathcal{E}_{\text{AW}}$.

%     \item \emph{Behavior validity:}
% \end{compactitem}

\paragraph{Proof.}
We now prove that the AW algorithm solves the graded consensus problem as defined in \Cref{subsection:graded_consensus}.
First, we prove that the AW algorithm satisfies validity.

\begin{lemma}
The AW algorithm satisfies validity.
\end{lemma}
\begin{proof}
By contradiction, suppose that the AW algorithm does not satisfy validity.
Hence, there exists a finite execution $\mathcal{E}$ in which (1) all correct processes that propose to the AW algorithm propose the same value $\mathit{val}$, and (2) a correct process decides a pair $(\mathit{val}' \neq \mathit{val}, *)$ or $(\mathit{val}, 0)$.
We now construct a finite execution $\mathcal{E}'$ in which the AW algorithm violates the AW-validity property:
\begin{compactenum}
    \item A process is correct in $\mathcal{E}'$ if and only if it is correct in $\mathcal{E}$.

    \item Then, $\mathcal{E}' \gets \mathcal{E}$.
    That is, execution $\mathcal{E}'$ is identical to $\mathcal{E}$ after this step.

    \item For every correct process $p_i$ that invokes the $\mathsf{abandon}()$ operation in execution $\mathcal{E}$:
    \begin{compactenum}
        \item For every message $m$ received by $p_i$ after the invocation of the $\mathsf{abandon}()$ operation in $\mathcal{E}$, we remove the reception of $m$ from $\mathcal{E}'$.
        (Observe that $p_i$ does not send any message or perform any local computation after it has invoked the $\mathsf{abandon}()$ operation in $\mathcal{E}$.)

        \item We remove the invocation of the $\mathsf{abandon}()$ operation from $\mathcal{E}'$.
    \end{compactenum}
    This step ensures that no correct process abandons the AW algorithm in $\mathcal{E}'$.

    \item For every correct process $p_j$ that does not propose to the AW algorithm in $\mathcal{E}$, we make $p_j$ propose value $\mathit{val}$ at the end of $\mathcal{E}'$.
    This step ensures that all correct processes propose value $\mathit{val}$ in $\mathcal{E}'$.
\end{compactenum}
The following holds for the constructed execution $\mathcal{E}'$: (1) all correct processes propose to the AW algorithm, (2) no correct process abandons the AW algorithm, (3) all correct processes propose value $\mathit{val}$, and (4) a correct process decides a pair $(\mathit{val}' \neq \mathit{val}, *)$ or $(\mathit{val}, 0)$.
Therefore, execution $\mathcal{E}'$ violates AW-validity of the AW algorithm, which is impossible as the AW algorithm satisfies AW-validity (as proven in~\cite{AttiyaWelch23}).
Thus, the starting assumption must be wrong, which implies that the AW algorithm satisfies validity.
\end{proof}

Next, we prove that the AW algorithm satisfies consistency.

\begin{lemma}
The AW algorithm satisfies consistency.
\end{lemma}
\begin{proof}
We prove the lemma by contradiction.
Hence, suppose that the AW algorithm does not satisfy consistency.
Therefore, there exists a finite execution $\mathcal{E}$ in which (1) a correct process decides a pair $(\mathit{val}, 1)$, and (2) a correct process decides a pair $(\mathit{val}' \neq \mathit{val}, *)$.
We now build a finite execution $\mathcal{E}'$ in which the AW algorithm violates AW-consistency:
\begin{compactenum}
    \item A process is correct in $\mathcal{E}'$ if and only if it is correct in $\mathcal{E}$.

    \item Then, $\mathcal{E}' \gets \mathcal{E}$.
    That is, execution $\mathcal{E}'$ is identical to $\mathcal{E}$ after this step.

    \item For every correct process $p_i$ that invokes the $\mathsf{abandon}()$ operation in execution $\mathcal{E}$:
    \begin{compactenum}
        \item For every message $m$ received by $p_i$ after the invocation of the $\mathsf{abandon}()$ operation in $\mathcal{E}$, we remove the reception of $m$ from $\mathcal{E}'$.
        (Observe that $p_i$ does not send any message or perform any local computation after it has invoked the $\mathsf{abandon}()$ operation in $\mathcal{E}$.)

        \item We remove the invocation of the $\mathsf{abandon}()$ operation from $\mathcal{E}'$.
    \end{compactenum}
    This step ensures that no correct process abandons the AW algorithm in $\mathcal{E}'$.

    \item For every correct process $p_j$ that does not propose to the AW algorithm in $\mathcal{E}$, we make $p_j$ propose any value at the end of $\mathcal{E}'$.
    This step ensures that all correct processes propose in $\mathcal{E}'$.
\end{compactenum}
The following is satisfied for the built execution $\mathcal{E}'$: (1) all correct processes propose to the AW algorithm, (2) no correct process abandons the AW algorithm, (3) a correct process decides a pair $(\mathit{val}, 1)$, and (4) a correct process decides a pair $(\mathit{val}' \neq \mathit{val}, *)$.
Therefore, $\mathcal{E}'$ indeed violates AW-consistency, which is impossible as the AW algorithm satisfies AW-consistency.
Hence, the starting assumption must be wrong: the AW algorithm satisfies consistency.
\end{proof}

Finally, we prove that the AW algorithm satisfies termination.

\begin{lemma}
The AW algorithm satisfies termination.
\end{lemma}
\begin{proof}
The lemma follows directly from the fact that the AW algorithm satisfies AW-termination.
\end{proof}
