# Supplementary material for: Partial Synchrony for Free? New Upper Bounds for Byzantine Agreement
Source: arXiv:2402.10059 source file (2024-10-23)
Supplement: Supplementary file 7 [file lower_bound.tex]

\section{Lower Bound on Message Complexity: Formal Proof} \label{section:lower_bound_appendix}

In this section, we give a formal proof of \Cref{lemma:final_lemma_lower_bound}.
Recall that we have fixed an algorithm $\mathcal{A}$ which solves the Byzantine consensus problem with a non-trivial validity property $\mathit{val}$.

\begin{theorem_lower_bound} [restated]
The message complexity of $\mathcal{E}_{\mathit{base}}$ is at least $(\lceil \frac{t}{2} \rceil)^2$.
\end{theorem_lower_bound}
\begin{proof}
By \Cref{lemma:behavior_without_receptions}, there exists a behavior $\beta_Q$ of process $Q$ in which $Q$ decides a value $v_Q$ without having received any message (from any other process).
Let $t_Q$ denote the time at which $Q$ decides $v_Q$ in $\beta_Q$.
Moreover, there exists an \add{infinite} execution $\mathcal{E}_{v}$ in which (1) $Q$ is faulty and silent, and (2) correct processes decide a value $v \neq v_Q$ (by \Cref{lemma:conflicting_execution}).
Let $t_{v}$ denote the time at which a correct process decides $v \neq v_Q$ in $\mathcal{E}_{v}$.

We now construct an execution $\mathcal{E}$ in the following way:
\begin{compactenum}
    \item Processes in $\mathit{Corr}_{\mathcal{A}}(\mathcal{E}_{v}) \cup \{Q\}$ are correct in $\mathcal{E}$.
    All other processes are faulty.
    
    \item All messages from and to $Q$ are delayed until after $\max(t_Q, t_{v})$.
    
    \item Process $Q$ exhibits the behavior $\beta_Q$.
    
    \item Until $\max(t_Q, t_{v})$, no process in $\mathit{Corr}_{\mathcal{A}}(\mathcal{E}_{v})$ can distinguish $\mathcal{E}$ from $\mathcal{E}_{v}$.
    
    \item GST is set to after $\max(t_Q, t_{v})$.
\end{compactenum}
As no process in $\mathit{Corr}_{\mathcal{A}}(\mathcal{E}_{v})$ can distinguish $\mathcal{E}$ from $\mathcal{E}_{v}$ until $\max(t_Q, t_{v})$, $v \neq v_Q$ is decided by a correct process in $\mathcal{E}$.
Moreover, $Q$ decides $v_Q$ in $\mathcal{E}$ (step 3 of the construction).
Thus, \emph{Agreement} is violated in $\mathcal{E}$, which contradicts the fact that $\mathcal{A}$ satisfies \emph{Agreement}.
Hence, the starting assumption is not correct: in $\mathcal{E}_{\mathit{base}}$, correct processes send (at least) $(\lceil \frac{t}{2} \rceil)^2$ messages.
% , which concludes the proof.
% implies that the message complexity of $\mathcal{A}$ is $\Omega(t^2)$.
\end{proof}
