# Supplementary material for: Partial Synchrony for Free? New Upper Bounds for Byzantine Agreement
Source: arXiv:2402.10059 source file (2024-10-23)
Supplement: Supplementary file 10 [file proof.tex]

\section{Full Computational Model} \label{section:full_model}

\paragraph{Messages.}
Each message has its sender and receiver.
Given a message $m$, $\mathsf{sender}(m) \in \Pi$ (resp., $\mathsf{receiver}(m) \in \Pi$) denotes the sender (resp., the receiver) of the message $m$.

\paragraph{Events.}
A run of the system unfolds in discrete \emph{events}.
Formally, an event $e$ is a pair $(P, \mathit{action})$, where (1) $P \in \Pi$ is a process at which $e$ occurs, and (2) $\mathit{action} \in \{\mathsf{start}, \mathsf{decide}(v), \mathsf{send}(m), \mathsf{receive}(m), \mathsf{heartbeat}\}$ is the occurring action.
The $\mathsf{start}$ action is a symbolic action signalizing that the process has ``woken up''.
Similarly, the $\mathsf{heartbeat}$ action is a symbolic action signalizing that the process is still ``alive''.
We assume that correct processes trigger infinitely many $\mathsf{heartbeat}$ events in an infinite run of the system (i.e., we assume that correct processes are always ``online'').
% For instance, $\big( P, \mathsf{start}(v) \big)$ denotes that process $P$ starts with a proposal $v \in \mathcal{V}$, whereas $\big( P, \mathsf{decide}(v') \big)$ denotes that $P$ decides $v' \in \mathcal{V}$.

The following holds for each event $e$:
\begin{compactitem}
    \item If $e = \big( P, \mathsf{send}(m) \big)$, then $P = \mathsf{sender}(m)$.
    That is, a process can only send its own messages.
    
    \item If $e = \big( Q, \mathsf{receive}(m) \big)$, then $Q = \mathsf{receiver}(m)$.
    That is, a process can only receive messages intended to it.
\end{compactitem}
Given a sequence of events $\mathcal{S}$ and an event $e$, we write ``$e \in \mathcal{S}$'' to mean that $e$ belongs to $\mathcal{S}$.
Moreover, $\mathcal{S}|_P$ denotes the subsequence of $\mathcal{S}$ that contains only events occurring on the process $P \in \Pi$.
% , where $P \in \Pi$ is a process.
We denote by $|\mathcal{S}|$ the length of $\mathcal{S}$, i.e., the number of events in $\mathcal{S}$.
Lastly, $\mathcal{S}[i]$ denotes the $i$-th event of $\mathcal{S}$, where $1 \leq i \leq |\mathcal{S}|$.

\paragraph{Behaviors \& executions.}
A \emph{behavior} of a process $P$ is a sequence of events $\beta_P$ such that:
\begin{compactenum}
    \item For every event $e \in \beta_P$, $e$ occurs on $P$.
    
    \item At most one $\big( P, \mathsf{start} \big)$ event belongs to $\beta_p$.
    Moreover, if $|\beta_P| > 0$, the first event of $\beta_P$ is $\big( P, \mathsf{start} \big)$.

    % \item If $|\beta_P| > 0$, the first event of $\beta_P$ is $\big( P, \mathsf{start}(v) \big)$, for some value $v \in \mathcal{V}$.
    % Moreover, at most one $\big( P, \mathsf{start}(\cdot) \big)$ event belongs to $\beta_P$.
    
    % \item For every event $e \in \beta_P$ such that $e = \big( P, \mathsf{receive}(m) \big)$ and $\mathsf{sender}(m) = P$, $e$ is associated with a unique event $e' = \big( P, \mathsf{send}(m) \big)$ such that $e'$ precedes $e$ in $\beta_P$.
    % That is, each received message (with the sender $P$) was previously sent.
\end{compactenum}
For every algorithm $\mathcal{A}$, every process $P \in \Pi$, and every behavior $\beta_P$ of $P$, we define the $\mathsf{valid}(\mathcal{A}, P, \beta_P) \in \{\mathit{true}, \mathit{false}\}$ function.
The $\mathsf{valid}(\mathcal{A}, P, \beta_P) = \mathit{true}$ if and only if $\beta_P$ is a behavior of $P$ which complies with the algorithm $\mathcal{A}$.
If $\mathsf{valid}(\mathcal{A}, P, \beta_P) = \mathit{true}$, we say that $\beta_P$ is \emph{valid} according to the algorithm $\mathcal{A}$.
We assume that $\mathsf{valid}(\mathcal{A}, P, \text{empty behavior}) = \mathit{true}$, for any algorithm $\mathcal{A}$ and any process $P \in \Pi$.
Similarly, we assume that $\mathsf{valid}(\mathcal{A}, P, (P, \mathsf{start})) = \mathit{true}$, for any algorithm $\mathcal{A}$ and any process $P \in \Pi$.

An \emph{execution} of an algorithm $\mathcal{A}$ is a tuple $\mathcal{E} = (\mathcal{A}, c, \mathcal{F}, \epsilon, \text{GST})$, where $\mathcal{A}$ is a protocol, $c \in \mathcal{I}$ is an input configuration mapping (correct) processes into their proposals, $\mathcal{F} \subset \Pi$ is a set of faulty processes ($|\mathcal{F}| \leq t$) which complies with $c$ ($\mathcal{F} = \Pi \setminus{\process{c}}$), $\epsilon$ is a totally-ordered sequence of events, and $\text{GST}$ is a time.
Each event is marked with a time at which it occurred; given an event $e \in \epsilon$, $\mathsf{time}(e, \epsilon)$ denotes the time at which $e$ occurred in the sequence $\epsilon$.
We allow multiple events to happen at the same time; however, $\epsilon$ arranges them in a total order.

The following holds for each execution $\mathcal{E} = (\mathcal{A}, c, \mathcal{F}, \epsilon, \text{GST})$ of an algorithm $\mathcal{A}$:
\begin{compactenum}
    \item For every process $P \in \Pi$, $\epsilon|_P$ is a behavior of $P$.
    
    \item If $\epsilon$ is infinite, then, for every process $P \in \Pi \setminus{\mathcal{F}}$, $\epsilon|_P$ includes infinitely many $\big( P, \mathsf{heartbeat} \big)$ events.
    That is, correct process are live.
    
    \item For every process $P \in \Pi \setminus{\mathcal{F}}$, the proposal of $P$ in $\mathcal{E}$ is determined by $c$.
    That is, $c$ represents the proposal assignments (of correct processes) in $\mathcal{E}$.
    
    \item For every process $P \in \Pi \setminus{\mathcal{F}}$, $\mathsf{valid}(\mathcal{A}, P, \epsilon|_P) = \mathit{true}$.
    That is, for every correct process $P$, its behavior is valid according to the algorithm $\mathcal{A}$.

    \item For every event $e \in \epsilon$ such that $e = \big( Q, \mathsf{receive}(m) \big)$, $e$ is associated with an event $e' = \big( P, \mathsf{send}(m) \big)$ (we write ``$e' \to e$'').\footnote{Observe that a $\mathsf{send}$ event can be associated with at most one $\mathsf{receive}$ event. Moreover, a $\mathsf{receive}$ event is associated with at exactly one $\mathsf{send}$ event.}
    Moreover, $e'$ precedes $e$ in $\epsilon$.
    That is, each received message was previously sent.
    
    \item Let $T = \mathsf{time}(\epsilon[|\epsilon|], \mathcal{E})$ be the time at which the last event of $\mathcal{E}$ occurs.
    If $T > \text{GST}$, then $e \in \epsilon$ and $\mathsf{time}(e, \epsilon) \leq \text{GST}$, where $e = \big( P, \mathsf{start} \big)$, for every process $P \in \Pi \setminus{\mathcal{F}}$.
    That is, all correct processes start by GST.
    
    \item If $\epsilon$ is infinite, then, for every event $e \in \epsilon$ such that $e = \big( P, \mathsf{send}(m) \big)$, there exists an event $e' \in \epsilon$ such that (1) $e' = \big( P, \mathsf{receive}(m) \big)$, and (2) $e \to e'$.
    That is, if $\epsilon$ is infinite, every sent message is received.
    
    \item Let $e \in \epsilon$ be any event such that $e = \big( Q, \mathsf{receive}(m) \big)$ and let $t_r = \mathsf{time}(e, \mathcal{E})$.
    Moreover, let $e' = \big( P, \mathsf{send}(m) \big)$ be an event associated with $e$ ($e' \to e$; recall that $e' \in \epsilon$).
    Then, $\mathsf{max}\big( \mathsf{time}(e', \epsilon), \text{GST} \big) + \delta \geq t_r$.
    That is, the message delays must follow the properties of the partially synchronous model (see \Cref{section:preliminaries}).
    
    \item Let $T = \mathsf{time}(\epsilon[|\epsilon|], \mathcal{E})$ be the time at which the last event of $\epsilon$ occurs.
    For every event $e \in \epsilon$ such that (1) $e = \big( P, \mathsf{send}(m) \big)$, and (2) $\mathsf{max}\big( \mathsf{time}(e, \epsilon), \text{GST} \big) + \delta < T$, there exists an event $e' = \big( Q, \mathsf{receive}(m) \big)$ such that (1) $e' \in \epsilon$, and (2) $e \to e'$.
    That is, the message delays must follow the properties of the partially synchronous model (see \Cref{section:preliminaries}).
\end{compactenum}
We say that an execution $\mathcal{E} = (\mathcal{A}, c, \mathcal{F}, \epsilon, \text{GST})$ \emph{corresponds} to the input configuration $c$.
Recall that an execution $\mathcal{E} = (\mathcal{A}, c, \mathcal{F}, \epsilon, \text{GST})$ is canonical if and only if, for every event $e \in \epsilon$, $e$ does not occur on any process $Q \in \mathcal{F}$.
