# Supplementary material for: Partial Synchrony for Free? New Upper Bounds for Byzantine Agreement
Source: arXiv:2402.10059 source file (2024-10-23)
Supplement: Supplementary file 11 [file rebuilding_broadcast_long_values_new.tex]

\section{Rebuilding Broadcast} \label{section:rebuilding_broadccast}

In this section, we introduce rebuilding broadcast, a distributed primitive that plays a major role in our hash-based implementations of graded consensus and validation broadcast optimized for long values.
Concretely, this section introduces a hash-based asynchronous (tolerating unbounded message delays) implementation of the rebuilding broadcast primitive named \longreb.
\longreb is resilient to $t < n / 3$ Byzantine failures and it terminates in $O(1)$ asynchronous rounds while exchanging $O(nL + n^2 \kappa)$ bits, where $\kappa$ denotes the size of a hash value.

% our with $n/3$-resiliency, $O(1)$ asynchronous rounds, and $O(nL + n^2 \kappa)$ exchanged bits, where $\kappa$ denotes the size of a hash value.
%with different trade-offs (see \Cref{fig:rebuilding_broadcast_summary} below).

% \begin{table}[ht]
% \centering
% \begin{tabular}{ |p{2.4cm}|p{2.7cm}|p{1.3cm}|p{1.4cm}|p{2.1cm}|p{1.6cm}|  }
%  \hline
%  \centering Algorithm & \centering Exchanged bits & \centering Async. rounds & \centering Resilience & 
% \centering Cryptography \tabularnewline
%  \hline
%  \hline

% \centering \textbf{\textsc{RebLong3}} (\Cref{subsection:longreb_3})     & \centering $O(nL + n^2\log(n)\kappa)$ & \centering 2 & \centering $3t+1$ & \centering Hash  \tabularnewline

%  \hline

%  \centering \textbf{\textsc{RebLong4}} (\Cref{subsection:longreb_4})                 & \centering $O(nL + n^2\kappa)$ & \centering 2 & \centering $4t+1$ & \centering Hash \tabularnewline
%  \hline
% \end{tabular}
%     \caption{Relevant aspects of the two rebuilding broadcast algorithms we propose.
%     \\($L$ denotes the bit-size of a value, whereas $\kappa$ denotes the bit-size of a hash value.)}
% \label{fig:rebuilding_broadcast_summary}
% \end{table}

% First, we define the problem of rebuilding broadcast (\Cref{subsection:rebuilding_broadcast_problem_definition}).
% Then, we review existing primitives we employ in \longreb (\Cref{subsection:longreb_crypto_primitives}).
% Second, we present \longreb and prove its correctness and complexity (\Cref{subsection:longreb}).
%Lastly, we present \textsc{RebLong3} (\Cref{subsection:longreb_3}) and \textsc{RebLong4} (\Cref{subsection:longreb_4}).

\subsection{Problem Definition} \label{subsection:rebuilding_broadcast_problem_definition}

The rebuilding broadcast primitive allows each process to broadcast its input value and eventually deliver and rebuild some values.
% Let $\mathsf{Value}_{\mathit{reb}}$ denote the set of $L$-bit values that processes can broadcast, deliver and rebuild.
% For every value $\mathit{val} \in \mathsf{Value}_{\mathit{reb}}$, $\mathsf{valid}(\mathit{val})$ is a predetermined logical predicate that indicates whether or not $\mathit{val}$ is valid.
% Importantly, the goal of reducing broadcast is to reduce the number of different values delivered by correct processes to a constant.
The specification of the problem is associated with the default value $\bot_{\mathit{reb}} \notin \mathsf{Value}$.
Rebuilding broadcast exposes the following interface:
\begin{compactitem}
    \item \textbf{request} $\mathsf{broadcast}(v \in \mathsf{Value})$: a process broadcasts value $v$.

    % \item \textbf{request} $\mathsf{wish\_to\_abandon}$: a process wishes to abandon rebuilding broadcast.

    \item \textbf{request} $\mathsf{abandon}$: a process abandons rebuilding broadcast.

    \item \textbf{indication} $\mathsf{deliver}(v' \in \mathsf{Value} \cup \{\bot_{\mathit{reb}}\})$: a process delivers value $v'$ ($v'$ can be $\bot_{\mathit{reb}}$).

    \item \textbf{indication} $\mathsf{rebuild}(v' \in \mathsf{Value})$: a process rebuilds value $v'$ ($v'$ cannot be $\bot_{\mathit{reb}}$).
\end{compactitem}
Any correct process broadcasts at most once.
% and no correct process broadcasts an invalid value.
We do not assume that all correct processes broadcast.
% Moreover, any correct process invokes a $\mathsf{wish\_to\_abandon}$ request at most once.
% Importantly, we assume that any correct process invokes a $\mathsf{wish\_to\_abandon}$ request only if some correct process has previously delivered some value from rebuilding broadcast.

The rebuilding broadcast primitive requires the following properties to be satisfied.
\begin{compactitem}
    \item \emph{Strong validity:} If all correct processes that broadcast do so with the same value, then no correct process delivers $\bot_{\mathit{reb}}$.

    \item \emph{Safety:} If a correct process delivers a value \rebnotbottom{v'}, then a correct process has previously broadcast $v'$.

    \item \emph{Rebuilding validity:} Suppose all correct processes broadcast.
    If a correct process delivers a value \rebnotbottom{v'} at some time $\tau$ and no correct process abandons rebuilding broadcast by time $\tau' = \max(\tau, \text{GST}) + 2\delta$, then every correct process rebuilds $v'$ by time $\tau'$.

    \item \emph{Integrity:} A correct process delivers at most once and only if it has previously broadcast.

    \item \emph{Termination:} If all correct processes broadcast and no correct process abandons rebuilding broadcast, then every correct process eventually delivers.

    % \item \emph{Abandoning safety:} A correct process abandons rebuilding broadcast only if it has previously invoked a $\mathsf{wish\_to\_abandon}$ request.

    % \item \emph{Abandoning liveness:} If a correct process invokes a $\mathsf{wish\_to\_abandon}$ request at some time $\tau$, then the process abandons rebuilding broadcast by time $\max(\tau, \text{GST}) + \delta$.
\end{compactitem}
Note that a correct process can rebuild a value even if (1) it has not previously broadcast, or (2) it has previously abandoned rebuilding broadcast, or (3) it has previously delivered a value (or $\bot_{\mathit{reb}}$).
Moreover, multiple values can be rebuilt by a correct process.

\subsection{\longreb: Pseudocode} \label{subsection:longreb}

We present the pseudocode of \longreb in \Cref{algorithm:longreb}.
\longreb relies on the following three primitives:
\begin{compactitem}
    \item \emph{Collision-resistant hash function.}
    In \longreb, we utilize a cryptographic collision-resistant hash function $\mathsf{hash}(\cdot)$ that guarantees that a computationally bounded adversary cannot devise two inputs $i_1$ and $i_2$ such that $\mathsf{hash}(i_1) = \mathsf{hash}(i_2)$, except with a negligible probability.
    Each hash value is of size $\kappa$ bits; we assume $\kappa > \log(n)$.

    \item \emph{Graded consensus.}
    \longreb internally utilizes the graded consensus primitive; the specification of the primitive is given in \Cref{subsection:graded_consensus_building_blocks}.
    Concretely, \longreb is built on top of a specific implementation proposed in~\cite{AttiyaWelch23}; we refer to this implementation of graded consensus as ``AW graded consensus''.
    Importantly, processes in \longreb propose (and decide) hash values to the AW graded consensus algorithm.
    Given that the size of each hash value is $\kappa$ bits, correct processes send $O(n^2 \kappa)$ bits while executing the AW graded consensus algorithm.
    % in \longreb.

    \item \emph{Asynchronous data dissemination (ADD).}
    \longreb utilizes two instances of the asynchronous data dissemination (ADD) primitive; recall that the primitive is defined in \Cref{subsection:finisher}.
    In brief, ADD ensures that if at least $t + 1$ correct processes start with the same value, all correct processes eventually output that value.
    Correct processes exchange $O\big( nL + n^2 \log(n) \big)$ bits while executing ADD.
\end{compactitem}

%%%%%%%%%%%%%
%% RebLong %%
%%%%%%%%%%%%%
\begin{algorithm}
\caption{\textsc{RebLong}: Pseudocode (for process $p_i$)}
\label{algorithm:longreb}
\footnotesize
\begin{algorithmic} [1]

\State \textbf{Uses:}
\State \hskip2em Attiya-Welch graded consensus~\cite{AttiyaWelch23}, \textbf{instance} $\mathcal{AW}$ \BlueComment{hash values are proposed and decided}
\State \hskip2em Asynchronous data dissemination (ADD)~\cite{das2021asynchronous}, \textbf{instance} $\mathcal{ADD}_1$, $\mathcal{ADD}_2$

\medskip
\State \textbf{Local variables:}
\State \hskip2em $\mathsf{Value}$ $\mathit{broadcast\_value}_i \gets \bot$
\State \hskip2em $\mathsf{Hash\_Value}$ $\mathcal{H}_i \gets \bot$
\State \hskip2em $\mathsf{Hash\_Value}$ $\mathcal{H}_i^{*} \gets \bot$
\State \hskip2em $\mathsf{Value}$ $\mathit{output}_i \gets \bot$
\State \hskip2em $\mathsf{Boolean}$ $\mathit{delivered}_i \gets \mathit{false}$

\medskip
\State \textbf{upon} $\mathsf{broadcast}(v \in \mathsf{Value})$: \label{line:reblong_broadcast}
\State \hskip2em $\mathit{broadcast\_value}_i \gets v$ \label{line:reblong_update_broadcast_value}
\State \hskip2em $\mathcal{H}_i \gets \mathsf{hash}(v)$ \label{line:reblong_personal_hash}
% \State \hskip2em Let $[m_1, m_2, ..., m_n] \gets \mathsf{RSEnc}(\mathit{val}_i, n, t + 1)$\label{line:reblong3-enc}
% \State \hskip2em Let $\mathcal{H}_i \gets \mathsf{Eval}([m_1, m_2, ..., m_n])$\label{line:reblong3-eval}

\State \hskip2em \textbf{invoke} $\mathcal{AW}.\mathsf{propose}(\mathcal{H}_i)$ \label{line:reblong_graded_consensus_hash_propose_aw}

\medskip
\State \textbf{upon} $\mathcal{AW}.\mathsf{decide}(\mathcal{H} \in \mathsf{Hash\_Value}, g \in \{0, 1\})$ and $\mathcal{H}_i \neq \bot$: \label{line:reblong_graded_consensus_decide_aw}
\State \hskip2em  $\mathcal{H}_i^{*} \gets \mathcal{H}$ \label{line:reblong_common_hash}
\State \hskip2em \textbf{if} $\mathcal{H}_i^* = \mathcal{H}_i$ and $g = 1$: \label{line:reblong_happy_condition}
\State \hskip4em input $\mathit{broadcast\_value}_i$ to $\mathcal{ADD}_1$ \label{line:reblong_nonbot_ADD_1}
\State \hskip2em \textbf{else:} \label{line:reblong_sad_condition}
\State \hskip4em \textbf{broadcast} $\langle \mathsf{SAD} \rangle$ \label{line:reblong_broadcast_sad}

% \State \hskip2em \textbf{if} $\mathcal{H}^{*} \neq \mathcal{H}_i \vee g = 0$: \label{line:reblong_sad_condition}
% \State \hskip4em \textbf{broadcast} $\langle \textsc{sad} \rangle$ \label{line:reblong_broadcast_sad}
\State \hskip4em input $\bot$ to $\mathcal{ADD}_1$ \label{line:reblong_bot_ADD_1}
% \State \hskip2em \textbf{else}:

% \State \hskip4em \textbf{trigger} $\mathcal{ADD}_1.\mathsf{input}(\mathit{val}_i)$ \label{line:reblong_nonbot_ADD_1}

\medskip
\State \textbf{upon} $\langle \mathsf{SAD} \rangle$ is received from $t + 1$ processes and $\mathit{delivered}_i = \mathit{false}$: \label{line:reblong_check_deliver_bot}
\State \hskip2em $\mathit{delivered}_i \gets \mathit{true}$ \label{line:reblong_update_delivered_bot}
\State \hskip2em \textbf{trigger} $\mathsf{deliver}(\bot_{\mathit{reb}})$ \label{line:reblong_deliver_bot_rebuilding}

\medskip
\State \textbf{upon} $\mathcal{H}_i^{*} \neq \bot$ and $\mathsf{Value}$ $v'$ is output from $\mathcal{ADD}_1$ such that $\mathsf{hash}(v') = \mathcal{H}_i^*$: \label{line:reblong_output_ADD_1}

\State \hskip2em input $v'$ to $\mathcal{ADD}_2$\label{line:reblong_nonbot_ADD_2}

\State \hskip2em $\mathit{output}_i \gets v'$ \label{line:reblong_update_output}

\State \hskip2em \textbf{broadcast} $\langle \mathsf{HAPPY}, \mathcal{H}_i^{*} \rangle$ \label{line:reblong_broadcast_happy}
% \State \hskip2em \textbf{trigger} $\mathsf{rebuild}(v')$ \label{line:reblong_rebuilding_1}

\medskip
\State \textbf{upon} $\mathcal{H}_i^{*} \neq \bot$ and $\mathsf{Value}$ $v'$ is output from $\mathcal{ADD}_2$ such that $\mathsf{hash}(v') = \mathcal{H}_i^*$: \label{line:reblong_output_ADD_2}

\State \hskip2em \textbf{trigger} $\mathsf{rebuild}(v')$ \label{line:reblong_rebuilding_2}

\medskip
\State \textbf{upon} $\mathit{output}_i \neq \bot$ and $\langle \mathsf{HAPPY}, \mathcal{H}_i^* \rangle$ is received from $2t + 1$ processes and $\mathit{delivered}_i = \mathit{false}$: \label{line:reblong_check_deliver_nonbot}
\State \hskip2em $\mathit{delivered}_i \gets \mathit{true}$ \label{line:reblong_update_delivered_nonbot}
\State \hskip2em \textbf{trigger} $\mathsf{deliver}( \mathit{output}_i)$ \label{line:reblong_nonbot_deliver}

% \medskip 
% \State \textbf{upon} $\mathsf{wish\_to\_abandon}$: \label{line:reblong_wish_to_abandon}
% \State \hskip2em \textbf{wait for} the completion of $\mathcal{ADD}_2$ \BlueComment{wait for $t + 1$ \textsc{disperse} message, and then broadcast a \textsc{reconstruct} message} \label{line:reblong_complete_add_2}
% \State \hskip2em \textbf{trigger} $\mathsf{abandon}$ \label{line:reblong_trigger_abandon}

\end{algorithmic} 
\end{algorithm}

We describe \longreb from the perspective of a correct process $p_i$.
When $p_i$ broadcasts its value $\mathit{broadcast\_value}_i$ (line~\ref{line:reblong_broadcast}), it proposes the hash of the value to the AW graded consensus algorithm (line~\ref{line:reblong_graded_consensus_hash_propose_aw}).
Once $p_i$ decides some pair $(\mathcal{H}, g)$ from the AW graded consensus algorithm, $p_i$ checks if (1) $\mathcal{H}$ is the hash value of $p_i$'s broadcast value $\mathit{broadcast\_value}_i$, and (2) the grade $g$ is $1$ (line~\ref{line:reblong_happy_condition}).
If this check passes, process $p_i$ inputs its value $\mathit{broadcast\_value}_i$ to the first instance $\mathcal{ADD}_1$ of the ADD primitive (line~\ref{line:reblong_nonbot_ADD_1}).
If the check does not pass, process $p_i$ knows that not all correct processes have broadcast the same value, thus allowing processes to deliver $\bot_{\mathit{reb}}$.
Hence, $p_i$ broadcasts a $\langle \mathsf{SAD} \rangle$ message (line~\ref{line:reblong_broadcast_sad}) and inputs $\bot$ to $\mathcal{ADD}_1$ (line~\ref{line:reblong_bot_ADD_1}).
If $p_i$ receives a $\langle \mathsf{SAD} \rangle$ message from $t + 1$ processes (line~\ref{line:reblong_check_deliver_bot}), $p_i$ delivers $\bot_{\mathit{reb}}$ (line~\ref{line:reblong_deliver_bot_rebuilding}) as it knows that at least one correct process has previously broadcast a $\langle \mathsf{SAD} \rangle$ message.
Once process $p_i$ outputs a value $v'$ whose hash $\mathcal{H} = \mathsf{hash}(v')$ it has previously decided from the AW graded consensus algorithm (line~\ref{line:reblong_output_ADD_1}), $p_i$ executes the following steps: (1) $p_i$ inputs $v'$ to the second instance $\mathcal{ADD}_2$ of the ADD primitive (line~\ref{line:reblong_nonbot_ADD_2}), and (2) $p_i$ broadcasts a $\langle \mathsf{HAPPY}, \mathcal{H} \rangle$ message (line~\ref{line:reblong_broadcast_happy}) notifying all processes that it has input a value to $\mathcal{ADD}_2$.
Once $p_i$ outputs a value from $\mathcal{ADD}_2$ whose hash value it has decided from the AW graded consensus algorithm (line~\ref{line:reblong_output_ADD_2}), $p_i$ rebuilds that value (line~\ref{line:reblong_rebuilding_2}).
Finally, when $p_i$ receives $2t + 1$ $\langle \mathsf{HAPPY}, \mathcal{H} \rangle$ messages (line~\ref{line:reblong_check_deliver_nonbot}), where $\mathcal{H}$ is the hash value of the value $v'$ previously output by $\mathcal{ADD}_1$ (and input to $\mathcal{ADD}_2$), $p_i$ delivers $v'$ (line~\ref{line:reblong_nonbot_deliver}).
Observe that, in this case, $p_i$ knows that at least $t + 1$ correct processes have input $v'$ to $\mathcal{ADD}_2$, thus ensuring that all correct processes eventually rebuild $v'$.

%%%%%%%%%%%%%%%%%%%
%% RebLong (end) %%
%%%%%%%%%%%%%%%%%%%

\subsection{\longreb: Proof of Correctness \& Complexity}

\paragraph{Proof of correctness.}
We start by showing that strong validity is satisfied. 

\begin{theorem} [Strong validity] \label{theorem:long_reb_strong_validity_3}
\longreb (\Cref{algorithm:longreb}) satisfies strong validity.
\end{theorem}
\begin{proof}
Assume all correct processes that broadcast (line~\ref{line:reblong_broadcast}) do so with the same value $v$; let $\mathcal{H} = \mathsf{hash}(v)$.
When all these correct processes propose $\mathcal{H}$ to $\mathcal{AW}$ (line~\ref{line:reblong_graded_consensus_hash_propose_aw}).
Due to the strong validity property of $\mathcal{AW}$, each correct process that decides from $\mathcal{AW}$ (line~\ref{line:reblong_graded_consensus_decide_aw}) does decide $(\mathcal{H}, 1)$.
% in $\mathcal{AW}$ at line~\ref{line:reblong_graded_consensus_decide_aw} does so with the pair $(\mathcal{H}, g=1)$.
Therefore, the condition at line~\ref{line:reblong_sad_condition} is never activated at a correct process, which implies that no correct process ever sends a $\langle \mathsf{SAD} \rangle$ message (line~\ref{line:reblong_broadcast_sad}).
Thus, the rule at line~\ref{line:reblong_check_deliver_bot} never activates at any correct process, which concludes the proof.
\end{proof}

Next, we prove the safety property.

\begin{theorem} [Safety]
\longreb (\Cref{algorithm:longreb}) satisfies safety.
\end{theorem}
\begin{proof}
Suppose a correct process $p_i$ delivers a value $v' \neq \bot_{\mathit{reb}}$ (line~\ref{line:reblong_nonbot_deliver}).
Hence, process $p_i$ must have previously received a $\langle \mathsf{HAPPY}, \mathcal{H}_i^* \rangle$ message from $2t + 1$ processes (line~\ref{line:reblong_check_deliver_nonbot}), where $\mathcal{H}_i^* = \mathsf{hash}(v')$ (see line~\ref{line:reblong_update_output}).
Let $p_j$ be any correct process that has sent a $\langle \mathsf{HAPPY}, \mathcal{H}_i^* \rangle$ message.
Note that $p_j$ does so at line~\ref{line:reblong_broadcast_happy} upon outputting value $v'$ from $\mathcal{ADD}_1$ (line~\ref{line:reblong_output_ADD_1}).
(Recall that $\mathsf{hash}(\cdot)$ is collission-resistant.)
Due to the properties of $\mathcal{ADD}_1$, there exists a correct process $p_s$ that has previously input $v'$ to $\mathcal{ADD}_1$ (line~\ref{line:reblong_nonbot_ADD_1}), which means that $v'$ is the value broadcast by $p_s$ (due to the assignment at line~\ref{line:reblong_update_broadcast_value}).
Therefore, the safety property is satisfied.
\end{proof}

The following theorem proves rebuilding validity.

\begin{theorem} [Rebuilding validity] \label{theorem:rebuilding_validity}
\longreb (\Cref{algorithm:longreb}) satisfies rebuilding validity.
\end{theorem} 

\begin{proof}
Assume any correct process $p_j$ delivers a value $\mathit{val}$ at line~\ref{line:reblong_nonbot_deliver} at time $\tau$. Consequently, based on the verification at line~\ref{line:reblong_check_deliver_nonbot}, line~\ref{line:reblong_output_ADD_1} and line~\ref{line:reblong_update_output}, $p_j$ must have received $2t + 1$ $\langle \textsc{happy}, \mathcal{H} \rangle$ messages, where $\mathsf{hash}(\mathit{val}) = \mathcal{H}$, and $\mathcal{AW}.\mathsf{decide}(\mathcal{H}, \cdot)$ has been triggered at line~\ref{line:reblong_graded_consensus_decide_aw}. This implies that $t+1$ $\langle \textsc{happy}, \mathcal{H} \rangle$ messages were broadcast by an equal number of correct processes at line~\ref{line:reblong_broadcast_happy}, indicating these correct processes triggered $\mathcal{ADD}_1.\mathsf{output}$ following the condition at line~\ref{line:reblong_output_ADD_1}.

Therefore, according to $\mathcal{ADD}_1$'s correctness, at least one correct process must have triggered (at line~\ref{line:reblong_nonbot_ADD_1}) $\mathcal{ADD}_1.\mathsf{input}(\mathit{val}_{\mathit{in}}^{1} \neq \bot)$, after triggering $\mathcal{AW}.\mathsf{decide}(\mathcal{H}', 1)$, with $\mathsf{hash}(\mathit{val}_{\mathit{in}}^{1}) = \mathcal{H}'$, as per the condition at line~\ref{line:reblong_happy_condition}. Given $\mathcal{AW}$'s consistency, every correct process that initiated $\mathcal{AW}.\mathsf{decide}(\mathcal{H}'', \cdot)$ at line~\ref{line:reblong_graded_consensus_decide_aw}, did so with $\mathcal{H}'' = \mathcal{H}' = \mathcal{H}$. The hash function's collision-resistance implies that every correct process triggering $\mathcal{ADD}_1.\mathsf{input}(\mathit{val}'' \neq \bot)$ at line~\ref{line:reblong_nonbot_ADD_1} did so with $\mathit{val}'' = \mathit{val}_{\mathit{in}}^{1} = \mathit{val}$. Thus, by $\mathcal{ADD}_1$'s correctness, every correct process that triggered $\mathcal{ADD}_1.\mathsf{output}(\mathit{val}_{\mathit{out}}^{1})$ at line~\ref{line:reblong_output_ADD_1} did so with $\mathit{val}_{\mathit{out}}^{1} = \mathit{val}$.

Therefore, every correct process that triggers $\mathcal{ADD}_2.\mathsf{input}(\mathit{val}_{\mathit{in}}^{2} \neq \bot)$ at line~\ref{line:reblong_nonbot_ADD_2} does so with $\mathit{val}_{\mathit{in}}^{2} = \mathit{val}$. Moreover, these correct processes number at least $t+1$ since $p_j$ received (at time $\tau$) $2t + 1$ $\langle \textsc{happy}, \mathcal{H} \rangle$ messages. By the correctness of $\mathcal{ADD}_2$, every correct process eventually triggers $\mathcal{ADD}_2.\mathsf{output}(\mathit{val})$ at line~\ref{line:reblong_output_ADD_2} and thus eventually triggers $\mathsf{rebuild}(\mathit{val})$ at line~\ref{line:reblong_rebuilding_2}. This occurs by time $\max(\tau, \text{GST}) + 2\delta$, given that $\mathcal{ADD}_2$ requires $2$ asynchronous rounds.
\end{proof}

We continue our proof by showing that \textsc{RebLong} satisfies integrity.

\begin{theorem} [Integrity]
\longreb (\Cref{algorithm:longreb}) satisfies integrity.
\end{theorem}
\begin{proof}
Follows directly from \Cref{algorithm:longreb} (namely the checks lines \ref{line:reblong_check_deliver_bot} and \ref{line:reblong_check_deliver_nonbot} and the corresponding updates lines \ref{line:reblong_update_delivered_bot} and \ref{line:reblong_update_delivered_nonbot}).
\end{proof}

Lastly, we prove \textsc{RebLong}'s termination.

\begin{theorem} [Termination] \label{theorem:termination_longreb_3t}
\textsc{RebLong} satisfies termination.
\end{theorem}
\begin{proof}
By termination property of $\mathcal{AW}$, every correct process eventually triggers $\mathcal{AW}.\mathsf{decide}(\mathcal{H}'_i, g_i)$ line~\ref{line:reblong_graded_consensus_decide_aw}. 
Consequently, due to the check line~\ref{line:reblong_happy_condition}, every correct process either (1) broadcasts a $\textsc{sad}$ message line~\ref{line:reblong_broadcast_sad} and triggers $\mathcal{ADD}.\mathsf{input}(\bot)$ line~\ref{line:reblong_bot_ADD_1} or (2) or triggers $\mathcal{ADD}.\mathsf{input}(\mathit{val}_i \neq \bot)$ line~\ref{line:reblong_nonbot_ADD_1}.
To prove termination, we consider two cases:
\begin{compactitem}
    \item Suppose that at least $t + 1$ correct processes broadcast a $\textsc{sad}$ message line~\ref{line:reblong_broadcast_sad}. Then, every correct process eventually receives $t+1$ $\textsc{sad}$ messages line~\ref{line:reblong_check_deliver_bot}, and then delivers $\bot$ line~\ref{line:reblong_deliver_bot_rebuilding} if it did not deliver yet.
    
    \item Suppose that strictly less than $t + 1$ correct processes send a $\textsc{sad}$ message line~\ref{line:reblong_broadcast_sad}. This means there exist a set $S$ of at least $t+1$ correct processes, such that for every correct process $p_i$ in $S$, $p_i$ has triggered $\mathcal{AW}.\mathsf{output}(\mathcal{H}_i, 1)$ line~\ref{line:reblong_graded_consensus_decide_aw} with $\mathcal{H}_i = \mathsf{hash}(\mathit{val}_i)$.
    By consistency of $\mathcal{AW}$, there exist a hash value $\mathcal{H}_S$, such that no correct process triggered $\mathcal{AW}.\mathsf{decide}(\mathcal{H}', \cdot)$ line~\ref{line:reblong_graded_consensus_decide_aw} with $\mathcal{H}' \neq \mathcal{H}_S$.
    Hence, every check of the form $\mathsf{hash}(\mathit{val}') = \mathcal{H}^{*}$ with $ \mathsf{hash}(\mathit{val}') = \mathcal{H}_S$ (line~\ref{line:reblong_output_ADD_1} and line~\ref{line:reblong_check_deliver_nonbot}) passes.
    Moreover, every correct process $p_i$ that triggered $\mathcal{ADD}_1.\mathsf{input}(\mathit{val}_i \neq \bot)$ line~\ref{line:reblong_nonbot_ADD_1}, did so with $\mathsf{hash}(\mathit{val}_i) = \mathcal{H}_S$.
    By collision-resistance of the hash function, every correct process $p_i$ that triggered $\mathcal{ADD}_1.\mathsf{input}(\mathit{val}_i \neq \bot)$ line~\ref{line:reblong_nonbot_ADD_1}, did so with $\mathit{val}_i = \mathit{val}_S$ for some common value $\mathit{val}_S$, such that $\mathsf{hash}(\mathit{val}_S) = \mathcal{H}_S$.
    By correctness of $\mathcal{ADD}_1$, every correct process eventually triggers $\mathcal{ADD}_1.\mathsf{output}(\mathit{val}_S)$ line~\ref{line:reblong_output_ADD_1}. Thus every correct process $p_i$ eventually update its variable $\mathit{output}_i$ to $\mathit{val}_S$ line~\ref{line:reblong_update_output}
    %triggers $\mathcal{ADD}_2.\mathsf{input}(\mathit{val}_S)$ line~\ref{line:reblong_nonbot_ADD_2} 
    and broadcasts $\langle \textsc{happy}, \mathcal{H}_S \rangle$ line~\ref{line:reblong_broadcast_happy}.
    %By correctness of $\mathcal{ADD}_2$, every correct process eventually triggers $\mathcal{ADD}_2.\mathsf{output}(\mathit{val}_S)$ line~\ref{line:reblong_output_ADD_2}. 
    Finally, every correct process eventually receives $2t+1$ $\langle \textsc{happy}, \mathcal{H}_S \rangle$ messages line~\ref{line:reblong_output_ADD_2} and thus triggers $\mathsf{deliver}(\mathit{val}_S)$ line~\ref{line:reblong_nonbot_deliver} if it did not deliver yet.
\end{compactitem}
As termination is ensured in any of the two possible scenarios, the proof is concluded.
\end{proof}

Therefore, \textsc{RebLong} is indeed correct.

\begin{corollary}
\textsc{RebLong} is correct.
\end{corollary}

\paragraph{Proof of complexity.}
% We start by proving that any correct process broadcasts at most two different \textsc{echo} messages.

% \begin{lemma} \label{lemma:two_echo}
% Any correct process broadcasts at most two different \textsc{echo} messages.
% \end{lemma}
% \begin{proof}
% Any correct process $p_i$ can receive $t + 1$ identical \textsc{init} messages for at most two values as $3t + 1 - 2(t + 1) < t + 1$.
% Recall that $p_i$ only ``accepts'' one \textsc{init} message per process (line~\ref{line:one_init_accept}).
% \end{proof}

The following theorem proves that no correct process sends more than $O(\kappa n + L)$ bits. % correct processes exchange $O(nL + n^2\log(n)\kappa)$ bits

\begin{theorem} [Exchanged bits]
A correct process sends less than $O(L + \kappa n)$ bits in \textsc{RebLong}.
%Correct processes send $O(nL + n^2\log(n)\kappa)$ bits in \textsc{RebLong}.
\end{theorem}
\begin{proof}
The per-process communication complexity of $\mathcal{AW}$ is $O(\kappa n)$, while the per-process communication complexity of $\mathcal{ADD}$ is $O(L + n\log(n))$.
Finally a correct process can broadcast either a $\textsc{sad}$ message of $O(1)$ bits (line~\ref{line:reblong_broadcast_sad}) or an $\textsc{happy}$ message of $O(\kappa)$ bits (line~\ref{line:reblong_broadcast_happy}).
Thus, every correct process sends less than $O(L + \kappa n)$ bits in \textsc{RebLong}.
\end{proof}

Finally, the following theorem proves that \textsc{RebLong} incurs $O(1)$ asynchronous rounds.

\begin{theorem} [Asynchronous rounds] \label{theorem:async_rounds_rebuilding_3}
Assuming that all correct processes broadcast via \textsc{RebLong} and no correct process abandons \textsc{RebLong}, \textsc{RebLong} incurs $O(1)$ asynchronous rounds. More precisely, \textsc{RebLong}, \textsc{RebLong} incurs $12$ asynchronous rounds before delivery, and $2$ asynchronous rounds between the first delivery and the corresponding rebuilding.
\end{theorem}
\begin{proof}
The $\mathcal{AW}$ instance incurs $9 \in O(1)$ asynchronous rounds, while each instance of ADD incurs $2 \in O(1)$ asynchronous rounds.

More precisely, similarly to the proof of the termination property (\Cref{theorem:termination_longreb_3t}), there are two distinct scenarios to analyze after processes triggered $\mathcal{AW}.\mathsf{decide}$:
either (1) at least $t+1$ correct processes broadcast a $\textsc{sad}$ message line~\ref{line:reblong_broadcast_sad} and triggers $\mathcal{ADD}.\mathsf{input}(\bot)$ line~\ref{line:reblong_bot_ADD_1} or (2) at least $t+1$ correct processes triggers $\mathcal{ADD}.\mathsf{input}(\mathit{val}_i \neq \bot)$ line~\ref{line:reblong_nonbot_ADD_1}.
\begin{compactitem}
    \item Suppose that at least $t + 1$ correct processes broadcast a $\textsc{sad}$ message line~\ref{line:reblong_broadcast_sad}. Then, every correct process eventually receives $t+1$ $\textsc{sad}$ messages line~\ref{line:reblong_check_deliver_bot} within one round, and then delivers $\bot$ line~\ref{line:reblong_deliver_bot_rebuilding} if it did not deliver yet.
    In this case, $\mathsf{deliver}$ is triggered after $9+1 = 10$ asynchronous rounds.
    \item Suppose that at least $t + 1$ correct processes triggers $\mathcal{ADD}.\mathsf{input}(\mathit{val} \neq \bot)$ line~\ref{line:reblong_nonbot_ADD_1}. 
    In this case, every correct process triggers $\mathcal{ADD}.\mathsf{output}(\mathit{val} \neq \bot)$ line~\ref{line:reblong_output_ADD_1} and then broadcast line~\ref{line:reblong_broadcast_happy} a corresponding $\textsc{happy}$ message after $9+2 = 11$ asynchronous rounds.
    Thus, the event line~\ref{line:reblong_check_deliver_nonbot} passes after 1 additional round, where $\mathsf{deliver}$ is triggered line~\ref{line:reblong_nonbot_deliver} by every correct process after $9+2+1 = 12$ asynchronous rounds.

 \end{compactitem}

Finally, the proof of the Rebuilding Validity (see Theorem~\ref{theorem:rebuilding_validity}), allows to conclude.  
\end{proof} 
