# Supplementary material for: Partial Synchrony for Free? New Upper Bounds for Byzantine Agreement
Source: arXiv:2402.10059 source file (2024-10-23)
Supplement: Supplementary file 12 [file repeater_proof.tex]

\section{\name: Proof of Correctness \& Complexity}

This section provides a formal proof of \name's correctness and message complexity.

\subsection{Preliminaries}

Following the formalism introduced in~\cite{civit2022byzantine}, we define the behaviors and timer histories of processes.
A \emph{behavior} of a process $p_i$ is a sequence of (1) message-sending events performed by $p_i$, (2) message-reception events performed by $p_i$, and (3) internal events performed by $p_i$ (e.g., invoking $\mathsf{measure}(\cdot)$ or $\mathsf{cancel()}$ methods on the local timers).
A \emph{timer history} of a process $p_i$ is a sequence of (1) invocations of the $\mathsf{measure}(\cdot)$ and $\mathsf{cancel}()$ methods on $\mathit{help\_timer}_i$ and $\mathit{enter\_timer}_i$, and (2) processed expiration events of $\mathit{help\_timer}_i$ and $\mathit{enter\_timer}_i$.
Observe that a timer history of a process is a subsequence of the behavior of the process.
If an event $e$ belongs to a sequence of events $\mathcal{S}$, we write $e \in \mathcal{S}$; otherwise, we write $e \notin \mathcal{S}$.
If an event $e_1$ precedes an event $e_2$ in a sequence $\mathcal{S}$, we write $e_1 \stackrel{\mathcal{S}}{\prec} e_2$.
% Note that, if $e_1 \stackrel{\beta_i}{\prec} e_2$ and $e_1$ occurs at some time $t_1$ and $e_2$ occurs at some time $t_2$, $t_1 \leq t_2$.

We denote by $h_i|_{\mathit{enter}}$ (resp., $h_i|_{\mathit{help}}$) a subsequence of $h_i$ associated with the $\mathit{enter\_timer}_i$ (resp., $\mathit{help\_timer}_i$) timer, where $h_i$ is a timer history of process $p_i$.
If an expiration event $\mathit{Exp}$ of a timer is associated with an invocation $\mathit{Inv}$ of the $\mathsf{measure(\cdot)}$ method on the timer, we say that $\mathit{Inv}$ \emph{produces} $\mathit{Exp}$.
Note that a single invocation of the $\mathsf{measure}(\cdot)$ method produces at most one expiration event.
Moreover, any expiration event is produced by exactly one invocation of the $\mathsf{measure}(\cdot)$ method.

% Given an execution, we denote by $\beta_i$ and $h_i$ the behavior and the timer history of the process $p_i$, respectively.

\subsection{Proof of Correctness}

To prove the correctness of \name, we need to prove that \name satisfies the validity, agreement, and termination properties.
We start by showing that, for any correct process $p_i$, any expiration event of $\mathit{enter\_timer}_i$ immediately follows in $h_i|_{\mathit{enter}}$ the invocation that produces it, where $h_i$ is the timer history of $p_i$.

\begin{lemma} \label{lemma:enter_invocation_expiration}
% Let $\mathcal{E}$ be any execution of \name.
Let $p_i$ be any correct process, and let $h_i$ be $p_i$'s timer history.
Let $\mathit{Exp}_e$ be any expiration event of $\mathit{enter\_timer}_i$ that belongs to $h_i$, and let $\mathit{Inv}_e$ be the invocation of the $\mathsf{measure}(\cdot)$ method (on $\mathit{enter\_timer}_i$) that produces $\mathit{Exp}_e$.
Then, $\mathit{Exp}_e$ immediately follows $\mathit{Inv}_e$ in $h_i|_{\mathit{enter}}$.
\end{lemma}
\begin{proof}
By contradiction, suppose that $\mathit{Exp}_e$ does not immediately follow $\mathit{Inv}_e$ in $h_i|_{\mathit{enter}}$.
We consider all possibilities:
\begin{compactitem}
    \item Let an invocation $\mathit{Inv}_e'$ of the $\mathsf{measure}(\cdot)$ method immediately follow $\mathit{Inv}_e$ in $h_i|_{\mathit{enter}}$:
    Invocation $\mathit{Inv}_e'$ could have only been invoked at line~\ref{line:measure_enter}.
    However, it is immediately preceded by an invocation of the $\mathsf{cancel}()$ method (line~\ref{line:cancel_enter}) in $h_i|_{\mathit{enter}}$.
    Therefore, this case is impossible.

    \item Let an invocation $\mathit{Inv}_e'$ of the $\mathsf{cancel}()$ method immediately follow $\mathit{Inv}_e$ in $h_i|_{\mathit{enter}}$:
    This case is impossible as $\mathit{Inv}_e$ does produce $\mathit{Exp}_e$.

    \item Let an expiration event $\mathit{Exp}_e' \neq \mathit{Exp}_e$ immediately follow $\mathit{Inv}_e$ in $h_i|_{\mathit{enter}}$:
    As $\mathit{Inv}_e$ could have only been invoked at line~\ref{line:measure_enter}, it is immediately preceded by an invocation of the $\mathsf{cancel}()$ method (line~\ref{line:cancel_enter}).
    Hence, it is impossible for $\mathit{Exp}_e'$ to be produced, which renders this case impossible as well.
\end{compactitem}
As neither of the three other possibilities can occur, $\mathit{Exp}_e$ indeed immediately follows $\mathit{Inv}_e$ in $h_i|_{\mathit{enter}}$.
\end{proof}

The next lemma proves that, for any correct process $p_i$, any expiration event of $\mathit{help\_timer}_i$ immediately follows in $h_i|_{\mathit{help}}$ the invocation that produces it, where $h_i$ is the timer history of $p_i$. 

\begin{lemma} \label{lemma:help_invocation_expiration}
% Let $\mathcal{E}$ be any execution of \name.
Let $p_i$ be any correct process, and let $h_i$ be $p_i$'s timer history.
% in $\mathcal{E}$.
Let $\mathit{Exp}_h$ be any expiration event of $\mathit{help\_timer}_i$ that belongs to $h_i$, and let $\mathit{Inv}_h$ be the invocation of the $\mathsf{measure}(\cdot)$ method (on $\mathit{help\_timer}_i$) that produces $\mathit{Exp}_h$.
Then, $\mathit{Exp}_h$ immediately follows $\mathit{Inv}_h$ in $h_i|_{\mathit{help}}$.
\end{lemma}
\begin{proof}
By contradiction, let us assume that $\mathit{Exp}_h$ does not immediately follow $\mathit{Inv}_h$ in $h_i|_{\mathit{help}}$.
We consider all possibilities:
\begin{compactitem}
    \item Let an invocation $\mathit{Inv}_h'$ of the $\mathsf{measure}(\cdot)$ method immediately follow $\mathit{Inv}_h$ in $h_i|_{\mathit{help}}$:
    Invocation $\mathit{Inv}_h'$ could have only been invoked at line~\ref{line:measure_help}.
    However, it is immediately preceded by an invocation of the $\mathsf{cancel}()$ method (line~\ref{line:cancel_help}) in $h_i|_{\mathit{help}}$, thus rendering this case impossible.

    \item Let an invocation $\mathit{Inv}_h'$ of the $\mathsf{cancel}()$ method immediately follow $\mathit{Inv}_h$ in $h_i|_{\mathit{help}}$:
    This case cannot happen as $\mathit{Inv}_h$ produces $\mathit{Exp}_h$.

    \item Let an expiration event $\mathit{Exp}_h' \neq \mathit{Exp}_h$ immediately follow $\mathit{Inv}_h$ in $h_i|_{\mathit{help}}$:
    As $\mathit{Inv}_h$ could have only been invoked at line~\ref{line:measure_help}, it is immediately preceded by an invocation of the $\mathsf{cancel}()$ method (line~\ref{line:cancel_help}).
    Hence, $\mathit{Exp}_h'$ cannot be produced, which makes this case impossible.
\end{compactitem}
As neither of the three other possibilities can occur, $\mathit{Exp}_h$ immediately follows $\mathit{Inv}_h$ in $h_i|_{\mathit{help}}$.
\end{proof}

Next, we show that the value of the $\mathit{view}_i$ variable of any correct process $p_i$ cannot decrease throughout an execution.

\begin{lemma} \label{lemma:view_i_increases}
% Let $\mathcal{E}$ be any execution of \name.
Let $p_i$ be any correct process.
% correct in $\mathcal{E}$.
Let the value of the $\mathit{view}_i$ variable be $v_1$ at some point, and let the value of the $\mathit{view}_i$ variable be $v_2$ at some later point.
Then, $v_1 \leq v_2$.
\end{lemma}
\begin{proof}
The only place at which $p_i$ updates its $\mathit{view}_i$ variable is line~\ref{line:update_view_2}.
Hence, the check at line~\ref{line:receive_quorum} ensures that $p_i$ only updates the $\mathit{view}_i$ variable to a value greater than the one previously held, which implies that the lemma holds.
\end{proof}

The following lemma proves that the value of the $\mathit{help\_view}_i$ variable of any correct process $p_i$ cannot decrease.

\begin{lemma} \label{lemma:help_view_i_increases}
Let $p_i$ be any correct process.
% in $\mathcal{E}$.
Let the value of the $\mathit{help\_view}_i$ variable be $v_1$ at some point, and let the value of the $\mathit{help\_view}_i$ variable be $v_2$ at some later point.
Then, $v_1 \leq v_2$.
\end{lemma}
\begin{proof}
The only place at which $p_i$ updates the $\mathit{help\_view}_i$ variable is line~\ref{line:update_help_view}.
Thus, the check at line~\ref{line:check_help} guarantees that $p_i$ updates $\mathit{help\_view}_i$ to a value greater than the one previously held, which concludes the proof.
\end{proof}

We now prove that correct processes send \textsc{start-view} messages only for views greater than $1$.

\begin{lemma} \label{lemma:start_view_for_1}
If a correct process sends a $\langle \textsc{start-view}, v \rangle$ message, then $v \geq 2$.
\end{lemma}
\begin{proof}
Consider any correct process $p_i$.
Throughout the entire execution, the value of the $\mathit{view}_i$ variable is equal to or greater than $1$ as (1) the initial value of $\mathit{view}_i$ is $1$ (line~\ref{line:init_view}), and (2) the value of $\mathit{view}_i$ cannot decrease (by \Cref{lemma:view_i_increases}).
Similarly, the value of the $\mathit{help\_view}_i$ variable is, at all times, equal to or greater than $1$ as (1) the initial value of $\mathit{help\_view}_i$ is $1$ (line~\ref{line:init_help_view}), and (2) the value of $\mathit{help\_view}_i$ cannot decrease (by \Cref{lemma:help_view_i_increases}).
Therefore, $v \geq 1$.

It is left to prove that $v \neq 1$.
By contradiction, suppose that $v = 1$.
We consider all places at which $p_i$ could have sent a $\langle \textsc{start-view}, v = 1 \rangle$ message:
\begin{compactitem}
    \item line~\ref{line:send_complete_1}: As the value of the $\mathit{view}_i$ variable is equal to or greater than $1$, $p_i$ could not have sent the $\langle \textsc{start-view}, 1 \rangle$ message here (as $\mathit{view}_i + 1 \geq 2$).

    \item line~\ref{line:send_complete_2}: Let $\mathit{Inv}_h$ denote the invocation of the $\mathsf{measure}(\cdot)$ method on $\mathit{help\_timer}_i$ that produces the expiration event processed at line~\ref{line:help_timer_expires}.
    Process $p_i$ must have invoked $\mathit{Inv}_h$ at line~\ref{line:measure_help}.
    At the moment of invoking $\mathit{Inv}_h$, the value of the $\mathit{help\_view}_i$ variable is greater than $1$ due to (1) the fact that the value of $\mathit{help\_view}_i$ is always equal to or greater than $1$, (2) the check at line~\ref{line:check_help}, and (3) the assignment at line~\ref{line:update_help_view}. 
    As the value of $\mathit{help\_view}_i$ only increases throughout the entire execution, $p_i$ could not have sent a $\langle \textsc{start-view}, 1 \rangle$ message at line~\ref{line:send_complete_2}.

    \item line~\ref{line:send_complete_2_prime}: Process $p_i$ could not have sent a $\langle \textsc{start-view}, 1 \rangle$ message here due to the check at line~\ref{line:check_help_2}.

    \item line~\ref{line:send_complete_3}: Let $\mathit{Inv}_e$ denote the invocation of the $\mathsf{measure}(\cdot)$ method on $\mathit{enter\_timer}_i$ that produces the expiration event processed at line~\ref{line:enter_expires}.
    Process $p_i$ must have invoked $\mathit{Inv}_e$ at line~\ref{line:measure_enter}.
    At the moment of invoking $\mathit{Inv}_e$, the value of the $\mathit{view}_i$ variable is greater than $1$ due to (1) the fact that the value of $\mathit{view}_i$ is always equal to or greater than $1$, (2) the check at line~\ref{line:receive_quorum}, and (3) the assignment at line~\ref{line:update_view_2}. 
    As the value of $\mathit{view}_i$ only increases throughout the entire execution, $p_i$ could not have sent a $\langle \textsc{start-view}, 1 \rangle$ message at line~\ref{line:send_complete_3}.

    \item line~\ref{line:send_complete_3_prime}: Process $p_i$ could not have sent a $\langle \textsc{start-view}, 1 \rangle$ message here due to the check at line~\ref{line:check_view}.
\end{compactitem}
Hence, we reach a contradiction with the fact that $p_i$ sends a $\langle \textsc{start-view}, 1 \rangle$ message, which concludes the proof.
\end{proof}

The following lemma proves that it is impossible for correct processes to send $\langle \textsc{start-view}, v \rangle$ and $\langle \textsc{start-view}, v + 2 \rangle$, for some view $v \geq 2$, without sending a $\langle \textsc{start-view}, v + 1 \rangle$ message.

\begin{lemma} \label{lemma:no_gaps}
Consider any execution $\mathcal{E}$ of \name in which at least one $\textsc{start-view}$ message is sent by correct processes.
Let $\mathcal{V}(\mathcal{E}) = \{ v \in \mathsf{View} \,|\, \langle \textsc{start-view}, v \rangle \text{ is sent by a correct process in } \mathcal{E} \}$.
Let $v^*$ be the greatest view of $\mathcal{V}(\mathcal{E})$.
% such that (1) $v_{\mathit{max}} \in \mathcal{V}_{\mathcal{E}}$, and (2) $v_{\mathit{max}} \geq v'$, for every view $v' \in \mathcal{V}_{\mathcal{E}}$.
Then, for every view $v \in [2, v^*]$, $v \in \mathcal{V}(\mathcal{E})$.
\end{lemma}
\begin{proof}
We prove the lemma by induction.

\medskip
\noindent \underline{\emph{Base step:}} \emph{We prove that the statement of the lemma holds for any execution $\mathcal{E}_1$ in which exactly one \textsc{start-view} message is sent by correct processes.}
\\ To prove the base step, we show that the first \textsc{start-view} message sent by correct processes in any execution must be sent for view $2$.
% By \Cref{lemma:start_view_for_1}, the first \textsc{start-view} message must be sent for a view greater than $1$.
% no correct process sends $\langle \textsc{start-view}, 1 \rangle$.
Let $m = \langle \textsc{start-view}, v \rangle$ be the only \textsc{start-view} message sent by correct processes in $\mathcal{E}_1$; let $p_i$ be the sender of $m$.
By \Cref{lemma:start_view_for_1}, $v \geq 2$.
Moreover, message $m$ could only be sent at line~\ref{line:send_complete_1}.
Indeed, message $m$ could not be sent at line~\ref{line:send_complete_2} or line~\ref{line:send_complete_2_prime} as this would imply that $m$ is not the only \textsc{start-view} message sent by correct processes in $\mathcal{E}_1$ (due to the rule at line~\ref{line:receive_plurality}).
Similarly, message $m$ could not be sent at line~\ref{line:send_complete_3} or line~\ref{line:send_complete_3_prime} as this would mean that $m$ is not the only \textsc{start-view} message sent by correct processes in $\mathcal{E}_1$ (due to the rule at line~\ref{line:receive_quorum}).
Finally, when $p_i$ sends $m$ (line~\ref{line:send_complete_1}), the value of the $\mathit{view}_i$ variable must be $1$; otherwise, $m$ would not be the only message sent by correct processes in $\mathcal{E}_1$ (due to the rule at line~\ref{line:receive_quorum}).
Therefore, $m = \langle \textsc{start-view}, 2 \rangle$, which concludes the proof of the base step.

\medskip
\noindent \underline{\emph{Inductive step:}} \emph{We assume that the statement of the lemma holds for any execution $\mathcal{E}_j$ in which exactly $j$ \textsc{start-view} messages are sent by correct processes, for some $j \geq 1$.
We prove that the statement of the lemma holds for any continuation $\mathcal{E}_{j + 1}$ of $\mathcal{E}_j$ in which exactly $j + 1$ \textsc{start-view} messages are sent by correct processes.}
\\ Consider the first \textsc{start-view} message $m = \langle \textsc{start-view}, v \rangle$ sent by a correct process in a continuation of $\mathcal{E}_j$; let $p_i$ be the sender of $m$.
According to \Cref{lemma:start_view_for_1}, $v \geq 2$.
Let $v^j$ denote the greatest view of $\mathcal{V}(\mathcal{E}_j)$.
If $v \in [2, v^j + 1]$, the inductive step is concluded.
Hence, let $v > v^j + 1$.
We consider all places at which message $m$ could be sent by $p_i$:
\begin{compactitem}
    \item line~\ref{line:send_complete_1}:
    At the moment of sending $m$, the value of the $\mathit{view}_i$ variable is $v - 1 \geq v^j + 1$.
    Therefore, prior to updating the $\mathit{view}_i$ variable to $v - 1$ (line~\ref{line:update_view_2}), $p_i$ has received a $\langle \textsc{start-view}, v - 1 \rangle$ message from a correct process (line~\ref{line:receive_quorum}).
    Hence, $v - 1 \in \mathcal{V}(\mathcal{E}_j)$, which is impossible as $v - 1 > v^j$.

    \item line~\ref{line:send_complete_2}:
    At the moment of sending $m$, the value of the $\mathit{help\_view}_i$ variable is $v > v^j$.
    Prior to updating the $\mathit{help\_view}_i$ variable to $v$ (line~\ref{line:update_help_view}), $p_i$ has received a $\langle \textsc{start-view}, v \rangle$ message from a correct process (line~\ref{line:receive_plurality}).
    Therefore, $v \in \mathcal{V}(\mathcal{E}_j)$, which cannot be true as $v > v^j$.

    \item line~\ref{line:send_complete_2_prime}:
    At the moment of sending $m$, the value of the $\mathit{help\_view}_i$ variable is $v + 1 > v^j$.
    Prior to updating the $\mathit{help\_view}_i$ variable to $v + 1$ (line~\ref{line:update_help_view}), $p_i$ has received a $\langle \textsc{start-view}, v + 1 \rangle$ message from a correct process (line~\ref{line:receive_plurality}).
    Therefore, $v + 1 \in \mathcal{V}(\mathcal{E}_j)$, which is impossible as $v + 1 > v^j$.

    \item line~\ref{line:send_complete_3}:
    At the moment of sending $m$, the value of the $\mathit{view}_i$ variable is $v > v^j$.
    Prior to updating the $\mathit{view}_i$ variable to $v$ (line~\ref{line:update_view_2}), $p_i$ has received a $\langle \textsc{start-view}, v \rangle$ message from a correct process (line~\ref{line:receive_quorum}).
    Thus, $v \in \mathcal{V}(\mathcal{E}_j)$, which cannot be true as $v > v^j$.

    \item line~\ref{line:send_complete_3_prime}:
    At the moment of sending $m$, the value of the $\mathit{view}_i$ variable is $v + 1 > v^j$.
    Prior to updating the $\mathit{view}_i$ variable to $v + 1$ (line~\ref{line:update_view_2}), $p_i$ has received a $\langle \textsc{start-view}, v + 1 \rangle$ message from a correct process (line~\ref{line:receive_quorum}).
    Hence, $v + 1 \in \mathcal{V}(\mathcal{E}_j)$, which cannot be true as $v + 1 > v^j$.
\end{compactitem}
As it is impossible for $p_i$ to send the message $m = \langle \textsc{start-view}, v > v^j + 1 \rangle$, it follows that $v \in [2, v^j + 1]$, which concludes the inductive step.
\end{proof}

Next, we prove that the first \textsc{start-view} message for any view sent by a correct process must be sent at line~\ref{line:send_complete_1}.

\begin{lemma} \label{lemma:first_message}
For any view $v$, the first correct process that sends a $\langle \textsc{start-view}, v \rangle$ message does so at line~\ref{line:send_complete_1}.
\end{lemma}
\begin{proof}
% \Cref{lemma:start_view_for_1} proves that $v \geq 2$.
Consider any execution $\mathcal{E}_v$ in which exactly one $\langle \textsc{start-view}, v \rangle$ message is sent by correct processes; let that message be denoted by $m$, and let the sender of $m$ be $p_i$.
We now consider all the places at which $p_i$ could have sent $m$ in $\mathcal{E}_v$:
\begin{compactitem}
    \item line~\ref{line:send_complete_2}:
    At the moment of sending $m$, the value of the $\mathit{help\_view}_i$ variable is $v$.
    Prior to updating the $\mathit{help\_view}_i$ variable to $v$ (line~\ref{line:update_help_view}), $p_i$ has received a $\langle \textsc{start-view}, v \rangle$ message from a correct process (line~\ref{line:receive_plurality}).
    However, this implies that $m$ is not the only $\langle \textsc{start-view}, v \rangle$ message sent by correct processes in $\mathcal{E}_v$, thus making this case impossible.

    \item line~\ref{line:send_complete_2_prime}:
    At the moment of sending $m$, the value of the $\mathit{help\_view}_i$ variable is $v + 1$.
    Prior to updating the $\mathit{help\_view}_i$ variable to $v + 1$ (line~\ref{line:update_help_view}), $p_i$ has received a $\langle \textsc{start-view}, v + 1 \rangle$ message from a correct process (line~\ref{line:receive_plurality}); let us denote this message by $m'$.
    However, as $m$ is the only $\langle \textsc{start-view}, v \rangle$ message sent by correct processes in $\mathcal{E}_v$ and $m'$ is sent before $m$ (as $m'$ causally precedes $m$ in $\mathcal{E}_v$), the prefix of $\mathcal{E}_v$ in which $m$ is not yet sent contradicts \Cref{lemma:no_gaps}.
    Therefore, this case is impossible.

    \item line~\ref{line:send_complete_3}:
    At the moment of sending $m$, the value of the $\mathit{view}_i$ variable is $v$.
    Prior to updating the $\mathit{view}_i$ variable to $v$ (line~\ref{line:update_view_2}), $p_i$ has received a $\langle \textsc{start-view}, v \rangle$ message from a correct process (line~\ref{line:receive_quorum}).
    However, this implies that $m$ is not the only $\langle \textsc{start-view}, v \rangle$ message sent by correct processes in $\mathcal{E}_v$, thus making this case impossible.

    \item line~\ref{line:send_complete_3_prime}:
    At the moment of sending $m$, the value of the $\mathit{view}_i$ variable is $v + 1$.
    Prior to updating the $\mathit{view}_i$ variable to $v + 1$ (line~\ref{line:update_view_2}), $p_i$ has received a $\langle \textsc{start-view}, v + 1 \rangle$ message from a correct process (line~\ref{line:receive_quorum}); let us denote this message by $m'$.
    However, as $m$ is the only $\langle \textsc{start-view}, v \rangle$ message sent by correct processes in $\mathcal{E}_v$ and $m'$ is sent before $m$ (as $m'$ causally precedes $m$ in $\mathcal{E}_v$), the statement of \Cref{lemma:no_gaps} is violated in the prefix of $\mathcal{E}_v$ in which $m$ is not yet sent.
    Thus, this case is impossible as well.
\end{compactitem}
As all other possibilities could not have occurred, $p_i$ must have sent $m$ at line~\ref{line:send_complete_1}.
\end{proof}

The following lemma proves that, if a correct process enters any view $v > 1$, then at least one correct process has previously finished view $v - 1$.
Recall that a correct process enters a view $v$ once it invokes $\mathsf{start}()$ on $\mathcal{VC}(v)$ (line~\ref{line:enter_1} or line~\ref{line:enter_v}).
Moreover, a correct process finishes a view $v - 1$ once it receives a $\mathsf{finished}()$ indication (line~\ref{line:view_timer_expire}) from the view core abstraction associated with view $v - 1$ (i.e., $\mathcal{VC}(v - 1)$).

\begin{lemma} \label{lemma:finish_before_enter_next}
If any correct process enters any view $v > 1$, then at least one correct process has previously finished view $v - 1$.
\end{lemma}
\begin{proof}
If any correct process $p_i$ enters any view $v > 1$ (line~\ref{line:enter_v}), $p_i$ has previously received a $\langle \textsc{start-view}, v \rangle$ from a correct process (line~\ref{line:receive_quorum}).
Hence, \Cref{lemma:first_message} states that there exists a correct process $p_j$ that has sent a $\langle \textsc{start-view}, v \rangle$ message at line~\ref{line:send_complete_1} before $p_i$ enters $v$.
Therefore, process $p_j$ has received a $\mathsf{finished}()$ indication from $\mathcal{VC}(v - 1)$ (line~\ref{line:view_timer_expire}) before sending the \textsc{start-view} message at line~\ref{line:send_complete_1}, which concludes the proof.
\end{proof}

Next, we prove that if a correct process broadcasts a $\langle \textsc{start-view}, v \rangle$ message at line~\ref{line:send_complete_1}, for any view $v$, then that process has previously entered view $v - 1$.

\begin{lemma} \label{lemma:start_finish}
If a correct process $p_i$ broadcasts a $\langle \textsc{start-view}, v \rangle$ message at line~\ref{line:send_complete_1}, for any view $v > 1$, then $p_i$ has previously entered view $v - 1$.
\end{lemma}
\begin{proof}
As $p_i$ broadcasts a $\langle \textsc{start-view}, v \rangle$ message at line~\ref{line:send_complete_1}, $p_i$ has previously finished view $v - 1$ (line~\ref{line:view_timer_expire}).
Therefore, $p_i$ has previously invoked the $\mathsf{start}()$ operation on $\mathcal{VC}(v - 1)$, which concludes the lemma.
\end{proof}

The following lemma proves that, if a correct process enters any view $v > 1$ at time $t$, then a correct process has entered view $v - 1$ by time $t$.

\begin{lemma} \label{lemma:view_previous_entered}
Let any correct process $p_i$ enter any view $v > 1$ at some time $t$.
Then, at least one correct process has entered view $v - 1$ by time $t$.
\end{lemma}
\begin{proof}
At the moment of entering view $v > 1$ (line~\ref{line:enter_v}), the value of the $\mathit{view}_i$ variable is $v$.
Hence, $p_i$ has received $2t + 1$ $\langle \textsc{start-view}, v \rangle$ messages (due to the rule at line~\ref{line:receive_quorum}) by time $t$.
Let $p_j$ be the first correct process that sends a $\langle \textsc{start-view}, v \rangle$ message; note that $p_j$ does so by time $t$.
According to \Cref{lemma:first_message}, $p_j$ sends the \textsc{start-view} message at line~\ref{line:send_complete_1}.
Then, \Cref{lemma:start_finish} proves that $p_j$ has entered the view $v - 1$ by time $t$, which concludes the proof.
\end{proof}

% \jovan{Check: to be continued}
Finally, we prove that every view is eventually entered by a correct process.
This represents one of the crucial intermediate results.
Note that the following lemma does not imply that \emph{all} correct processes enter every view.

\begin{lemma} \label{lemma:every_view_entered}
Every view is eventually entered by a correct process.
\end{lemma}
\begin{proof}
By contradiction, suppose that this is not the case.
Let $v + 1$ be the smallest view that is not entered by any correct process.
As each correct process initially enters view $1$ (line~\ref{line:enter_1}), $v + 1 \geq 2$.
Moreover, by \Cref{lemma:view_previous_entered}, no correct process enters any view greater than $v + 1$.
We prove the lemma through a sequence of intermediate results.

\medskip
\noindent \underline{\emph{Step 1.}} \emph{No correct process $p_i$ sets the value of its $\mathit{view}_i$ variable to a view greater than $v$.}
\\ By contradiction, suppose that some correct process $p_i$ updates its $\mathit{view}_i$ variable to a view $v' > v$ (line~\ref{line:update_view_2}).
We now consider two cases:
\begin{compactitem}
    \item Let $v' > v + 1$.
    In this case, $p_i$ has received a \textsc{start-view} message for view $v'$ from a correct process (due to the rule at line~\ref{line:receive_quorum}).
    By \Cref{lemma:first_message}, the first correct process that sends a $\langle \textsc{start-view}, v' \rangle$ message does so at line~\ref{line:send_complete_1}.
    Therefore, \Cref{lemma:start_finish} shows that this correct process has previously entered view $v' - 1 > v$, which is impossible as no correct process enters any view greater than $v$.

    \item Let $v' = v + 1$.
    When $p_i$ updates its $\mathit{view}_i$ variable to $v' = v + 1$ (line~\ref{line:update_view_2}), $p_i$ invokes the $\mathsf{measure}(\delta)$ method on $\mathit{enter\_timer}_i$ (line~\ref{line:measure_enter}) .
    Importantly, this invocation is never canceled as $p_i$ never updates its $\mathit{view}_i$ variable to a view greater than $v' = v + 1$ (see the case above).
    % , and (2) the value of the $\mathit{view}_i$ variable never decreases (by \Cref{lemma:view_i_increases}).
    Hence, when the aforementioned invocation of the $\mathsf{measure}(\delta)$ method expires (line~\ref{line:enter_expires}), $p_i$ enters view $v + 1$ (line~\ref{line:enter_v}).
    However, this is impossible as no correct process enters a view greater than $v$.
\end{compactitem}
As neither of the two possible cases can occur, the statement is correct.

\medskip
\noindent \underline{\emph{Step 2.}} \emph{No correct process $p_i$ sets the value of its $\mathit{help\_view}_i$ variable to a view greater than $v + 1$ (line~\ref{line:update_help_view}).}
\\ By contradiction, suppose that some correct process $p_i$ updates its $\mathit{help\_view}_i$ variable to a view $v' > v + 1$.
Hence, $p_i$ has received a $\langle \textsc{start-view}, v' \rangle$ message from a correct process (due to the rule at line~\ref{line:receive_plurality}).
By \Cref{lemma:first_message}, the first correct process that sends a $\langle \textsc{start-view}, v' \rangle$ message does so at line~\ref{line:send_complete_1}.
Furthermore, \Cref{lemma:start_finish} shows that this correct process has previously entered view $v' - 1 > v$, which is impossible as no correct process enters a view greater than $v$.
Therefore, the statement holds.

\medskip
\noindent \underline{\emph{Step 3.}} \emph{If $v > 1$, then every correct process $p_i$ eventually broadcasts a $\langle \textsc{start-view}, v \rangle$ message.}
\\ Let $p_j$ be any correct process that enters view $v > 1$; such a process exists as $v$ is entered by a correct process.
Prior to entering view $v$, $p_j$ has received $2t + 1$ $\langle \textsc{start-view}, v \rangle$ messages (due to the rule at line~\ref{line:receive_quorum}), out of which (at least) $t + 1$ are sent by correct processes.
By contradiction, suppose that some correct process $p_i$ never broadcasts a $\langle \textsc{start-view}, v \rangle$ message.
Eventually, process $p_i$ receives the aforementioned $t + 1$ $\langle \textsc{start-view}, v \rangle$ messages.
% Process $p_i$ eventually receives $t + 1$ $\langle \textsc{start-view}, v \rangle$ messages.
We now consider two possibilities:
\begin{compactitem}
    \item The rule at line~\ref{line:receive_plurality} never activates for view $v$ at process $p_i$.
    This implies that $p_i$ eventually sets its $\mathit{view}_i$ variable to $v$ (line~\ref{line:update_view_2}); otherwise, the rule at line~\ref{line:receive_plurality} would eventually activate.
    (Recall that the statement of the first step proves that $p_i$ cannot set its $\mathit{view}_i$ variable to a view greater than $v$.)
    After updating its $\mathit{view}_i$ variable to $v$, process $p_i$ invokes the $\mathsf{measure}(\delta)$ method on $\mathit{enter\_timer}_i$ (line~\ref{line:measure_enter}).
    Due to the statement of the first step,
    % , and (2) the fact that the value of the $\mathit{view}_i$ variable never decreases (by \Cref{lemma:view_i_increases}),
    this invocation is never canceled.
    Therefore, once this invocation expires (line~\ref{line:enter_expires}), $p_i$ broadcasts a $\langle \textsc{start-view}, v \rangle$ message at line~\ref{line:send_complete_3}.
    % , which contradicts the fact that $p_i$ never broadcasts a \textsc{start-view} message for $v$.

    \item The rule at line~\ref{line:receive_plurality} eventually activates for view $v$.
    We further distinguish two scenarios:
    \begin{compactitem}
        \item The check at line~\ref{line:check_help} does not pass.
        In this case, the value of the $\mathit{help\_view}_i$ variable is equal to or greater than $v$.
        Moreover, by the statement of the second step, no correct process updates its $\mathit{help\_view}_i$ variable to a view greater than $v + 1$.
        Hence, the value of the $\mathit{help\_view}_i$ variable is $v$ or $v + 1$ when the check at line~\ref{line:check_help} does not pass.
        Let us investigate both possibilities:
        \begin{compactitem}
            \item The value of the $\mathit{help\_view}_i$ variable is $v + 1$.
            Immediately after $p_i$ has updated its $\mathit{help\_view}_i$ variable to $v + 1$ (line~\ref{line:update_help_view}), $p_i$ invoked the $\mathsf{measure}(\delta)$ method on $\mathit{help\_timer}_i$ (line~\ref{line:measure_help}).
            As $p_i$ never updates its $\mathit{help\_view}_i$ variable to a view greater than $v + 1$ (by the statement of the second step),
            % , and (2) the value of the $\mathit{help\_view}_i$ never decreases (by \Cref{lemma:help_view_i_increases}),
            the aforementioned invocation of the $\mathsf{measure}(\delta)$ method is never canceled.
            Thus, once the invocation expires (line~\ref{line:help_timer_expires}), $p_i$ broadcasts a $\langle \textsc{start-view}, v \rangle$ message at line~\ref{line:send_complete_2_prime}.
            (Note that, as $v > 1$, $v + 1 > 2$, which ensures that the check at line~\ref{line:check_help_2} passes.)

            \item The value of the $\mathit{help\_view}_i$ variable is $v$.
            Immediately after $p_i$ has updated its $\mathit{help\_view}_i$ variable to $v$ (line~\ref{line:update_help_view}), $p_i$ invoked the $\mathsf{measure}(\delta)$ method on $\mathit{help\_timer}_i$ (line~\ref{line:measure_help}).
            If this invocation does not get canceled, then $p_i$ broadcasts a $\langle \textsc{start-view}, v \rangle$ message at line~\ref{line:send_complete_2}.
            (Observe that the value of the $\mathit{help\_view}_i$ variable does not change between the invocation of the $\mathsf{measure}(\delta)$ method on $\mathit{help\_timer}_i$ and its expiration event due to \Cref{lemma:help_invocation_expiration}.)

            If the invocation gets canceled (line~\ref{line:cancel_help}), then $p_i$ has updated its $\mathit{help\_view}_i$ variable to a view greater than $v$ (because of the check at line~\ref{line:check_help}).
            Due to the statement of the second step, $p_i$ could have only updated $\mathit{help\_view}_i$ to $v + 1$ (line~\ref{line:update_help_view}).
            Immediately after updating $\mathit{help\_view}_i$ to $v + 1$, $p_i$ has invoked the $\mathsf{measure}(\delta)$ method on $\mathit{help\_timer}_i$ (line~\ref{line:measure_help}).
            Due to the fact that $p_i$ does not update its $\mathit{help\_view}_i$ variable to a view greater than $v + 1$ (by the statement of the second step), 
            % and (2) the value of the $\mathit{help\_view}_i$ never decreases (by \Cref{lemma:help_view_i_increases}), 
            the aforementioned invocation never gets canceled.
            Hence, once the invocation expires (line~\ref{line:help_timer_expires}), $p_i$ broadcasts a $\langle \textsc{start-view}, v \rangle$ at line~\ref{line:send_complete_2_prime}.
            (As $v > 1$, $v + 1 > 2$, thus ensuring that the check at line~\ref{line:check_help_2} passes.)
        \end{compactitem}

        \item The check at line~\ref{line:check_help} passes.
        In this case, $p_i$ updates its $\mathit{help\_view}_i$ variable to $v$ (line~\ref{line:update_help_view}).
        Moreover, $p_i$ invokes the $\mathsf{measure}(\delta)$ method on $\mathit{help\_timer}_i$ (line~\ref{line:measure_help}).
        From this point, the same argument as in the case immediately above is applied, which ensures that $p_i$ sends a $\langle \textsc{start-view}, v \rangle$ message at line~\ref{line:send_complete_2} or at line~\ref{line:send_complete_2_prime}.
    \end{compactitem}
\end{compactitem}
As $p_i$ broadcasts a $\langle \textsc{start-view}, v \rangle$ message in any possible case, the statement of the third step holds.

\medskip
\noindent \underline{\emph{Step 4.}} \emph{Every correct process $p_i$ eventually enters view $v$.}
\\ If $v = 1$, the statement of the lemma holds as every correct process enters view $1$ (line~\ref{line:enter_1}) immediately upon starting. 

Hence, let $v > 1$.
By the statement of the third step, every correct process eventually broadcasts a $\langle \textsc{start-view}, v \rangle$ message.
Therefore, every correct process $p_i$ eventually receives $2t + 1$ $\langle \textsc{start-view}, v \rangle$ messages (line~\ref{line:receive_quorum}).
We consider two cases:
\begin{compactitem}
    \item The rule at line~\ref{line:receive_quorum} never activates for view $v$ at process $p_i$.
    This implies that $p_i$ eventually sets its $\mathit{view}_i$ variable to $v$ (line~\ref{line:update_view_2}); otherwise, the rule at line~\ref{line:receive_plurality} would eventually activate.
    (Recall that the statement of the first step proves that $p_i$ cannot set its $\mathit{view}_i$ variable to a view greater than $v$.)

    \item The rule at line~\ref{line:receive_quorum} activates for view $v$ at process $p_i$.
    When the rule activates, $p_i$ updates its $\mathit{view}_i$ variable to $v$.
\end{compactitem}
In any of the two possibilities, every correct process $p_i$ eventually updates its $\mathit{view}_i$ variable to $v$ (line~\ref{line:update_view_2}) and invokes the $\mathsf{measure}(\delta)$ method on $\mathit{enter\_timer}_i$ (line~\ref{line:measure_enter}).
As $p_i$ does not update its $\mathit{view}_i$ variable to a view greater than $v$ (by the statement of the first step), 
% and (2) the value of the $\mathit{view}_i$ never decreases (by \Cref{lemma:view_i_increases}), 
$\mathit{enter\_timer}_i$ eventually expires (line~\ref{line:enter_expires}), and $p_i$ enters view $v$ (line~\ref{line:enter_v}).
(Note that the value of the $\mathit{view}_i$ variable does not change between the invocation of the $\mathsf{measure}(\cdot)$ method on $\mathit{enter\_timer}_i$ and its expiration event due to \Cref{lemma:enter_invocation_expiration}.)

\medskip
\noindent \underline{\emph{Epilogue.}} Due to the statement of the fourth step, every correct process eventually enters view $v$.
Moreover, no correct process ever abandons view $v$ (i.e., invokes $\mathsf{stop}()$ on $\mathcal{VC}(v)$) as no correct process ever enters a view greater than $v$.

First, every correct process $p_i$ eventually validates some bit in view $v$.
If $v = 1$, $p_i$'s proposal is trivially validated.
Otherwise, as $v > 1$ is entered by $p_i$, $p_i$ has previously received $2t + 1$ $\langle \textsc{start-view}, v \rangle$ messages (line~\ref{line:receive_quorum}).
Therefore, before $p_i$ has entered view $v$, some correct process $p_j$ had sent a $\langle \textsc{start-view}, v \rangle$ message at line~\ref{line:send_complete_1} (by \Cref{lemma:first_message}).
Before sending the $\langle \textsc{start-view}, v \rangle$ message, $p_j$ has finished view $v - 1$ (line~\ref{line:view_timer_expire}) by receiving $2f + 1$ \textsc{echo} messages for some bit $b$.
As at least $t + 1$ $\langle \textsc{echo}, b \rangle$ messages received by $p_j$ are sent by correct processes, $p_i$ must eventually validate $b$ (if it does not validate $\bar{b}$ before).
Moreover, each correct process eventually comes to the last step of the view (as graded consensus primitives ensure termination, every timer eventually expires and no correct process $p_k$ ever gets trapped in the synchronous consensus primitive due to the utilization of $\mathit{sync\_consensus\_timer}_k$).
Finally, every correct process concludes the last step of $\mathcal{VC}(v)$ as there exists a bit for which every correct process broadcasts an \textsc{echo} message.
Hence, every correct process eventually broadcasts $\langle \textsc{start-view}, v + 1 \rangle$ at line~\ref{line:send_complete_1}.

Therefore, every correct process eventually receives $2f + 1$ $\langle \textsc{start-view}, v + 1 \rangle$ messages and the rule at line~\ref{line:receive_quorum} activates; recall that, according to the statement of the first step, no correct process $p_i$ updates its $\mathit{view}_i$ variable to a view greater than $v$.
Hence, every correct process $p_i$ eventually updates its $\mathit{view}_i$ variable to a view greater than $v$ (line~\ref{line:update_view_2}), which contradicts the statement of the first step and concludes the proof of the lemma.
\end{proof}

% \jovan{Stopped here}
We now introduce a few definitions.
First, for every view $v$, we define the first time any correct process enters $v$.

\begin{definition} [First-entering time] \label{definition:first_time}
For every view $v$, $t_v$ denotes the time at which the first correct process enters $v$.
\end{definition}

Next, we define the greatest view that is entered by a correct process before GST.

\begin{definition} [View $\vmax$] \label{definition:vmax}
We denote by $\vmax$ the greatest view for which $t_{\vmax} < \text{GST}$.
% that is entered by a correct process before GST.
If such a view does not exist, $\vmax = 0$.\footnote{We slightly abuse notation here as $0 \notin \mathsf{View}$.}
\end{definition}

The final definition is concerned with the smallest view that is entered by every correct process at or after GST.

\begin{definition} [View $\vfinal$] \label{definition:vfinal}
We denote by $\vfinal$ the smallest view for which $t_{\vfinal} \geq \text{GST}$.
% that is not entered by any correct process before GST.
\end{definition}

% Note that \Cref{lemma:view_previous_entered} implies that $\vfinal = \vmax + 1$.
The following lemma proves that, for every view $v \geq \vfinal$, $t_v \geq \text{GST}$.

\begin{lemma} \label{lemma:starting_time_vfinal}
For every view $v \geq \vfinal$, $t_v \geq \text{GST}$.
\end{lemma}
\begin{proof}
By the definition of $\vfinal$ (\Cref{definition:vfinal}), $t_{\vfinal} \geq \text{GST}$.
Furthermore, \Cref{lemma:view_previous_entered} proves that $t_{v - 1} \leq t_v$, for any view $v \geq 2$.
As $v \geq \vfinal$, $t_v \geq t_{\vfinal} \geq \text{GST}$.
Therefore, $t_v \geq \text{GST}$.
\end{proof}

Next, we give a relation between the time at which a correct process enters a view $v \geq \vfinal$ and the time at which it sends a $\langle \textsc{start-view}, v + 1 \rangle$ message at line~\ref{line:send_complete_1}.
% Recall that $\mathit{view\_duration}$ is a constant of the view core primitive (line~\ref{line:init_view_duration} of \Cref{algorithm:repeater_view_core}).

\begin{lemma} \label{lemma:start_view_message_no_drifts}
Let $p_i$ be any correct process and let $v$ be any view such that (1) $v \geq \vfinal$, (2) $p_i$ enters $v$ at time $t_v(i)$, and (3) $p_i$ broadcasts a $\langle \textsc{start-view}, v + 1 \rangle$ at line~\ref{line:send_complete_1} at some time $t^*$.
Then, $t^* \geq t_v(i) + \mathit{view\_duration}$, where $\mathit{view\_duration}$ is a constant associated with the view core abstraction and defined at line~\ref{line:init_view_duration} of \Cref{algorithm:repeater_view_core}.
\end{lemma}
\begin{proof}
As $v \geq \vfinal$, $t_v \geq \text{GST}$ (by \Cref{lemma:starting_time_vfinal}).
Since $t_v(i) \geq t_v$, $t_v(i) \geq \text{GST}$.
Hence, the local clock of $p_i$ does not drift while executing $\mathcal{VC}(v)$, which implies that $p_i$ cannot finish view $v$ before time $t_v(i) + \mathit{view\_duration}$, i.e., $t^* \geq t_v(i) + \mathit{view\_duration}$ (see \Cref{algorithm:repeater_view_core}).
\end{proof}

The following lemma represents a direct consequence of \Cref{lemma:start_view_message_no_drifts}.

\begin{lemma} \label{lemma:first_start_view_message}
No correct process sends a $\langle \textsc{start-view}, v \rangle$ message for any view $v > \vfinal$ before time $t_{v -  1} + \mathit{view\_duration}$.
\end{lemma}
\begin{proof}
Consider any view $v > \vfinal$.
Let $t^*$ be the time at which the first correct process (say, $p_i$) sends a $\langle \textsc{start-view}, v \rangle$ message.
By \Cref{lemma:start_finish}, $p_i$ previously entered $v - 1$; let $t_{v - 1}(i)$ denote the time at which $p_i$ enters $v - 1$.
As $v - 1 \geq \vfinal$, \Cref{lemma:start_view_message_no_drifts} states that $t^* \geq t_{v - 1}(i) + \mathit{view\_duration} \geq t_{v - 1} + \mathit{view\_duration}$, which concludes the lemma.
\end{proof}

Next, we prove that no correct process $p_i$ updates its $\mathit{view}_i$ variable to a view greater than $\vfinal$ before time $t_{\vfinal} + \mathit{view\_duration}$.

\begin{lemma} \label{lemma:update_view_time}
No correct process $p_i$ updates its $\mathit{view}_i$ variable to a view greater than $\vfinal$ before time $t_{\vfinal} + \mathit{view\_duration}$.
\end{lemma}
\begin{proof}
Let $p_i$ be any correct process that updates its $\mathit{view}_i$ variable to any view $v$ such that $v > \vfinal$; $p_i$ does so at line~\ref{line:update_view_2}.
As $v - 1 \geq \vfinal$, \Cref{lemma:view_previous_entered} proves that $t_{v - 1} \geq t_{\vfinal}$.
Prior to updating $\mathit{view}_i$ to $v$, $p_i$ has received a $\langle \textsc{start-view}, v \rangle$ message from a correct process (due to the rule at line~\ref{line:receive_quorum}).
By \Cref{lemma:first_start_view_message}, no correct process sends a $\langle \textsc{start-view}, v \rangle$ message before time $t_{v - 1} + \mathit{view\_duration}$.
Therefore, $p_i$ could not have updated its $\mathit{view}_i$ variable to $v$ before time $t_{v - 1} + \mathit{view\_duration} \geq t_{\vfinal} + \mathit{view\_duration}$, which concludes the proof.
\end{proof}

Similarly to \Cref{lemma:update_view_time}, no correct process $p_i$ updates its $\mathit{help\_view}_i$ variable to a view greater than $\vfinal$ before time $t_{\vfinal} + \mathit{view\_duration}$.

\begin{lemma} \label{lemma:update_help_view_time}
No correct process $p_i$ updates its $\mathit{help\_view}_i$ variable to a view greater than $\vfinal$ before time $t_{\vfinal} + \mathit{view\_duration}$.
\end{lemma}
\begin{proof}
Let $p_i$ be any correct process that updates its $\mathit{help\_view}_i$ variable to any view $v$ such that $v > \vfinal$; $p_i$ does so at line~\ref{line:update_help_view}.
As $v - 1 \geq \vfinal$, \Cref{lemma:view_previous_entered} proves that $t_{v - 1} \geq t_{\vfinal}$.
Prior to updating $\mathit{help\_view}_i$ to $v$, $p_i$ has received a $\langle \textsc{start-view}, v \rangle$ message from a correct process (due to the rule at line~\ref{line:receive_plurality}).
By \Cref{lemma:first_start_view_message}, no correct process sends a $\langle \textsc{start-view}, v \rangle$ message before time $t_{v - 1} + \mathit{view\_duration}$.
Therefore, $p_i$ could not have updated its $\mathit{help\_view}_i$ variable to $v$ before time $t_{v - 1} + \mathit{view\_duration} \geq t_{\vfinal} + \mathit{view\_duration}$, which concludes the proof.
\end{proof}

Next, assuming that $\vfinal > 1$, we prove that every correct process broadcasts a $\langle \textsc{start-view}, \vfinal \rangle$ message by time $t_{\vfinal} + 2\delta$.

\begin{lemma} \label{lemma:start_view_v_final_all_correct}
If $\vfinal > 1$, then every correct process broadcasts a $\langle \textsc{start-view}, \vfinal \rangle$ message by time $t_{\vfinal} + 2\delta$.
\end{lemma}
\begin{proof}
Recall that $t_{\vfinal}$ denotes the time at which the first correct process enters view $\vfinal$.
Let us denote that process by $p_i$.
As $p_i$ enters $\vfinal > 1$ (line~\ref{line:enter_v}) at time $t_{\vfinal} \geq \text{GST}$, $p_i$ has received $2t + 1$ $\langle \textsc{start-view}, \vfinal \rangle$ messages by time $t_{\vfinal}$ (due to the rule at line~\ref{line:receive_quorum}).
At least $t + 1$ out of the aforementioned $2t + 1$ $\langle \textsc{start-view}, \vfinal \rangle$ messages have been sent by correct processes.
Consider now any correct process $p_j$.
Process $p_j$ receives at least $t + 1$ $\langle \textsc{start-view}, \vfinal \rangle$ messages at some time $t^*$; as $t_{\vfinal} \geq \text{GST}$, $t^* \leq t_{\vfinal} + \delta$.
At time $t^*$, the following holds at process $p_j$: (1) $\mathit{view}_j \leq \vfinal$ as $\mathit{view\_duration} > \delta$ (by \Cref{lemma:update_view_time}), and (2) $\mathit{help\_view}_j \leq \vfinal$ as $\mathit{view\_duration} > \delta$ (by \Cref{lemma:update_help_view_time}).
We distinguish two scenarios:
\begin{compactitem}
    \item Let $\mathit{view}_j = \vfinal$ at process $p_j$ when $p_j$ receives $t + 1$ $\langle \textsc{start-view}, \vfinal \rangle$ messages at time $t^* \leq t_{\vfinal} + \delta$.
    In this case, process $p_j$ has previously invoked the $\mathsf{measure}(\delta)$ method on $\mathit{enter\_timer}_j$ (line~\ref{line:measure_enter}).
    Importantly, this invocation cannot be canceled as \Cref{lemma:update_view_time} guarantees that $p_j$ cannot update its $\mathit{view}_j$ variable to a view greater than $\vfinal$ before time $t_{\vfinal} + \mathit{view\_duration} > t_{\vfinal} + 2\delta$ (recall that $t^* \leq t_{\vfinal} + \delta$).
    % , and (2) the value of the $\mathit{view}_j$ variable never decreases (by \Cref{lemma:view_i_increases}).
    Hence, the aforementioned invocation produces an expiration event by time $t_{\vfinal} + 2\delta$ (line~\ref{line:enter_expires}), and $p_j$ broadcasts a $\langle \textsc{start-view}, \vfinal \rangle$ message (line~\ref{line:send_complete_3}) by time $t_{\vfinal} + 2\delta$.
    Therefore, the statement of the lemma holds in this case.

    \item Let $\mathit{view}_j < \vfinal$ at process $p_j$ when $p_j$ receives $t + 1$ $\langle \textsc{start-view}, \vfinal \rangle$ messages at time $t^* \leq t_{\vfinal} + \delta$.
    Hence, the rule at line~\ref{line:receive_plurality} activates at time $t^*$.
    We further distinguish two possibilities:
    \begin{compactitem}
        \item Let the check at line~\ref{line:check_help} pass.
        In this case, $p_j$ updates its $\mathit{help\_view}_j$ variable to $\vfinal$ (line~\ref{line:update_help_view}) and invokes the $\mathsf{measure}(\delta)$ method on $\mathit{help\_timer}_i$ (line~\ref{line:measure_help}).
        Importantly, the aforementioned invocation does not get canceled as $p_j$ cannot update its $\mathit{help\_view}_j$ variable to a view greater than $v$ before time $t_{\vfinal} + \mathit{view\_duration} > t_{\vfinal} + 2\delta$ (by \Cref{lemma:update_help_view_time}).
        % , and (2) the value of the $\mathit{view}_j$ variable never decreases (by \Cref{lemma:help_view_i_increases}).
        Hence, by time $t_{\vfinal} + 2\delta$, the aforementioned invocation produces an expiration event (line~\ref{line:help_timer_expires}), and $p_j$ broadcasts a $\langle \textsc{start-view}, \vfinal \rangle$ message (line~\ref{line:send_complete_2}).
        Thus, the statement of the lemma holds.

        \item Let the check at line~\ref{line:check_help} not pass.
        As the check does not pass, the value of the $\mathit{help\_view}_j$ variable is $\vfinal$; recall that it cannot be greater than $\vfinal$ at time $t^* \leq t_{\vfinal} + \delta$ due to the fact that $\delta < \mathit{view\_duration}$ and \Cref{lemma:update_help_view_time}.
        Hence, $p_j$ has previously updated its $\mathit{help\_view}_j$ variable to $\vfinal$ (line~\ref{line:update_help_view}) and invoked the $\mathsf{measure}(\delta)$ method on $\mathit{help\_timer}_j$ (line~\ref{line:measure_help}).
        Crucially, this invocation is never canceled as $p_j$ does not update its $\mathit{help\_view}_j$ variable to a view greater than $\vfinal$ before time $t_{\vfinal} + \mathit{view\_duration} > t_{\vfinal} + 2\delta$ (by \Cref{lemma:update_help_view_time}).
        % , and (2) the value of the $\mathit{help\_view}_j$ variable never decreases (by \Cref{lemma:help_view_i_increases}).
        Hence, by time $t_{\vfinal} + 2\delta$, the aforementioned invocation produces an expiration event (line~\ref{line:help_timer_expires}), and $p_j$ broadcasts a $\langle \textsc{start-view}, \vfinal \rangle$ message (line~\ref{line:send_complete_2}).
        Thus, the statement of the lemma holds.
    \end{compactitem}
\end{compactitem}
As the statement of the lemma holds in all possible scenarios, the proof is concluded.
\end{proof}

Next, we prove that every correct process enters view $\vfinal$ by time $t_{\vfinal} + 4\delta$.

\begin{lemma} \label{lemma:vfinal_start}
Every correct process enters view $\vfinal$ by time $t_{\vfinal} + 4\delta$.
\end{lemma}
\begin{proof}
Recall that $t_{\vfinal}$ denotes the time at which the first correct process enters view $\vfinal$.
If $\vfinal = 1$, all correct processes enter $\vfinal$ at time $t_{\vfinal} = \text{GST}$.
Hence, the lemma holds in this case.

Let $\vfinal > 1$.
By \Cref{lemma:start_view_v_final_all_correct}, all correct processes broadcast a $\langle \textsc{start-view}, \vfinal \rangle$ message by time $t_{\vfinal} + 2\delta$.
Therefore, all correct processes receive $2t + 1$ $\langle \textsc{start-view}, \vfinal \rangle$ messages by time $t_{\vfinal} + 3\delta$.
Note that, for any correct process $p_i$, when $p_i$ receives the aforementioned $2t + 1$ messages, the value of the $\mathit{view}_i$ variable is equal to or smaller than $\vfinal$ as $p_i$ does not update its $\mathit{view}_i$ variable to a view greater than $\vfinal$ before time $t_{\vfinal} + \mathit{view\_duration} > t_{\vfinal} + 3\delta$ (by \Cref{lemma:update_view_time}).
% , and (2) the value of the $\mathit{view}_i$ variable never decreases (by \Cref{lemma:view_i_increases}).
Let us consider two possibilities when any correct process $p_i$ receives the aforementioned $2t + 1$ $\langle \textsc{start-view}, \vfinal \rangle$ messages:
\begin{compactitem}
    \item Let $\mathit{view}_i = \vfinal$.
    Hence, $p_i$ has previously updated its $\mathit{view}_i$ variable to $\vfinal$ (line~\ref{line:update_view_2}) and invoked the $\mathsf{measure}(\delta)$ method on $\mathit{enter\_timer}_i$ (line~\ref{line:measure_enter}).
    Crucially, this invocation is not canceled as $p_i$ does not update its $\mathit{view}_i$ variable to a view greater than $\vfinal$ before time $t_{\vfinal} + \mathit{view\_duration} > t_{\vfinal} + 4\delta$ (by \Cref{lemma:update_view_time}).
    % , and (2) the value of the $\mathit{view}_i$ variable never decreases (by \Cref{lemma:view_i_increases}).
    Thus, by time $t_{\vfinal} + 4\delta$ (at the latest), the aforementioned invocation produces an expiration event (line~\ref{line:enter_expires}), and $p_i$ enters $\vfinal$ (line~\ref{line:enter_v}).
    The statement of the lemma holds in this case.

    \item Let $\mathit{view}_i < \vfinal$.
    Hence, the rule at line~\ref{line:receive_quorum} activates.
    This implies that $p_i$ updates its $\mathit{view}_i$ variable to $\vfinal$ (line~\ref{line:update_view_2}) and invokes the $\mathsf{measure}(\delta)$ method on $\mathit{enter\_timer}_i$ (line~\ref{line:measure_enter}).
    Crucially, this invocation is not canceled as $p_i$ does not update its $\mathit{view}_i$ variable to a view greater than $\vfinal$ before time $t_{\vfinal} + \mathit{view\_duration} > t_{\vfinal} + 4\delta$ (by \Cref{lemma:update_view_time}).
    % , and (2) the value of the $\mathit{view}_i$ variable never decreases (by \Cref{lemma:view_i_increases}).
    Thus, by time $t_{\vfinal} + 4\delta$, the aforementioned invocation produces an expiration event (line~\ref{line:enter_expires}), and $p_i$ enters $\vfinal$ (line~\ref{line:enter_v}).
    The statement of the lemma holds in this case.
\end{compactitem}
As the statement of the lemma holds in both possible cases, the proof is concluded.
\end{proof}

The following lemma proves that no correct process enters a view greater than $\vfinal$ before time $t_{\vfinal} + \mathit{view\_duration}$.

\begin{lemma} \label{lemma:vfinal_end}
No correct process enters a view greater than $\vfinal$ before time $t_{\vfinal} + \mathit{view\_duration}$.
\end{lemma}
\begin{proof}
For any correct process $p_i$ to enter a view greater than $\vfinal$ (line~\ref{line:enter_v}), $p_i$ must have previously updated its $\mathit{view}_i$ variable to a view greater than $\vfinal$.
As $p_i$ cannot update its $\mathit{view}_i$ variable to a view greater than $\vfinal$ before time $t_{\vfinal} + \mathit{view\_duration}$ (by \Cref{lemma:update_view_time}), the lemma holds.
\end{proof}

% \jovan{Stop here}
We now prove that, if a correct process validates a bit in $\mathcal{VC}(\vfinal)$ at some time $t$, then $t_{\vfinal} \leq t \leq t_{\vfinal} + \delta$.

\begin{lemma} \label{lemma:vfinal_validation_time}
Consider any correct process $p_i$.
Then, process $p_i$ validates some bit in $\mathcal{VC}(\vfinal)$ by time $t_{\vfinal} + \delta$.
\end{lemma}
\begin{proof}
% No correct process validates any bit in $\mathcal{VC}(\vfinal)$ before entering $\vfinal$.
% Thus, $t_{\vfinal} \leq t$.
If $\vfinal = 1$, then every correct process validates some bit by time $t_{\vfinal} = \text{GST}$, which concludes the lemma.

Let $\vfinal > 1$.
As the first correct process that enters view $\vfinal$ does so at time $t_{\vfinal}$, \Cref{lemma:finish_before_enter_next} guarantees some correct process $p_j$ has finished view $\vfinal - 1$ by time $t_{\vfinal}$.
For $p_j$ to finish view $\vfinal - 1$, $p_j$ has necessarily received $2t + 1$ \textsc{echo} messages for some bit $b$ in $\mathcal{VC}(\vfinal - 1)$ (by the rule at line~\ref{line:rcv_enough_echo_to_leave} of \Cref{algorithm:repeater_view_core}).
At least $t + 1$ of the aforementioned \textsc{echo} messages are sent by correct processes by time $t_{\vfinal}$, which implies that every correct process receives these messages by time $t_{\vfinal} + \delta$, and validates bit $b$ (if it has not validated the other bit before).
\end{proof}

Next, we define synchronized executions of synchronous algorithms.

\begin{definition} [Synchronized executions] \label{definition:synchronized_execution}
Let $\mathcal{A}$ be any synchronous algorithm.
An execution of $\mathcal{A}$ is said to be \emph{synchronized} if and only if the following holds:
\begin{compactitem}
    \item Let $t_{\mathcal{A}}$ denote the time at which the first correct process starts executing $\mathcal{A}$.
    Then, $t_{\mathcal{A}} \geq \text{GST}$.

    \item All correct processes start executing $\mathcal{A}$ by time $t_{\mathcal{A}} + 4\delta$.

    \item The round duration is $5\delta$.

    \item In round $r$ that locally begins at time $t_r(i)$ (note that $t_r(i) \geq \text{GST}$) at a correct process $p_i$, $p_i$ processes algorithmic messages of $\mathcal{A}$ associated with round $r$ if they are received by time $t_r(i) + 5\delta$.
\end{compactitem}
\end{definition}

The following lemma proves that a synchronized execution of a synchronous algorithm $\mathcal{A}$ is a valid execution of $\mathcal{A}$.

\begin{lemma} \label{lemma:synchronized_execution}
Let $\mathcal{A}$ be any synchronous algorithm, and let $\mathcal{E}_s$ be any synchronized execution of $\mathcal{A}$.
Then, $\mathcal{E}_s$ is a valid execution of $\mathcal{A}$.
\end{lemma}
\begin{proof}
As all correct processes start executing $\mathcal{A}$ at or after GST, the local clocks of processes do not drift.
Hence, every correct process accurately measures the duration of each round (i.e., $5\delta$).

Consider any correct process $p_i$.
Let $p_i$ start a round $r$ at some time $t_r(i)$.
Let $p_j$ be another correct process that starts round $r$ at some time $t_r(j)$ and sends a message to $p_i$ in round $r$.
As we assume that all correct processes start executing $\mathcal{A}$ by time $t_{\mathcal{A}} + 4\delta$ and the local clocks of correct processes do not drift (as $t_{\mathcal{A}} \geq \text{GST}$), $t_r(j) \leq t_r(i) + 4\delta$.
Moreover, a message sent by $p_j$ to $p_i$ (at time $t_r(j)$) arrives at time $t_a$, where $t_a \leq t_r(j) + \delta$.
Note that $p_i$ starts executing round $r + 1$ (and stops executing round $r$) at time $t_{r + 1}(i) = t_{r}(i) + 5\delta$.
Hence, $t_a \leq t_r(i) + 5\delta = t_{r + 1}(i)$, and the message will be processed by $p_i$ while executing round $r$, which concludes the proof of the lemma.
\end{proof}

We now prove that the execution of the synchronous consensus primitive employed in view $\vfinal$ is synchronized.
% Recall that $\mathit{gc\_start}$ is the first graded consensus primitive of a view core abstraction.

\begin{lemma} \label{lemma:sync_consensus_synchronized_execution}
The execution of the $\mathit{sync\_consensus}$ primitive employed in $\mathcal{VC}(\vfinal)$ is synchronized.
\end{lemma}
\begin{proof}
The lemma holds as (1) all processes start executing $\mathit{sync\_consensus}$ at or after GST (as $t_{\vfinal} \geq \text{GST}$), (2) all correct processes start executing $\mathit{sync\_consensus}$ at most $4\delta$ time within each other as (a) all correct processes terminate from $\mathit{gc\_start}$ by time $t_{\vfinal} + \mathit{gc\_duration}$ (ensured by the $\mathit{gc\_start}$ primitive), and (b) every correct process $p_i$ invokes the $\mathsf{measure}(\mathit{gc\_duration})$ $4\delta$ within each other, (3) the round duration is $5\delta$ (ensured by line~\ref{line:propose_sync_consensus}), and (4) every correct process $p_i$ processes algorithmic messages associated with round $r$ if they are received by time $t_r(i) + 5\delta$, where $t_r(i)$ is the local time at which $p_i$ starts round $r$ of $\mathit{sync\_consensus}$.
\end{proof}

Finally, we are ready to prove that \name satisfies termination.

\begin{lemma} [Termination] \label{lemma:repeater_termination}
\name satisfies termination.
Specifically, every correct process decides by time $t_{\vfinal} + \mathit{view\_duration}$.
\end{lemma}
\begin{proof}
By \Cref{lemma:every_view_entered}, every view is eventually entered by at least one correct process.
According to \Cref{lemma:vfinal_start}, every correct process enters view $\vfinal$ by time $t_{\vfinal} + 4\delta$.
Moreover, no correct process leaves view $\vfinal$ (i.e., enters another view) before time $t_{\vfinal} + \mathit{view\_duration} = t_{\vfinal} + 2 \cdot \mathit{gc\_duration} + \mathit{sync\_consensus\_steps} \cdot \mathit{step\_duration} + \mathit{echo\_duration}$ according to \Cref{lemma:vfinal_end}, which ensures sufficient overlap for each closed-box primitive of $\mathcal{VC}(\vfinal)$.
To prove the lemma, we rely on the following intermediate result.

% As the duration of each communication sub-round is $5\delta$, all correct processes are synchronized at the level of sub-rounds (of $5\delta$ duration) in $\vfinal$.
% Note that no correct process leaves $\vfinal$ before it finishes all communication sub-rounds of $\vfinal$.
% We conclude the proof through a sequence of intermediate results.

\medskip
\noindent \underline{\emph{Intermediate result.}} \emph{All correct processes propose the same bit to the $\mathit{gc\_end}$ primitive of $\mathcal{VC}(\vfinal)$.}
\\ By \Cref{lemma:sync_consensus_synchronized_execution}, the execution of the $\mathit{sync\_consensus}$ primitive is synchronized.
Moreover, as this execution is a valid execution of $\mathit{sync\_consensus}$ (by \Cref{lemma:synchronized_execution}) and every correct process executes $\mathcal{T}$ synchronous rounds, every correct process decides from $\mathit{sync\_consensus}$.
Therefore, no correct process inputs to the $\mathit{gc\_end}$ primitive of $\mathcal{VC}(\vfinal)$ at line~\ref{line:gc_end_input_3} of \Cref{algorithm:repeater_view_core}.
% Therefore, every correct process proposes to $\mathit{gc\_end}$.

Consider now any two correct processes $p_i$ and $p_j$.
Let $p_i$ propose bit $b$ to $\mathit{gc\_end}$, and let $p_j$ propose bit $b'$ to $\mathit{gc\_end}$ while executing $\mathcal{VC}(\vfinal)$.
We consider three possibilities:
\begin{compactitem}
    \item Let $p_i$ (resp., $p_j$) output $b$ (resp., $b'$) from the $\mathit{gc\_start}$ primitive with grade $1$, and inputs to $\mathit{gc\_end}$ at line~\ref{line:gc_end_input_1} of \Cref{algorithm:repeater_view_core}.
    In this case, $b = b'$ due to the consistency property of the $\mathit{gc\_start}$ primitive.

    \item Let $p_i$ output $b$ from $\mathit{gc\_start}$ with grade $1$, and inputs to $\mathit{gc\_end}$ at line~\ref{line:gc_end_input_1} of \Cref{algorithm:repeater_view_core}.
    Moreover, let $p_j$ output from $\mathit{gc\_start}$ with grade $0$, and let $p_j$ decide $b'$ from $\mathit{sync\_consensus}$ (thus, $p_j$ inputs to $\mathit{gc\_end}$ at line~\ref{line:gc_end_input_2} of \Cref{algorithm:repeater_view_core}).
    As $p_i$ decides $b$ with grade $1$ from $\mathit{gc\_start}$, all correct processes propose $b$ to $\mathit{sync\_consensus}$ (due to the consistency property of graded consensus).
    Since $\mathit{sync\_consensus}$ satisfies validity, $b' = b$.

    \item Let both $p_i$ and $p_j$ output a bit with grade $0$ from the $\mathit{gc\_start}$ primitive.
    Moreover, let $p_i$ (resp., $p_j$) decide 
    $b$ (resp., $b'$) from $\mathit{sync\_consensus}$.
    (Thus, both $p_i$ and $p_j$ input to $\mathit{gc\_end}$ at line~\ref{line:gc_end_input_2} of \Cref{algorithm:repeater_view_core}.)
    In this case, $b = b'$ due to the agreement property of $\mathit{sync\_consensus}$.
\end{compactitem}

\medskip
\noindent \underline{\emph{Epilogue.}} Recall that no correct process leaves view $\vfinal$ before time $t_{\vfinal} + \mathit{view\_duration}$, which ensures that each process outputs from the $\mathit{gc\_end}$ primitive.
As all correct processes propose the same bit to the $\mathit{gc\_end}$ primitive (due to the statement of the intermediate step), the validity property of the $\mathit{gc\_end}$ primitive ensures that all correct processes output a bit with grade $1$.
Therefore, all correct processes decide in view $\vfinal$ (line~\ref{line:decide} of \Cref{algorithm:repeater_view_core}), which happens by time $t_{\vfinal} + \mathit{view\_duration}$.
% i.e., while executing $\mathcal{VC}(\vfinal)$.
\end{proof} 

Next, we prove that \name satisfies agreement.
We start by proving that, if any correct process decides a bit $b$ in some view $v$, no correct process sends an $\langle \textsc{echo}, \bar{b} \rangle$ message in $\mathcal{VC}(v')$, for any view $v' \geq v$.

\begin{lemma} \label{lemma:decide_echo}
If a correct process decides a bit $b$ in some view $v$ (i.e., while executing $\mathcal{VC}(v)$), then no correct process sends an $\langle \textsc{echo}, \bar{b} \rangle$ message in $\mathcal{VC}(v')$, for any view $v' \geq v$.
\end{lemma}
\begin{proof}
We prove the lemma by induction.

\medskip
\noindent \underline{\emph{Base step:}} \emph{No correct process sends an $\langle \textsc{echo}, \bar{b} \rangle$ message while executing $\mathcal{VC}(v)$.}
\\ As a correct process decides $b$ in $\mathcal{VC}(v)$ (line~\ref{line:decide} of \Cref{algorithm:repeater_view_core}), that correct process has previously output $(b, 1)$ from $\mathit{gc\_end}$ (due to the check at line~\ref{line:gc_end_grade_1} of \Cref{algorithm:repeater_view_core}).
Therefore, the consistency property of $\mathit{gc\_end}$ ensures that all correct processes output $b$ (with grade $1$ or $0$) from $\mathit{gc\_end}$.
Hence, no correct process sends an $\langle \textsc{echo}, \bar{b} \rangle$ message while executing $\mathcal{VC}(v)$.

\medskip
\noindent \underline{\emph{Inductive step:}} \emph{We assume that no correct process sends an $\langle \textsc{echo}, \bar{b} \rangle$ message while executing $\mathcal{VC}(v')$, for some view $v' \geq v$.
We prove that no correct process sends an $\langle \textsc{echo}, \bar{b} \rangle$ message while executing $\mathcal{VC}(v' + 1)$.}
\\ Any correct process that inputs to the $\mathit{gc\_start}$ primitive inputs bit $b$.
(Indeed, due to the inductive hypothesis, bit $\bar{b}$ cannot be validated at a correct process.)
Therefore, every correct process that outputs from $\mathit{gc\_start}$ outputs bit $b$ with grade $1$ (due to the validity property of $\mathit{gc\_start}$).
Hence, every correct process that inputs to the $\mathit{gc\_end}$ primitive inputs bit $b$. 
Similarly, every correct process that outputs from $\mathit{gc\_end}$ outputs bit $b$ with grade $1$ (due to the validity property of $\mathit{gc\_end}$), which implies that no correct process sends an $\langle \textsc{echo}, \bar{b} \rangle$ message while executing $\mathcal{VC}(v' + 1)$, thus concluding the inductive step.
\end{proof}

Next, we prove a direct consequence of \Cref{lemma:decide_echo}.

\begin{lemma} \label{lemma:decide_validate}
If a correct process decides a bit $b$ in some view $v$ (i.e., while executing $\mathcal{VC}(v)$), then no correct process validates bit $\bar{b}$ in any view $v' > v$ (i.e., while executing $\mathcal{VC}(v')$).
\end{lemma}
\begin{proof}
For bit $\bar{b}$ to be validated in any view $v' > v$ (i.e., while executing $\mathcal{VC}(v')$), there must exist a correct process that sends an $\langle \textsc{echo}, \bar{b} \rangle$ message in $\mathcal{VC}(v' - 1)$.
As $v' > v$, $v' - 1 \geq v$.
According to \Cref{lemma:decide_echo}, no correct process sends an $\langle \textsc{echo}, \bar{b} \rangle$ message while executing $\mathcal{VC}(v^*)$, for any view $v^* \geq v$, which concludes the proof.
\end{proof}

The next lemma proves that, if all correct processes propose the same bit $b$ to the $\mathit{gc\_start}$ primitive of some view core instance, no process decides bit $\bar{b}$ in that view core instance.

\begin{lemma} \label{lemma:all_same_decision}
Consider $\mathcal{VC}(v)$, for some view $v$.
If all correct processes that input to the $\mathit{gc\_start}$ primitive in $\mathcal{VC}(v)$ input the same bit $b$, no correct process decides bit $\bar{b}$ while executing $\mathcal{VC}(v)$.
\end{lemma}
\begin{proof}
Due to the validity property of $\mathit{gc\_start}$, all correct processes that output do output bit $b$ from $\mathit{gc\_start}$.
Hence, all correct processes that input do input bit $b$ to the $\mathit{gc\_end}$ primitive.
Similarly, the validity property of $\mathit{gc\_end}$ ensures that all correct processes decide $b$ with grade $1$ from $\mathit{gc\_end}$.
Hence, no correct process decides $\bar{b}$ while executing $\mathcal{VC}(v)$.
\end{proof}

% \begin{lemma} \label{lemma:all_same_echo}
% Consider any view core instance $\mathcal{VC}(v)$, for some view $v$.
% If all correct processes that propose to the $\mathit{gc\_start}$ primitive in $\mathcal{VC}(v)$ propose the same bit $b$, no correct process.
% Then, no correct process sends a $\langle \textsc{echo}, v, \bar{b} \rangle$ message.
% \end{lemma}
% \begin{proof}
% Due to the validity property of the first graded consensus box, all correct processes that decide do decide $b$ from the first graded consensus box.
% Hence, all correct processes that propose do propose $b$ to the second graded consensus box.
% Again, the validity property ensures that all correct processes decide $b$ with grade $1$ from the second graded consensus box.
% Hence, no correct process sends a $\langle \textsc{echo}, v, \bar{b} \rangle$ message
% \end{proof}

We are now ready to prove the agreement property of \name.

\begin{lemma} [Agreement]
\name satisfies agreement.
\end{lemma}
\begin{proof}
Suppose that some correct process $p_i$ decides a bit $b$ in some view $v$ (i.e., while executing $\mathcal{VC}(v)$.
Moreover, suppose that some other correct process $p_j$ decides a bit $b'$ in some view $v'$ (i.e., while executing $\mathcal{VC}(v')$).
We consider two possibilities:
\begin{compactitem}
    \item Let $v = v'$.
    In this case, $b = b'$ due to the consistency property of the $\mathit{gc\_end}$ primitive.
    % second graded consensus box.

    \item Let $v \neq v'$.
    Without loss of generality, let $v < v'$.
    Due to \Cref{lemma:decide_validate}, all correct processes that input to the $\mathit{gc\_start}$ primitive of $\mathcal{VC}(v')$ do input bit $b$.
    Hence, \Cref{lemma:all_same_decision} implies that $b = b'$.
\end{compactitem}
The agreement property is satisfied as it holds in both possible cases.
\end{proof}

Lastly, we prove that \name satisfies validity.

\begin{lemma} [Validity]
\name satisfies validity.
\end{lemma}
\begin{proof}
Suppose that all correct processes propose the same bit $b$.
First, we prove that there exists a correct process that decides bit $b$ in the first view (i.e., while executing $\mathcal{VC}(1)$).

\medskip
\noindent \underline{\emph{Intermediate result.}} \emph{There exists a correct process that decides bit $b$ in view $1$ (i.e., while executing $\mathcal{VC}(1)$).}
\\ According to \Cref{lemma:finish_before_enter_next}, no correct process leaves view $1$ (i.e., enters another view) before at least one correct process $p_i$ has finished view $1$.
Moreover, every correct process outputs bit $b$ with grade $1$ from the $\mathit{gc\_start}$ primitive in $\mathcal{VC}(1)$ (due to the validity property of $\mathit{gc\_start}$).
Similarly, every correct process decides bit $b$ with grade $1$ from the $\mathit{gc\_end}$ primitive.
Hence, as $p_i$ has finished the first view, it has output bit $b$ with grade $1$ from $\mathit{gc\_end}$, which ensures that $p_i$ indeed decides bit $b$ in view $1$ at line~\ref{line:decide} of \Cref{algorithm:repeater_view_core}.

\medskip
\noindent \underline{\emph{Epilogue.}}
Due to the intermediate result, at least one correct process decides bit $b$ in the first view.
As \name satisfies agreement, no correct process decides bit $\bar{b}$, which proves that \name satisfies validity.
\end{proof}

\subsection{Proof of Complexity}

This subsection proves that \name exchanges $O(n \cdot \mathcal{PC} + n^2)$ messages, where $\mathcal{PC}$ denotes the per-process message complexity of the $\mathit{sync\_consensus}$ algorithm.
First, we prove that $\vfinal = \vmax + 1$.
Recall that $\vmax$ (resp., $\vfinal$) denotes the greatest (resp., smallest) view for which $t_{\vmax} < \text{GST}$ (resp., $t_{\vfinal} \geq \text{GST}$).

\begin{lemma} \label{lemma:vfinal_vmax}
$\vfinal = \vmax + 1$.
\end{lemma}
\begin{proof}
Follows directly from \Cref{lemma:view_previous_entered} and the definitions of views $\vmax$ (\Cref{definition:vmax}) and $\vfinal$ (\Cref{definition:vfinal}).
\end{proof}

The following lemma proves that correct processes enter monotonically increasing views.

\begin{lemma} \label{lemma:increasing_views}
Consider any correct process $p_i$.
Let $p_i$ enter some view $v_2$ after it has previously entered some view $v_1$.
Then, $v_1 < v_2$.
\end{lemma}
\begin{proof}
Process $p_i$ enters view $v_2$ at line~\ref{line:enter_v} (as it has previously entered view $v_1$).
According to \Cref{lemma:view_i_increases}, the value of the $\mathit{view}_i$ variable never decreases.
Therefore, $v_1 \leq v_2$.
It is left to prove that $v_1 \neq v_2$.

When $p_i$ enters view $v_1$ (line~\ref{line:enter_1} or line~\ref{line:enter_v}), the value of its $\mathit{view}_i$ variable is $v_1$.
Similarly, when $p_i$ enters view $v_2$ (must be done at line~\ref{line:enter_v}), the value of its $\mathit{view}_i$ variable is $v_2$.
Let $\mathit{Inv}_2$ denote the invocation of the $\mathsf{measure}(\delta)$ method on $\mathit{enter\_timer}_i$ (line~\ref{line:measure_enter}) that produces the expiration event which enables $p_i$ to enter view $v_2$.
Note that $p_i$ invokes $\mathit{Inv}_2$ before $p_i$ enters view $v_2$.
% Note that $\mathit{Inv}_2 \stackrel{\beta_i}{\prec} \mathsf{enter}(v_2)$.
We distinguish two possibilities:
\begin{compactitem}
    \item Let $p_i$ enter view $v_1$ at line~\ref{line:enter_1}.
    (This implies that $v_1 = 1$.)
    In this case, $p_i$ enters view $v_1$ before it invokes $\mathit{Inv}_2$.
    Hence, when $\mathit{Inv}_2$ is invoked, the value of the $\mathit{view}_i$ variable is greater than $v_1$ (due to the check at line~\ref{line:receive_quorum} and the assignment at line~\ref{line:update_view_2}).
    As the value of the $\mathit{view}_i$ variable never decreases (by \Cref{lemma:view_i_increases}), $v_1 < v_2$ in this case.

    \item Let $p_i$ enter view $v_1$ at line~\ref{line:enter_v}.
    Let $\mathit{Inv}_1$ denote the invocation of the $\mathsf{measure}(\delta)$ method on $\mathit{enter\_timer}_i$ (line~\ref{line:measure_enter}) that produces an expiration event which enables $p_i$ to enter view $v_1$.
    Let $\mathsf{enter}(v_1)$ (resp., $\mathsf{enter}(v_2)$) denote the event of $p_i$ entering view $v_1$ (resp., $v_2$).
    Finally, recall that $\beta_i$ denotes the behavior of process $p_i$.

    The following holds: $\mathit{Inv}_1 \stackrel{\beta_i}{\prec} \mathsf{enter}(v_1) \stackrel{\beta_i}{\prec} \mathsf{enter}(v_2)$.
    Moreover, $\mathsf{enter}(v_1) \stackrel{\beta_i}{\prec} \mathit{Inv}_2$.
    By contradiction, suppose that the previous claim is wrong, i.e., $\mathit{Inv}_2 \stackrel{\beta_i}{\prec} \mathsf{enter}(v_1)$.
    There are two cases to distinguish:
    \begin{compactitem}
        \item Let $\mathit{Inv}_1 \stackrel{\beta_i}{\prec} \mathit{Inv}_2 \stackrel{\beta_i}{\prec} \mathsf{enter}(v_1)$.
        This case conflicts with \Cref{lemma:enter_invocation_expiration}.

        \item Let $\mathit{Inv}_2 \stackrel{\beta_i}{\prec} \mathit{Inv}_1 \stackrel{\beta_i}{\prec} \mathsf{enter}(v_1)$.
        This case also conflicts with \Cref{lemma:enter_invocation_expiration}.
    \end{compactitem}
    Therefore, $\mathsf{enter}(v_1) \stackrel{\beta_i}{\prec} \mathit{Inv}_2$.
    Hence, when $\mathit{Inv}_2$ is invoked, the value of the $\mathit{view}_i$ variable is greater than $v_1$ (due to the check at line~\ref{line:receive_quorum} and the assignment at line~\ref{line:update_view_2}).
    As the value of the $\mathit{view}_i$ variable never decreases (according to \Cref{lemma:view_i_increases}), $v_1 < v_2$ in this case.
\end{compactitem}
In both possible cases, $v_1 < v_2$, which concludes the proof.
\end{proof}

Next, we prove that all correct processes broadcast a $\langle \textsc{start-view}, \vmax \rangle$ message by time $\text{GST} + 3\delta$ (if $\vmax > 1$).

\begin{lemma} \label{lemma:vmax_all_broadcast}
If $\vmax > 1$, every correct process broadcasts a $\langle \textsc{start-view}, \vmax \rangle$ message by time $\text{GST} + 3\delta$.
\end{lemma}
\begin{proof}
First, \Cref{lemma:vfinal_vmax} ensures that $\vfinal > 2$ (as $\vfinal = \vmax + 1$ and $\vmax > 1$).
According to \Cref{lemma:update_view_time}, no correct process $p_i$ updates its $\mathit{view}_i$ variable to a view greater than $\vfinal$ before time $t_{\vfinal} + \mathit{view\_duration} \geq \text{GST} + \mathit{view\_duration}$.
Similarly, \Cref{lemma:update_help_view_time} proves that no correct process $p_i$ updates its $\mathit{help\_view}_i$ variable to a view greater than $\vfinal$ before time $t_{\vfinal} + \mathit{view\_duration} \geq \text{GST} + \mathit{view\_duration}$.
As some correct process enters view $\vmax > 1$ before GST, every correct process $p_i$ receives $t + 1$ $\langle 
\textsc{start-view}, \vmax \rangle$ messages at some time $t^* \leq \text{GST} + \delta$.
Note that $\mathit{view\_duration} > \delta$.
The following holds at process $p_i$ at time $t^* \leq \text{GST} + \delta < \text{GST} + \mathit{view\_duration}$: (1) $\mathit{view}_i \in \{\vmax, \vfinal\}$ (if the rule at line~\ref{line:receive_plurality} does not activate at time $t^*$), or (2) $\mathit{help\_view}_i \in \{\vmax, \vfinal\}$ (if the rule at line~\ref{line:receive_plurality} activates at time $t^*$).
Let us consider both scenarios:
\begin{compactitem}
    \item Let $\mathit{view}_i \in \{\vmax, \vfinal\}$ at time $t^*$.
    We further distinguish two scenarios:
    \begin{compactitem}
        \item Let $\mathit{view}_i = \vfinal$.
        When $p_i$ updated $\mathit{view}_i$ to $\vfinal > 2$ (line~\ref{line:update_view_2}), $p_i$ invoked the $\mathsf{measure}(\delta)$ method on $\mathit{enter\_view}_i$ timer (line~\ref{line:measure_enter}).
        This invocation cannot be canceled as $p_i$ does not update its $\mathit{view}_i$ variable to a view greater than $\vfinal$ before time $t_{\vfinal} + \mathit{view\_duration} \geq \text{GST} + \mathit{view\_duration} > \text{GST} + 2\delta$ (by \Cref{lemma:update_view_time}).
        Therefore, when the aforementioned invocation expires (line~\ref{line:enter_expires}), which happens by time $t^* + \delta \leq \text{GST} + 2\delta$, $p_i$ enters $\vfinal$ (line~\ref{line:enter_v}) and broadcasts a \textsc{start-view} message for both $\vfinal$ (line~\ref{line:send_complete_3}) and $\vmax$ (line~\ref{line:send_complete_3_prime}).
        % The statement of the lemma holds in this case.

        \item Let $\mathit{view}_i = \vmax$.
        When $p_i$ updated $\mathit{view}_i$ to $\vmax > 1$ (line~\ref{line:update_view_2}), $p_i$ invoked the $\mathsf{measure}(\delta)$ method on $\mathit{enter\_view}_i$ timer (line~\ref{line:measure_enter}).
        If this invocation does not get canceled, $p_i$ enters $\vmax$ (line~\ref{line:enter_v}) by time $t^* + \delta \leq \text{GST} + 2\delta$ and broadcasts a \textsc{start-view} message for $\vmax$ (line~\ref{line:send_complete_3}).

        Otherwise, as $p_i$ must cancel the invocation by time $t^* + \delta \leq \text{GST} + 2\delta$, $p_i$ sets its $\mathit{view}_i$ variable to $\vfinal$ (line~\ref{line:update_view_2}).
        (Recall that \Cref{lemma:update_view_time} guarantees that $p_i$ cannot update its $\mathit{view}_i$ variable to a view greater than $\vfinal$ before time $t_{\vfinal} + \mathit{view\_duration} \geq \text{GST} + \mathit{view\_duration} > \text{GST} + 2\delta$.)
        Importantly, this invocation cannot be canceled.
        Therefore, when the invocation expires (by time $t^* + 2\delta \leq \text{GST} + 3\delta$), $p_i$ enters view $\vfinal$ and broadcasts a $\langle \textsc{start-view}, \vmax \rangle$ message at line~\ref{line:send_complete_3_prime}.
    \end{compactitem}

    \item Let $\mathit{help\_view}_i \in \{\vmax, \vfinal\}$ at time $t^*$.
    % $\text{GST} + \delta$.
    We further distinguish two scenarios:
    \begin{compactitem}
        \item Let $\mathit{help\_view}_i = \vfinal$.
        When $p_i$ updated $\mathit{help\_view}_i$ to $\vfinal > 2$ (line~\ref{line:update_help_view}), it invoked the $\mathsf{measure}(\delta)$ method on $\mathit{help\_view}_i$ timer (line~\ref{line:measure_help}).
        This invocation cannot be canceled as $p_i$ does not update its $\mathit{help\_view}_i$ variable to a view greater than $\vfinal$ before time $t_{\vfinal} + \mathit{view\_duration} \geq \text{GST} + \mathit{view\_duration} > \text{GST} + 2\delta$ (by \Cref{lemma:update_help_view_time}).
        Therefore, when the aforementioned invocation expires (line~\ref{line:help_timer_expires}), which happens by time $t^* + \delta \leq \text{GST} + 2\delta$, $p_i$ broadcasts a \textsc{start-view} message for $\vmax$ at line~\ref{line:send_complete_2_prime}.

        \item Let $\mathit{help\_view}_i = \vmax$.
        When $p_i$ updated $\mathit{help\_view}_i$ to $\vmax$ (line~\ref{line:update_help_view}), it invoked the $\mathsf{measure}(\delta)$ method on $\mathit{help\_view}_i$ timer (line~\ref{line:help_timer_expires}).
        If this invocation does not get canceled, $p_i$ broadcasts a \textsc{start-view} message for $\vmax$ at line~\ref{line:send_complete_2} by time $t^* + \delta \leq \text{GST} + 2\delta$.

        Otherwise, as $p_i$ must cancel the invocation by time $t^* + \delta \leq \text{GST} + 2\delta$, $p_i$ sets its $\mathit{help\_view}_i$ variable to $\vfinal$ (line~\ref{line:update_view_2}).
        (Recall that \Cref{lemma:update_help_view_time} guarantees that $p_i$ cannot update its $\mathit{help\_view}_i$ variable to a view greater than $\vfinal$ before time $t_{\vfinal} + \mathit{view\_duration} \geq \text{GST} + \mathit{view\_duration} > \text{GST} + 2\delta$.)
        Importantly, this invocation cannot be canceled.
        Therefore, when the invocation expires (by time $t^* + 2\delta \leq \text{GST} + 3\delta$), $p_i$ broadcasts a $\langle \textsc{start-view}, \vmax \rangle$ at line~\ref{line:send_complete_2_prime}.
    \end{compactitem}
\end{compactitem}
In any possible case, $p_i$ broadcasts a $\langle \textsc{start-view}, \vmax \rangle$ message by time $\text{GST} + 3\delta$, which concludes the proof.
\end{proof}

The following lemma proves that every correct process enters view $\vmax$ or $\vfinal$ by time $\text{GST} + 6\delta$.

\begin{lemma} \label{lemma:enter_vmax_vfinal}
Every correct process enters view $\vmax$ or $\vfinal = \vmax + 1$ by time $\text{GST} + 6\delta$.
\end{lemma}
\begin{proof}
If $\vmax = 1$ (resp., $\vfinal = 1$), every correct process enters $\vmax$ (resp., $\vfinal$) at line~\ref{line:enter_1} before (resp., at) time GST, which concludes the lemma.
Hence, let $\vmax > 1$.
(According to \Cref{lemma:vfinal_vmax}, this implies that $\vfinal > 1$.)

Consider any correct process $p_i$.
By \Cref{lemma:vmax_all_broadcast}, every correct process broadcasts a $\langle \textsc{start-view}, \vmax \rangle$ message by time $\text{GST} + 3\delta$.
Hence, by some time $t^* \leq \text{GST} + 4\delta$, $p_i$ receives $2t + 1$ $\langle \textsc{start-view}, \vmax \rangle$ messages.
Moreover, note that process $p_i$ cannot update its $\mathit{view}_i$ variable to a view greater than $\vfinal$ before time $t_{\vfinal} + \mathit{view\_duration} \geq \text{GST} + \mathit{view\_duration} > \text{GST} + 4\delta$.
Therefore, the following holds at process $p_i$ at time $t^* \leq \text{GST} + 4\delta$: $\mathit{view}_i \in \{\vmax, \vfinal\}$.
Let us consider both possible scenarios:
\begin{compactitem}
    \item Let $\mathit{view}_i = \vfinal$.
    When $p_i$ updated $\mathit{view}_i$ to $\vfinal$ (line~\ref{line:update_view_2}), $p_i$ invoked the $\mathsf{measure}(\delta)$ method on $\mathit{enter\_view}_i$ timer (line~\ref{line:measure_enter}).
    This invocation cannot be canceled as $p_i$ does not update its $\mathit{view}_i$ variable to a view greater than $\vfinal$ before time $t_{\vfinal} + \mathit{view\_duration} \geq \text{GST} + \mathit{view\_duration} > \text{GST} + 5\delta$ (by \Cref{lemma:update_view_time}).
    Therefore, when the aforementioned invocation expires (line~\ref{line:enter_expires}), which happens by time $t^* + \delta \leq \text{GST} + 5\delta$, $p_i$ enters $\vfinal$ (line~\ref{line:enter_v}).

    \item Let $\mathit{view}_i = \vmax$.
    When $p_i$ updated $\mathit{view}_i$ to $\vmax > 1$ (line~\ref{line:update_view_2}), $p_i$ invoked the $\mathsf{measure}(\delta)$ method on $\mathit{enter\_view}_i$ timer (line~\ref{line:measure_enter}).
    If this invocation does not get canceled, $p_i$ enters $\vmax$ (line~\ref{line:enter_v}) by time $t^* + \delta \leq \text{GST} + 5\delta$ and enters view $\vmax$ (line~\ref{line:enter_v}).

    Otherwise, as $p_i$ must cancel the invocation by time $t^* + \delta \leq \text{GST} + 5\delta$, $p_i$ sets its $\mathit{view}_i$ variable to $\vfinal$ (line~\ref{line:update_view_2}).
    (Recall that \Cref{lemma:update_view_time} guarantees that $p_i$ cannot update its $\mathit{view}_i$ variable to a view greater than $\vfinal$ before time $t_{\vfinal} + \mathit{view\_duration} \geq \text{GST} + \mathit{view\_duration} > \text{GST} + 5\delta$.)
    Importantly, this invocation cannot be canceled.
    Therefore, when the invocation expires (by time $t^* + 2\delta \leq \text{GST} + 6\delta$), $p_i$ enters view $\vfinal$ (line~\ref{line:enter_v}).
\end{compactitem}
The statement of the lemma holds in both possible scenarios, which concludes the proof.
\end{proof}

To prove the message complexity of \name, we first consider the number of messages correct processes send during the unsynchronized time period $[\text{GST}, \text{GST} + 6\delta]$.
First, we prove that, if a correct process broadcasts a $\langle \textsc{start-view}, v \rangle$ message at line~\ref{line:send_complete_1}, then $v - 1$ is the last view entered by that process before sending the \textsc{start-view} message.

% First, we prove that each correct process broadcasts at most one \textsc{start-view} message at line~\ref{line:send_complete_1} during the unsynchronized time period.

\begin{lemma} \label{lemma:start_view_last_entered}
Consider any correct process $p_i$ that broadcasts a $\langle \textsc{start-view}, v \rangle$ message at line~\ref{line:send_complete_1}.
Then, view $v - 1$ is the last view entered by $p_i$ before sending the \textsc{start-view} message.
\end{lemma}
\begin{proof}
Let $s_m$ denote the $p_i$'s event of broadcasting the $\langle \textsc{start-view}, v \rangle$ message at line~\ref{line:send_complete_1}.
As $p_i$ sends the \textsc{start-view} message upon processing the $\mathsf{finished}()$ indication triggered by $\mathcal{VC}(v - 1)$ (line~\ref{line:view_timer_expire}), $\mathcal{VC}(v - 1).\mathsf{start()} \stackrel{\beta_i}{\prec} s_m$.
(Recall that $\beta_i$ denotes the behavior of process $p_i$.)

By contradiction, let $v'$ denote a view such that (1) $\mathcal{VC}(v - 1).\mathsf{start}() \stackrel{\beta_i}{\prec} \mathcal{VC}(v').\mathsf{start}() \stackrel{\beta_i}{\prec} s_m$, and (2) no view $v''$ exists with $\mathcal{VC}(v - 1).\mathsf{start}() \stackrel{\beta_i}{\prec} \mathcal{VC}(v'').\mathsf{start()} \stackrel{\beta_i}{\prec} \mathcal{VC}(v').\mathsf{start}()$.
Immediately before invoking $\mathcal{VC}(v').\mathsf{start}()$ (line~\ref{line:enter_v}), $p_i$ invokes $\mathcal{VC}(v - 1).\mathsf{stop()}$ at line~\ref{line:leave_v}.
Due to \Cref{lemma:increasing_views}, $p_i$ never invokes the $\mathsf{start()}$ operation on $\mathcal{VC}(v - 1)$ such that $\mathcal{VC}(v').\mathsf{start()} \stackrel{\beta_i}{\prec} \mathcal{VC}(v - 1).\mathsf{start()}$.
However, we reach a contradiction with the fact that $\mathcal{VC}(v - 1)$ triggers the $\mathsf{finished()}$ event, which concludes the proof of the lemma.
\end{proof}

The following lemma proves that any correct process broadcasts at most one \textsc{start-view} message at line~\ref{line:send_complete_1} during the unsynchronized period $[\text{GST}, \text{GST} + 6\delta]$.

\begin{lemma} \label{lemma:unsynchronized_period_1}
Any correct process broadcasts at most one \textsc{start-view} message at line~\ref{line:send_complete_1} during the $[\text{GST}, \text{GST} + 6\delta]$ time period.
\end{lemma}
\begin{proof}
Consider any correct process $p_i$.
% To prove the lemma, we prove that at least $6\delta$ time must elapse between any two broadcasting events at line~\ref{line:send_complete_1} that occur at or after GST.
Let $m_1 = \langle \textsc{start-view}, v_1 \rangle$ be a message that $p_i$ broadcasts at line~\ref{line:send_complete_1} at some time $t_1 \in [\text{GST}, \text{GST} + 6\delta]$.
Moreover, let $m_2 = \langle \textsc{start-view}, v_2 \rangle$ be another message that $p_i$ broadcasts at line~\ref{line:send_complete_1} after broadcasting $m_1$; let $m_2$ be broadcast at some time $t_2$.
To prove the lemma, we show that $t_2 > \text{GST} + 6\delta$.

We denote by $s_{m_1}$ (resp., $s_{m_2}$) the $p_i$'s event of sending the message $m_1$ (resp., $m_2$).
As $s_{m_1}$ is sent upon $\mathcal{VC}(v_1 - 1)$ triggers the $\mathsf{finished()}$ invocation, the following holds: $\mathcal{VC}(v_1 - 1).\mathsf{start()} \stackrel{\beta_i}{\prec} s_{m_1}$.
(Recall that $\beta_i$ denotes the behavior of process $p_i$.)
Similarly, $\mathcal{VC}(v_2 - 1).\mathsf{start()} \stackrel{\beta_i}{\prec} s_{m_2}$.
Moreover, $s_{m_1} \stackrel{\beta_i}{\prec} s_{m_2}$.
Finally, by \Cref{lemma:start_view_last_entered}, the following holds: $\mathcal{VC}(v_1 - 1).\mathsf{start()} \stackrel{\beta_i}{\prec} s_{m_1} \stackrel{\beta_i}{\prec} \mathcal{VC}(v_2 - 1).\mathsf{start()} \stackrel{\beta_i}{\prec} s_{m_2}$.

As $m_1$ is sent during the time period $[\text{GST}, \text{GST} + 6\delta]$, $\mathcal{VC}(v_2 - 1).\mathsf{start()}$ is invoked at or after GST.
As the local clock of $p_i$ does not drift after GST, $t_2 \geq \text{GST} + \mathit{view\_duration} > \text{GST} + 6\delta$ (see \Cref{algorithm:repeater_view_core}).
Therefore, the lemma holds.
\end{proof}

Next, we prove that the rule at line~\ref{line:help_timer_expires} activates at any correct process $O(1)$ times during the unsynchronized time period $[\text{GST}, \text{GST} + 6\delta]$.

\begin{lemma} \label{lemma:unsynchronized_period_2}
The rule at line~\ref{line:help_timer_expires} activates at any correct process $O(1)$ times during the $[\text{GST}, \text{GST} + 6\delta]$ time period.
\end{lemma}
\begin{proof}
To prove the lemma, we prove that any two activations of the rule at or after GST must be separated by at least $\delta$ time.
Let $p_i$ be any correct process.
Let $\mathit{Exp}_h^1$ denote any expiration event of $\mathit{help\_timer}_i$ that occurs at some time $t_1 \in [\text{GST}, \text{GST} + 6\delta]$.
Moreover, let $\mathit{Exp}_h^2$ denote the first expiration event of $\mathit{help\_timer}_i$ that follows $\mathit{Exp}_h^1$ in $h_i|_{\mathit{help}}$; let $\mathit{Exp}_h^2$ occur at some time $t_2 \geq t_1$.
Let $\mathit{Inv}_h^2$ denote the invocation of the $\mathsf{measure}(\delta)$ method (line~\ref{line:measure_help}) that produces $\mathit{Exp}_h^2$; note that $\mathit{Inv}_h^2 \stackrel{\beta_i}{\prec} \mathit{Exp}_h^2$.
Moreover, \Cref{lemma:help_invocation_expiration} proves that $\mathit{Exp}_h^1 \stackrel{\beta_i}{\prec} \mathit{Inv}_h^2 \stackrel{\beta_i}{\prec} \mathit{Exp}_h^2$.
As $t_1 \geq \text{GST}$, $\mathit{Inv}_h^2$ occurs at some time $t_2' \geq t_1 \geq \text{GST}$.
Finally, as the local clock of $p_i$ does not drift after GST, $t_2 - t_2' = \delta$.
Therefore, $t_2 - t_1 \geq \delta$, which proves the lemma.
\end{proof}

Next, we prove that the rule at line~\ref{line:enter_expires} activates at any correct process $O(1)$ times during the unsynchronized time period $[\text{GST}, \text{GST} + 6\delta]$.

\begin{lemma} \label{lemma:unsynchronized_period_3}
The rule at line~\ref{line:enter_expires} activates at any correct process $O(1)$ times during the $[\text{GST}, \text{GST} + 6\delta]$ time period.
\end{lemma}
\begin{proof}
To prove the lemma, we follow the strategy used in proving \Cref{lemma:unsynchronized_period_2}.
Namely, we prove that any two activations of the rule at or after GST must be separated by at least $\delta$ time.
Let $p_i$ be any correct process.
Let $\mathit{Exp}_e^1$ denote any expiration event of $\mathit{enter\_timer}_i$ that occurs at some time $t_1 \in [\text{GST}, \text{GST} + 6\delta]$.
Moreover, let $\mathit{Exp}_e^2$ denote the first expiration event of $\mathit{enter\_timer}_i$ that follows $\mathit{Exp}_e^1$ in $h_i|_{\mathit{enter}}$; let $\mathit{Exp}_e^2$ occur at some time $t_2 \geq t_1$.
Let $\mathit{Inv}_e^2$ denote the invocation of the $\mathsf{measure}(\delta)$ method (line~\ref{line:measure_enter}) that produces $\mathit{Exp}_e^2$; note that $\mathit{Inv}_e^2 \stackrel{\beta_i}{\prec} \mathit{Exp}_e^2$.
Moreover, \Cref{lemma:enter_invocation_expiration} proves that $\mathit{Exp}_e^1 \stackrel{\beta_i}{\prec} \mathit{Inv}_e^2 \stackrel{\beta_i}{\prec} \mathit{Exp}_e^2$.
As $t_1 \geq \text{GST}$, $\mathit{Inv}_e^2$ occurs at some time $t_2' \geq t_1 \geq \text{GST}$.
Finally, as the local clock of $p_i$ does not drift after GST, $t_2 - t_2' = \delta$.
Therefore, $t_2 - t_1 \geq \delta$, which proves the lemma.
\end{proof}

The next lemma proves that any correct process sends $O(\mathcal{PC} + n)$ messages while executing any view core abstraction.

\begin{lemma} \label{lemma:message_complexity_view_core}
Consider any correct process $p_i$, and any view $v$.
Process $p_i$ sends $O(\mathcal{PC} + n)$ messages while executing $\mathcal{VC}(v)$.
\end{lemma}
\begin{proof}
Process $p_i$ sends $O(n)$ messages while executing the AW graded consensus algorithm (by~\cite{AttiyaWelch23}).
Moreover, process $p_i$ sends at most $\mathcal{PC}$ messages while executing the $\mathit{sync\_consensus}$ primitive.
Lastly, $p_i$ sends $O(n)$ messages while executing the ``\textsc{echo}'' step of $\mathcal{VC}(v)$.
Therefore, $p_i$ indeed sends $O(\mathcal{PC} + n)$ messages while executing $\mathcal{VC}(v)$.
\end{proof}

Finally, we are ready to prove that any correct process sends $O(\mathcal{PC} + n)$ messages during the unsynchronized time period $[\text{GST}, \text{GST} + 6\delta]$.

\begin{lemma} \label{lemma:final_unsynchronized}
Any correct process sends $O(\mathcal{PC} + n)$ messages during the $[\text{GST}, \text{GST} + 6\delta]$ time period.
\end{lemma}
\begin{proof}
Consider any correct process $p_i$.
Let us first count the number of \textsc{start-view} messages $p_i$ sends. during the $[\text{GST}, \text{GST} + 6\delta]$ time period.
According to \Cref{lemma:unsynchronized_period_1}, $p_i$ broadcasts at most one \textsc{start-view} message at line~\ref{line:send_complete_1}.
\Cref{lemma:unsynchronized_period_2} proves that $p_i$ broadcasts at most $O(1)$ \textsc{start-view} messages at lines~\ref{line:send_complete_2} and~\ref{line:send_complete_2_prime}.
Similarly, \Cref{lemma:unsynchronized_period_3} states that $p_i$ broadcasts at most $O(1)$ \textsc{start-view} messages at line~\ref{line:send_complete_3} and~\ref{line:send_complete_3_prime}.
Therefore, $p_i$ sends 
\begin{equation*}
    \underbrace{1 \cdot n}_\text{line~\ref{line:send_complete_1}} + \underbrace{O(1) \cdot n}_\text{lines~\ref{line:send_complete_2} and~\ref{line:send_complete_2_prime}} + \underbrace{O(1) \cdot n}_\text{lines~\ref{line:send_complete_3} and~\ref{line:send_complete_3_prime}} = O(n) \text{ \textsc{start-view} messages during the } [\text{GST}, \text{GST} + 6\delta] \text{ time period.}
\end{equation*}

Lastly, we count the number of messages associated with the view core abstraction that $p_i$ sends during the $[\text{GST}, \text{GST} + 6\delta]$ time period.
According to \Cref{lemma:unsynchronized_period_3}, $p_i$ enters $O(1)$ views during the aforementioned time period.
As $p_i$ sends $O(\mathcal{PC} + n)$ messages while executing any view core abstraction (by \Cref{lemma:message_complexity_view_core}), $p_i$ sends $O(1) \cdot O(\mathcal{PC} + n) = O(\mathcal{PC} + n)$ messages associated with the view core abstraction.
Thus, the total number of messages $p_i$ sends during the $[\text{GST}, \text{GST} + 6\delta]$ time period is
\begin{equation*}
    \underbrace{O(n)}_\text{\textsc{start-view} messages} + \underbrace{O(\mathcal{PC} + n)}_\text{view core} = O(\mathcal{PC} + n).
\end{equation*}
\end{proof}

We now prove that any correct process broadcasts at most two \textsc{start-view} messages at line~\ref{line:send_complete_1} during the synchronized period $[\text{GST} + 6\delta, t_{\vfinal} + \mathit{view\_duration}]$.
Recall that all correct processes decide from \name by time $t_{\vfinal} + \mathit{view\_duration}$ (by \Cref{lemma:repeater_termination}).

\begin{lemma} \label{lemma:synchronized_1}
Any correct process broadcasts at most two \textsc{start-view} messages at line~\ref{line:send_complete_1} during the $[\text{GST} + 6\delta, t_{\vfinal} + \mathit{view\_duration}]$ time period.
\end{lemma}
\begin{proof}
According to \Cref{lemma:enter_vmax_vfinal}, any correct process $p_i$ enters view $\vmax$ or $\vfinal$ by time $\text{GST} + 6\delta$.
Moreover, \Cref{lemma:vfinal_end} proves that $p_i$ does not enter a view greater than $\vfinal$ before time $t_{\vfinal} + \mathit{view\_duration}$.
Finally, \Cref{lemma:increasing_views} shows that $p_i$ enters at most two views (i.e., $\vmax$ and $\vfinal$) during the $[\text{GST} + 6\delta, t_{\vfinal} + \mathit{view\_duration}]$ time period.

Let us consider any message $m = \langle \textsc{start-view}, v' > 1 \rangle$ broadcast by $p_i$ at line~\ref{line:send_complete_1} after $p_i$ has entered view $\vmax$ or $\vfinal$ (which happens by time $\text{GST} + 6\delta$).
Due to \Cref{lemma:start_view_last_entered}, $v' - 1$ is the last view entered by $p_i$ before sending message $m$.
As $p_i$ enters at most two views during the $[\text{GST} + 6\delta, t_{\vfinal} + \mathit{view\_duration}]$ time period, $p_i$ broadcasts at most two messages at line~\ref{line:send_complete_1}, which completes the proof.
\end{proof}

Next, we prove that the rule at line~\ref{line:help_timer_expires} activates $O(1)$ times at any correct process during the synchronized time period $[\text{GST} + 6\delta, t_{\vfinal} + \mathit{view\_duration}]$.

\begin{lemma} \label{lemma:synchronized_2}
The rule at line~\ref{line:help_timer_expires} activates at any correct process $O(1)$ times during the $[\text{GST} + 6\delta, t_{\vfinal} + \mathit{view\_duration}]$ time period.
\end{lemma}
\begin{proof}
According to \Cref{lemma:enter_vmax_vfinal}, any correct process $p_i$ enters view $\vmax$ or $\vfinal$ by time $\text{GST} + 6\delta$.
Hence, at time $\text{GST} + 6\delta$, the value of the $\mathit{view}_i$ variable is $\geq \vmax$.
According to \Cref{lemma:update_view_time}, $p_i$ does not update its $\mathit{view}_i$ variable to a view greater than $\vfinal$ before time $t_{\vfinal} + \mathit{view\_duration}$.
Finally, as the value of the $\mathit{view}_i$ variable never decreases (by \Cref{lemma:view_i_increases}), the value of the $\mathit{view}_i$ variable can either be $\vmax$ or $\vfinal$ throughout the $[\text{GST} + 6\delta, t_{\vfinal} + \mathit{view\_duration}]$ time period.

Let us consider the first time $p_i$ invokes the $\mathsf{measure}(\delta)$ method on $\mathit{help\_timer}_i$ (line~\ref{line:measure_help}) after $p_i$ has entered view $\vmax$ or $\vfinal$ (which happens by time $\text{GST} + 6\delta$).
Before invoking the $\mathsf{measure}(\delta)$ method (line~\ref{line:measure_help}), $p_i$ has updated its $\mathit{help\_view}_i$ variable to some view $v^*$.
According to \Cref{lemma:update_help_view_time}, $v^* \leq \vfinal$.
Moreover, $v^*$ is greater than the value of the $\mathit{view}_i$ variable (according to the check at line~\ref{line:receive_plurality}); recall that the value of the $\mathit{view}_i$ variable at this point is $\vmax$ or $\vfinal$.
Hence, $v^*$ must be equal to $\vfinal$, whereas the value of the $\mathit{view}_i$ variable must be equal to $\vmax$.
Lastly, due to the check at line~\ref{line:check_help}, the aforementioned scenario cannot be repeated.
In other words, process $p_i$ invokes the $\mathsf{measure}(\delta)$ method on $\mathit{help\_timer}_i$ at most once after $p_i$ has entered view $\vmax$ or $\vfinal$; let us denote this invocation of the $\mathsf{measure}(\delta)$ method by $\mathit{Inv}_h$.

It is left to prove that only one expiration event $\mathit{Exp}_h$ of $\mathit{help\_timer}_i$ exists such that (1) $\mathit{Exp}_h$ occurs after $p_i$ has entered view $\vmax$ or $\vfinal$, and (2) $\mathit{Exp}_h \stackrel{\beta_i}{\prec} \mathit{Inv}_h$.
(Recall that $\beta_i$ denotes the behavior of process $p_i$.)
There cannot be multiple expiration events of $\mathit{help\_timer}_i$ that satisfy the aforementioned description due to \Cref{lemma:help_invocation_expiration}.
Thus, the rule at line~\ref{line:help_timer_expires} can be activated at process $p_i$ at most $2 = O(1)$ times during the $[\text{GST} + 6\delta, t_{\vfinal} + \mathit{view\_duration}]$ time period: once before $\mathit{Inv}_h$ has been invoked, and once due to the $\mathit{Inv}_h$ invocation.
\end{proof}

The following lemma proves that the rule at line~\ref{line:enter_expires} activates at any correct process $O(1)$ times during the $[\text{GST} + 6\delta, t_{\vfinal} + \mathit{view\_duration}]$ time period.

\begin{lemma} \label{lemma:synchronized_3}
The rule at line~\ref{line:enter_expires} activates at any correct process $O(1)$ times during the $[\text{GST} + 6\delta, t_{\vfinal} + \mathit{view\_duration}]$ time period.
\end{lemma}
\begin{proof}
According to \Cref{lemma:enter_vmax_vfinal}, any correct process $p_i$ enters view $\vmax$ of $\vfinal$ by time $\text{GST} + 6\delta$.
\Cref{lemma:vfinal_end} proves that $p_i$ does not enter any view greater than $\vfinal$ before time $t_{\vfinal} + \mathit{view\_duration}$.
Finally, \Cref{lemma:increasing_views} proves that $p_i$ can only enter two views (i.e., $\vmax$ and $\vfinal$) during the $[\text{GST} + 6\delta, t_{\vfinal} + \mathit{view\_duration}]$ time period.
Therefore, the lemma holds.
\end{proof}

Finally, we prove that any correct process sends $O(\mathcal{PC} + n)$ messages during the synchronized time period $[\text{GST} + 6\delta, t_{\vfinal} + \mathit{view\_duration}]$.

\begin{lemma} \label{lemma:final_synchronized}
Any correct process sends $O(\mathcal{PC} + n)$ messages during the $[\text{GST} + 6\delta, t_{\vfinal} + \mathit{view\_duration}]$ time period.
\end{lemma}
\begin{proof}
Consider any correct process $p_i$.
Let us first count the number of \textsc{start-view} messages $p_i$ sends. during the $[\text{GST} + 6\delta, t_{\vfinal} + \mathit{view\_duration}]$ time period.
According to \Cref{lemma:synchronized_1}, $p_i$ broadcasts at most two \textsc{start-view} messages at line~\ref{line:send_complete_1}.
\Cref{lemma:synchronized_2} proves that $p_i$ broadcasts at most $O(1)$ \textsc{start-view} messages at lines~\ref{line:send_complete_2} and~\ref{line:send_complete_2_prime}.
Similarly, \Cref{lemma:synchronized_3} states that $p_i$ broadcasts at most $O(1)$ \textsc{start-view} messages at line~\ref{line:send_complete_3} and~\ref{line:send_complete_3_prime}.
Therefore, $p_i$ sends 
\begin{equation*}
    \underbrace{2 \cdot n}_\text{line~\ref{line:send_complete_1}} + \underbrace{O(1) \cdot n}_\text{lines~\ref{line:send_complete_2} and~\ref{line:send_complete_2_prime}} + \underbrace{O(1) \cdot n}_\text{lines~\ref{line:send_complete_3} and~\ref{line:send_complete_3_prime}} = O(n) \text{ \textsc{start-view} messages during the } [\text{GST} + 6\delta, t_{\vfinal} + \mathit{view\_duration}] \text{ time period.}
\end{equation*}

Lastly, we count the number of messages associated with the view core abstraction that $p_i$ sends during the $[\text{GST} + 6\delta, t_{\vfinal} + \mathit{view\_duration}]$ time period.
According to \Cref{lemma:synchronized_3}, $p_i$ enters $O(1)$ views during the aforementioned time period.
As $p_i$ sends $O(\mathcal{PC} + n)$ messages while executing any view core abstraction (by \Cref{lemma:message_complexity_view_core}), $p_i$ sends $O(1) \cdot O(\mathcal{PC} + n) = O(\mathcal{PC} + n)$ messages associated with the view core abstraction.
Thus, the total number of messages $p_i$ sends during the $[\text{GST} + 6\delta, t_{\vfinal} + \mathit{view\_duration}]$ time period is
\begin{equation*}
    \underbrace{O(n)}_\text{\textsc{start-view} messages} + \underbrace{O(\mathcal{PC} + n)}_\text{view core} = O(\mathcal{PC} + n).
\end{equation*}
\end{proof}

The following lemma proves the $O(n \cdot \mathcal{PC} + n^2)$ message complexity of \name.

\begin{lemma} [Message complexity]
\name achieves $O(n \cdot \mathcal{PC} + n^2)$ message complexity.
\end{lemma}
\begin{proof}
Consider any correct process $p_i$.
Process $p_i$ sends $O(\mathcal{PC} + n)$ messages during the unsynchronized time period $[\text{GST}, \text{GST} + 6\delta]$ (by \Cref{lemma:final_unsynchronized}).
Similarly, $p_i$ sends $O(\mathcal{PC} + n)$ messages during the synchronized time period $[\text{GST} + 6\delta, t_{\vfinal} + \mathit{view\_duration}]$ (by \Cref{lemma:final_synchronized}).
Therefore, $p_i$ sends $O(\mathcal{PC} + n)$ messages during the time period $[\text{GST}, t_{\vfinal} + \mathit{view\_duration}]$, which implies that the total message complexity of \name is $O(n \cdot \mathcal{PC} + n^2)$.
\end{proof}
