# Supplementary material for: Partial Synchrony for Free? New Upper Bounds for Byzantine Agreement
Source: arXiv:2402.10059 source file (2024-10-23)
Supplement: Supplementary file 13 [file triviality.tex]

\newpage
\section{Triviality of Solvable Validity Properties if $n \leq 3t$: Formal Proof} \label{section:triviality_appendix}

In this section, we give formal proofs of the intermediate results from \Cref{subsection:triviality_main}.
First, we formally prove that only $v_{\mathit{base}}$ can be decided in any canonical execution which corresponds to any input configuration compatible with $\mathit{base}$.

\begin{lemma_1_triviality} [restated]
Let $c \in \mathcal{I}$ be any input configuration such that $c \diamond \mathit{base}$.
Let $\mathcal{E}_c \in \mathit{execs}(\mathcal{A})$ be any canonical execution such that $\mathsf{input\_conf}(\mathcal{E}_c) = c$.
If a value $v_c \in \mathcal{V}_O$ is decided by a correct process in $\mathcal{E}_c$, then $v_c = v_{\mathit{base}}$.
\end{lemma_1_triviality}
\begin{proof}
By contradiction, suppose that some value $v_c \neq v_{\mathit{base}}$ is decided by a correct process in $\mathcal{E}_c$.
Since $c \diamond \mathit{base}$, there exists a correct process $Q \in \processes{c}\setminus{\processes{\mathit{base}}}$.
Let $\mathcal{E}_c^Q$ be an infinite \add{canonical} continuation of $\mathcal{E}_c$ in which $Q$ decides; note that $\mathcal{E}_c^Q$ exists as $\mathcal{A}$ satisfies \emph{Termination}.
The following holds for process $Q$: (1) $Q$ decides $v_c$ in $\mathcal{E}_c^Q$ (as $\mathcal{A}$ satisfies \emph{Agreement}), and (2) process $Q$ is silent in $\mathcal{E}_{\mathit{base}}$.
Let $t_Q$ denote the time at which $Q$ decides in $\mathcal{E}_c^Q$.
Similarly, there exists a process $P \in \processes{\mathit{base}} \setminus{\processes{c}}$; observe that (1) process $P$ decides $v_{\mathit{base}}$ in $\mathcal{E}_{\mathit{base}}$, and (2) process $P$ is silent in $\mathcal{E}_c^Q$.
Let $t_P$ denote the time at which $P$ decides in $\mathcal{E}_{\mathit{base}}$.

We now construct an execution $\mathcal{E} \in \mathit{execs}(\mathcal{A})$ by ``merging'' $\mathcal{E}_{\mathit{base}}$ and $\mathcal{E}_c^Q$:
\begin{compactenum}
    \item Processes in $\processes{c} \cap \processes{\mathit{base}}$ behave towards processes in $\processes{\mathit{base}} \setminus{\processes{c}}$ as in $\mathcal{E}_{\mathit{base}}$, and towards processes in $\processes{c} \setminus{\processes{\mathit{base}}}$ as in $\mathcal{E}_c^Q$.

    \item Communication between (1) processes in $\processes{\mathit{base}} \setminus{\processes{c}}$ and (2) processes in $\processes{c} \setminus{\processes{\mathit{base}}}$ is delayed until after $\max(t_P, t_Q)$.
    % $P$ has decided $v_{\mathit{base}}$ and $Q$ has decided $v_c$. 
    
    \item We set GST to after $\max(t_P, t_Q)$.
\end{compactenum}
The following holds for $\mathcal{E}$:
\begin{compactitem}
    \item Processes in $\processes{\mathit{base}} \ominus \processes{c}$ (symmetric difference) are correct in $\mathcal{E}$.

    \item Only processes in $\processes{\mathit{base}} \cap \processes{c}$ are faulty in $\mathcal{E}$.
    Recall that $|\processes{\mathit{base}} \cap \processes{c}| \leq t$ as $\mathit{base} \diamond c$.

    \item Process $Q$, which is correct in $\mathcal{E}$, cannot distinguish $\mathcal{E}$ from $\mathcal{E}_c^Q$ until time $\max(t_P, t_Q)$.
    % in which it decides $v_c$.
    Hence, process $Q$ decides $v_c$ in $\mathcal{E}$.

    \item Process $P$, which is correct in $\mathcal{E}$, cannot distinguish $\mathcal{E}$ from $\mathcal{E}_{\mathit{base}}$ until time $\max(t_P, t_Q)$.
    % in which it decides $v_{\mathit{base}}$.
    Hence, process $P$ decides $v_{\mathit{base}} \neq v_c$ in $\mathcal{E}$.
\end{compactitem}
Therefore, we reach a contradiction with the fact that $\mathcal{A}$ satisfies \emph{Agreement}.
Thus, $v_c = v_{\mathit{base}}$.
\end{proof}

Next, we formally prove that, for every input configuration $c_n \in \mathcal{I}_n$, there exists an execution $\mathcal{E}_n$ such that (1) $\mathcal{E}_n$ corresponds to $c_n$, and (2) $v_{\mathit{base}}$ is decided in $\mathcal{E}_n$.

\begin{lemma_triviality_complete} [restated]
For every input configuration $c_n \in \mathcal{I}_n$, there exists an execution $\mathcal{E}_{n} \in \mathit{execs}(\mathcal{A})$ such that (1) $\mathsf{input\_conf}(\mathcal{E}_{n}) = c_n$, and (2) $v_{\mathit{base}}$ is decided in $\mathcal{E}_{n}$.
\end{lemma_triviality_complete}
\begin{proof}
Fix any input configuration $c_n \in \mathcal{I}_n$.
We construct an input configuration $c_{n - t} \in \mathcal{I}_{n - t}$:
\begin{compactenum}
    \item For every process $P_i \notin \processes{\mathit{base}}$, we include a process-proposal pair $(P_i, v)$ in $c_{n - t}$ such that $v = \mathsf{proposal}(c_n[i])$.
    Note that there are $t$ such processes as $|\processes{\mathit{base}}| = n - t$.

    \item We include $n - 2t$ process-proposal pairs $(P_i, v)$ in $c_{n - t}$ such that (1) $P_i \in \processes{\mathit{base}}$, and (2) $v = \mathsf{proposal}(c_n[i])$.
    That is, we ``complete'' $c_{n - t}$ (constructed in the step 1) with $n - 2t$ process-proposal pairs such that the process is ``borrowed'' from $\mathit{base}$, and its proposal is ``borrowed'' from $c_n$.
\end{compactenum}
Observe that $c_{n - t} \diamond \mathit{base}$ as (1) $|\processes{c_{n - t}} \cap \processes{\mathit{base}}| \leq t$ (because $n - 2t \leq t$ when $n \leq 3t$), (2) there exists a process $P \in \processes{\mathit{base}} \setminus \processes{c_{n - t}}$ (because, when constructing $c_{n - t}$, we excluded $t > 0$ processes from $\mathit{base}$), and (3) there exists a process $Q \in \processes{c_{n - t}} \setminus{\processes{\mathit{base}}}$ (because we included $t > 0$ processes in $\mathit{c_{n - t}}$ which are not in $\mathit{base}$; step 1).

Let $\mathcal{E}_{n - t} \in \mathit{execs}(\mathcal{A})$ denote any infinite canonical execution such that $\mathsf{input\_conf}(\mathcal{E}_{n - t}) = c_{n - t}$.
As $\mathcal{A}$ satisfies \emph{Termination}, some value is decided by correct processes in $\mathcal{E}_{n - t}$; due to \Cref{lemma:triviality_compatible}, that value is $v_{\mathit{base}}$.
Finally, we are able to construct an infinite execution $\mathcal{E}_n \in \mathit{execs}(\mathcal{A})$ such that (1) $\mathsf{input\_conf}(\mathcal{E}_n) = c_n$, and (2) $v_{\mathit{base}}$ is decided in $\mathcal{E}_n$:
\begin{compactenum}
    \item All processes are correct in $\mathcal{E}_n$.

    \item Until some correct process $P \in \processes{c_{n - t}}$ decides $v_{\mathit{base}}$, $\mathcal{E}_n$ is identical to $\mathcal{E}_{n - t}$.
    \add{Let $\mathcal{S}$ denote the set of all processes which take a computational step in $\mathcal{E}_{n - t}$ until $P$ decides $v_{\mathit{base}}$; note that $\mathcal{S} \subseteq \processes{c_{n - t}}$ and $P \in \mathcal{S}$.}

    \item Afterwards, every process \add{$Q \notin \mathcal{S}$} ``wakes up'' with the proposal specified in $c_n$.
    
    \item GST is set to after all processes have taken a computational step.
\end{compactenum}
Therefore, $v_{\mathit{base}}$ is indeed decided in $\mathcal{E}_n$ and $\mathsf{input\_conf}(\mathcal{E}_n) = c_n$, which concludes the proof.
\end{proof}
