# Supplementary material for: Partial Synchrony for Free? New Upper Bounds for Byzantine Agreement
Source: arXiv:2402.10059 source file (2024-10-23)
Supplement: Supplementary file 14 [file vector_with_quadratic_communication.tex]

\section{Quadratic Communication}

%%%%%%%%%
% View core's utilities (begin)
%%%%%%%%%
\begin{algorithm} [h]
\caption{View core's utilities (for process $P_i$)}
\label{algorithm:utilities}
\begin{algorithmic} [1]
\State \textbf{function} $\mathsf{msg(String} \text{ } \mathit{type}, \mathsf{Value} \text{ } \mathit{value}, \mathsf{Quorum\_Certificate} \text{ } \mathit{qc}, \mathsf{View} \text{ }\mathit{view}\mathsf{)}$:
\State \hskip2em $m.\mathit{type} \gets \mathit{type}$; $m.\mathit{value} \gets \mathit{value}$; $m.\mathit{qc} \gets \mathit{qc}$; $m.\mathit{view} \gets \mathit{view}$
\State \hskip2em \textbf{return} $m$

\smallskip
\State \textbf{function} $\mathsf{vote\_msg(String} \text{ } \mathit{type}, \mathsf{Value} \text{ } \mathit{value}, \mathsf{Quorum\_Certificate} \text{ } \mathit{qc}, \mathsf{View} \text{ }\mathit{view}\mathsf{)}$:
\State \hskip2em $m \gets \mathsf{msg(}\mathit{type}, \mathit{value}, \mathit{qc}, \mathit{view}\mathsf{)}$
\State \hskip2em $m.\mathit{partial\_sig} \gets \mathit{ShareSign}_i([m.\mathit{type}, m.\mathit{value}, m.\mathit{view}])$
\State \hskip2em \textbf{return} $m$

\smallskip
\State \textcolor{blue}{\(\triangleright\) All the messages in $M$ have the same type, value and view}
\State \textbf{function} $\mathsf{qc(Set(Vote\_Message)} \text{ } M\mathsf{)}$:
\State \hskip2em $\mathit{qc}.\mathit{type} \gets m.\mathit{type}$, where $m \in M$
\State \hskip2em $\mathit{qc}.\mathit{value} \gets m.\mathit{value}$, where $m \in M$
\State \hskip2em $\mathit{qc}.\mathit{view} \gets m.\mathit{view}$, where $m \in M$
\State \hskip2em $\mathit{qc}.\mathit{sig} \gets \mathit{Combine}\big(\{\mathit{partial\_sig} \,|\, \mathit{partial\_sig} \text{ is in a message that belongs to } M\}\big)$
\State \hskip2em \textbf{return} $\mathit{qc}$

\smallskip
\State \textbf{function} $\mathsf{matching\_msg(Message} \text{ }m, \mathsf{String} \text{ }\mathit{type}, \mathsf{View} \text{ } \mathit{view}\mathsf{)}$:
\State \hskip2em \textbf{return} $m.\mathit{type} = \mathit{type}$ and $m.\mathit{view} = \mathit{view}$

\smallskip
\State \textbf{function} $\mathsf{matching\_qc(Quorum\_Certificate} \text{ } \mathit{qc}, \mathsf{String} \text{ } \mathit{type}, \mathsf{View} \text{ } \mathit{view}\mathsf{)}$:
\State \hskip2em \textbf{return} $\mathit{qc}.\mathit{type} = \mathit{type}$ and $\mathit{qc}.\mathit{view} = \mathit{view}$

\smallskip
\State \textbf{function} $\mathsf{encode(String} \text{ } \mathit{file} \mathsf{)}$:
\State \hskip2em \textbf{return} $[c_1, ..., ... c_n]$

\smallskip
\State \textbf{function} $\mathsf{decode(Array(Chunk) } \text{ } \mathit{chunks}, \mathsf{String} \text{ } \mathit{h} \mathsf{)}$:
\State \hskip2em $file \gets \mathsf{reverse(} \mathit{chunks} \mathsf{)}$
\State \hskip2em \textbf{if} $\mathsf{Hash(} \mathit{file}\mathsf{)} = \mathit{h}$
\State \hskip4em \textbf{return} $file$
\end{algorithmic}
\end{algorithm} 
%%%%%%%%
% View core utilities (end)
%%%%%%%%

%%%%%%%%
% View core (begin)
%%%%%%%%
\begin{algorithm} 
\caption{View core (for process $P_i$)}
\label{algorithm:view_1}
\begin{algorithmic} [1]
\State \textbf{upon} $\mathsf{init(Value } \text{ } \mathit{proposal})$:
\State \hskip2em $\mathit{proposal}_i \gets \mathit{proposal}$ \BlueComment{$P_i$'s proposal}

\smallskip
\State \textbf{upon} $\mathsf{start\_executing(View} \text{ } \mathit{view}\mathsf{)}$:

% \smallskip 
\State \hskip2em \textcolor{blue}{\(\triangleright\) Discover phase}
\State \hskip2em \textbf{send} $\mathsf{msg(}\textsc{view-change}, \bot, \mathit{prepareQC}, \mathit{view}\mathsf{)}$ to $\mathsf{leader}(\mathit{view})$

\smallskip
\State \hskip2em \textbf{as} $\mathsf{leader}(\mathit{view})$:
\State \hskip4em \textbf{wait for} $2f + 1$ \textsc{view-change} messages:
\State \hskip6em $M \gets \{m \,|\, \mathsf{matching\_msg(}m, \textsc{view-change}, \mathit{view}\mathsf{)}\}$
\State \hskip4em $\mathsf{Quorum\_Certificate} \text{ } \mathit{highQC} \gets \mathit{qc}$ with the highest $\mathit{qc}.\mathit{view}$ in $M$ \label{line:highest_qc}
\State \hskip4em $\mathsf{HashValue} \text{ } \mathit{hashProposal} \gets \mathit{highQC}.\mathit{value}$
\State \hskip4em \textbf{if} $\mathit{hashProposal} = \bot$: \BlueComment{No one prepared anything among the senders of $M$}
\State \hskip6em $\mathsf{VectorValue} \text{ }  \mathit{proposal} \gets \mathsf{Vector(}M\mathsf{)}$
\BlueComment{building a vector of $2f+1$ proposals}
\State \hskip6em $\text{GO TO Prepare phase at line } \ref{line:bcast_prepare}$
\State \hskip4em \textbf{else}:
\State \hskip6em \textbf{broadcast} $\mathsf{msg(}\textsc{discover}, \mathit{hashProposal}, \mathit{highQC}, \mathit{view}\mathsf{)}$

\smallskip
\State \hskip2em \textbf{as} a process: \BlueComment{every process executes this part of the pseudocode}
\State \hskip4em \textbf{wait for} message $m$: $\mathsf{matching\_msg(}m, \textsc{discover}, \mathit{view}\mathsf{)}$ from $\mathsf{leader}(\mathit{view})$
\State \hskip4em \textbf{send} $\mathsf{msg(}\textsc{discover}, \mathsf{chunkStore}_i[m.\mathit{qc}.\mathit{value}]\mathsf{)}$ to $\mathsf{leader}(\mathit{view})$ \label{line:proposal_support}

% \smallskip 
\State \hskip2em \textcolor{blue}{\(\triangleright\) Prepare phase}
%\State \hskip2em \textbf{send} $\mathsf{msg(}\textsc{view-change}, \bot, \mathit{prepareQC}, \mathit{view}\mathsf{)}$ to $\mathsf{leader}(\mathit{view})$

\smallskip
\State \hskip2em \textbf{as} $\mathsf{leader}(\mathit{view})$:
\State \hskip4em \textbf{wait for} a set $M$ of $f + 1$ consistent \textsc{discover} messages:
\State \hskip6em $\mathsf{VectorValue} \text{ }  \mathit{proposal} \gets \mathsf{decode(}\{m.\mathit{chunk} \,|\, m \in M\})$
\BlueComment{We have $\mathsf{Hash(}\mathit{proposal}\mathsf{)} = \mathit{hashProposal}$}
%\State \hskip4em $\mathsf{Quorum\_Certificate} \text{ } \mathit{highQC} \gets \mathit{qc}$ with the highest $\mathit{qc}.\mathit{view}$ in $M$ \label{line:highest_qc}
%\State \hskip4em $\mathsf{Value} \text{ } \mathit{proposal} \gets \mathit{highQC}.\mathit{value}$
%\State \hskip4em \textbf{if} $\mathit{proposal} = \bot$:
%\State \hskip6em $\mathit{proposal} \gets \mathit{proposal}_i$ \BlueComment{$\mathit{proposal}_i$ denotes the proposal of $P_i$}
\State \hskip4em \textbf{broadcast} $\mathsf{msg(}\textsc{prepare}, \mathit{proposal}, \mathit{highQC}, \mathit{view}\mathsf{)}$ \label{line:bcast_prepare}

\smallskip
\State \hskip2em \textbf{as} a process: \BlueComment{every process executes this part of the pseudocode}
\State \hskip4em \textbf{wait for} message $m$: $\mathsf{matching\_msg(}m, \textsc{prepare}, \mathit{view}\mathsf{)}$ from $\mathsf{leader}(\mathit{view})$
\State \hskip4em \textbf{if} $m.\mathit{qc}.\mathit{hashValue} = \mathsf{Hash(}m.\mathit{value}\mathsf{)}$ and ($\mathit{lockedQC}.\mathit{value} = m.\mathit{value}$ or $\mathit{qc}.\mathit{view} > \mathit{lockedQC}.\mathit{view}$): \label{line:view_core_check}
\State \hskip6em \textbf{send} $\mathsf{vote\_msg(}\textsc{prepare}, m.\mathit{value},\bot, \mathit{view}\mathsf{)}$ to $\mathsf{leader}(\mathit{view})$ \label{line:proposal_support}

\smallskip
\State \hskip2em \textcolor{blue}{\(\triangleright\) Precommit phase}
\State \hskip2em \textbf{as} $\mathsf{leader}(\mathit{view})$:
\State \hskip4em \textbf{wait for} $2f + 1$ votes: $V \gets \{\mathit{vote} \,|\, \mathsf{matching\_msg(}\mathit{vote}, \textsc{prepare}, \mathit{view}\mathsf{)}\}$
\State \hskip4em $\mathsf{Quorum\_Certificate} \text{ } \mathit{qc} \gets \mathsf{qc(}V\mathsf{)}$
\State \hskip4em \textbf{broadcast} $\mathsf{msg(}\textsc{precommit}, \bot, \mathit{qc}, \mathit{view}\mathsf{)}$

\smallskip
\State \hskip2em \textbf{as} a process: \BlueComment{every process executes this part of the pseudocode}
\State \hskip4em \textbf{wait for} message $m$: $\mathsf{matching\_qc(}m.\mathit{qc}, \textsc{prepare}, \mathit{view}\mathsf{)}$ from $\mathsf{leader}(\mathit{view})$
\State \hskip4em $\mathit{prepareQC} \gets m.\mathit{qc}$ \label{line:quad_update_prepare_qc}
\State \hskip4em \textbf{send} $\mathsf{vote\_msg(}\textsc{precommit}, m.\mathit{qc}.\mathit{value}, \bot, \mathit{view}\mathsf{)}$ to $\mathsf{leader}(\mathit{view})$

\smallskip
\State \hskip2em \textcolor{blue}{\(\triangleright\) Commit phase}
\State \hskip2em \textbf{as} $\mathsf{leader}(\mathit{view})$:
\State \hskip4em \textbf{wait for} $2f + 1$ votes: $V \gets \{\mathit{vote} \,|\, \mathsf{matching\_msg(}\mathit{vote}, \textsc{precommit}, \mathit{view}\mathsf{)}\}$
\State \hskip4em $\mathsf{Quorum\_Certificate}$ $\mathit{qc} \gets \mathsf{qc(}V\mathsf{)}$
\State \hskip4em \textbf{broadcast} $\mathsf{msg(}\textsc{commit}, \bot, \mathit{qc}, \mathit{view}\mathsf{)}$

\smallskip
\State \hskip2em \textbf{as} a process: \BlueComment{every process executes this part of the pseudocode}
\State \hskip4em \textbf{wait for} message $m$: $\mathsf{matching\_qc(}m.\mathit{qc}, \textsc{precommit}, \mathit{view}\mathsf{)}$ from $\mathsf{leader}(\mathit{view})$
\State \hskip4em $\mathit{lockedQC} \gets m.\mathit{qc}$ \label{line:update_locked_qc}
\State \hskip4em \textbf{send} $\mathsf{vote\_msg(}\textsc{commit}, m.\mathit{qc}.\mathit{value}, \bot, \mathit{view}\mathsf{)}$ to $\mathsf{leader}(\mathit{view})$

%%%%%%%%%%%
%%store before restore
%%%%%%%%%%%
\algstore{myalg}
\end{algorithmic}
\end{algorithm}

\begin{algorithm} 
%\caption{\name: View core (for process $P_i$)} \label{algorithm:view_1}
\begin{algorithmic} [1]
%%%%%%%%%%%
%restore after store
%%%%%%%%%%%
\algrestore{myalg}

\smallskip
\State \hskip2em \textcolor{blue}{\(\triangleright\) Decide phase}
\State \hskip2em \textbf{as} $\mathsf{leader}(\mathit{view})$:
\State \hskip4em \textbf{wait for} $2f + 1$ votes: $V \gets \{\mathit{vote} \,|\, \mathsf{matching\_msg(}\mathit{vote}, \textsc{commit}, \mathit{view}\mathsf{)}\}$
\State \hskip4em $\mathsf{Quorum\_Certificate}$ $\mathit{qc} \gets \mathsf{qc(}V\mathsf{)}$
\State \hskip4em \textbf{broadcast} $\mathsf{msg(}\textsc{decide}, \bot, \mathit{qc}, \mathit{view}\mathsf{)}$ \label{line:broadcast_decide_message}

\smallskip
\State \hskip2em \textbf{as} a process: \BlueComment{every process executes this part of the pseudocode}
\State \hskip4em \textbf{wait for} message $m$: $\mathsf{matching\_qc(}m.\mathit{qc}, \textsc{commit}, \mathit{view}\mathsf{)}$ from $\mathsf{leader}(\mathit{view})$
\State \hskip4em \textbf{trigger} $\mathsf{decide}(\mathit{vectorValue})$ \label{line:decide_view_core} \BlueComment{$\mathsf{Hash(} \mathit{vectorValue} \mathsf{)} = m.\mathit{qc}.\mathit{hashValue}$}
\State \hskip4em \textbf{send} $\mathsf{vote\_msg(}\textsc{decide}, m.\mathit{qc}.\mathit{value}, \bot, \mathit{view}\mathsf{)}$ to $\mathsf{leader}(\mathit{view})$
\State \hskip4em \textbf{broadcast} $\mathsf{msg(}\textsc{decision}, (m.\mathit{qc}, \mathsf{chunk}_i(\mathit{vectorValue})),\bot, \bot \mathsf{)}$

\smallskip
\State \hskip2em \textcolor{blue}{\(\triangleright\) Finalize phase}
\State \hskip2em \textbf{as} $\mathsf{leader}(\mathit{view})$:
\State \hskip4em \textbf{wait for} $2f + 1$ votes: $V \gets \{\mathit{vote} \,|\, \mathsf{matching\_msg(}\mathit{vote}, \textsc{decide}, \mathit{view}\mathsf{)}\}$
\State \hskip4em $\mathsf{Quorum\_Certificate}$ $\mathit{qc} \gets \mathsf{qc(}V\mathsf{)}$
\State \hskip4em \textbf{broadcast} $\mathsf{msg(}\textsc{finalize}, \bot, \mathit{qc}, \mathit{view}\mathsf{)}$ \label{line:broadcast_finalize_message}

\smallskip
\State \hskip2em \textbf{as} a process: \BlueComment{every process executes this part of the pseudocode}
\State \hskip4em \textbf{wait for} message $m$: $\mathsf{matching\_qc(}m.\mathit{qc}, \textsc{decide}, \mathit{view}\mathsf{)}$ from $\mathsf{leader}(\mathit{view})$
\State \hskip4em \textbf{broadcast} $m$ \label{line:echo_finalize_message} \BlueComment{allow other process to stop in case the leader is Byzantine}
\State \hskip4em \textbf{trigger} $\mathsf{stop}()$ \BlueComment{At least $t+1$ processes decided, so $P_i$ can stop to participate} \label{line:stop_view_core}

\smallskip \smallskip
\State \hskip2em \textcolor{blue}{\(\triangleright\) Always (Quadratic uniform decision and halting)}
\State \hskip2em \textbf{as} \text{ a } $\mathsf{process}$:
\State \hskip4em \textbf{upon} the reception of a consistent set $M$ of $f+1$ $\textsc{decision}$ messages \label{line:wait_for_uniformity}:
\State \hskip6em $\mathsf{VectorValue} \text{ }  \mathit{decision} \gets \mathsf{decode(}\{m.\mathit{chunk} \,|\, m \in M\})$
\BlueComment{"consistent" means: $\forall m \in M, m.\mathit{qc}.\mathit{hashValue} = \mathsf{Hash(} \mathit{decision}  \mathsf{)}$}
\State \hskip6em \textbf{trigger} $\mathsf{decide}(\mathit{decision})$ \label{line:decide_view_core} 

\smallskip \smallskip
\State \hskip4em \textbf{upon} the reception of message $m$ s.t.  $\mathsf{matching\_qc}(m.\mathit{qc}, \textsc{decide}, v)$ for some view $v$:
%$m.\mathit{type} = \textsc{finalize}$,
\State \hskip6em \textbf{trigger} $\mathsf{stop}()$ \BlueComment{At least $t+1$ processes decided, so $P_i$ can stop to participate. Of course, if $P_i$ did not decide yet, line \ref{line:wait_for_uniformity} remains active} \label{line:stop_view_core}

\end{algorithmic}
\end{algorithm}
%%%%%%%%
% View core (end)
%%%%%%%%
