# Supplementary material for: Partial Synchrony for Free? New Upper Bounds for Byzantine Agreement
Source: arXiv:2402.10059 source file (2024-10-23)
Supplement: Supplementary file 15 [file view_synchronization_proof.tex]

\section{\sync: Formal Proof of Correctness \& Complexity}

This section proves the correctness and establishes the complexity of \sync (\Cref{algorithm:sync}).

\paragraph{Behaviors \& timer histories.}
Following the formalism introduced in~\cite{civit2022byzantine}, we define the behaviors and timer histories of processes.
A \emph{behavior} of a process $p_i$ is a sequence of (1) message-sending events performed by $p_i$, (2) message-reception events performed by $p_i$, and (3) internal events performed by $p_i$ (e.g., triggering the $\mathsf{advance}(\cdot)$ event or invocations of the $\mathsf{measure}(\cdot)$ and $\mathsf{cancel()}$ methods on the local timers).
A \emph{timer history} of a process $p_i$ is a sequence of (1) invocations of the $\mathsf{measure}(\cdot)$ and $\mathsf{cancel}()$ methods on $\mathit{view\_timer}_i$, $\mathit{help\_timer}_i$ and $\mathit{enter\_timer}_i$, and (2) processed expiration events of $\mathit{view\_timer}_i$, $\mathit{help\_timer}_i$ and $\mathit{enter\_timer}_i$.
Observe that a timer history of a process is a subsequence of the behavior of the process.

If an event $e$ belongs to a sequence of events $\mathcal{S}$, we write $e \in \mathcal{S}$; otherwise, we write $e \notin \mathcal{S}$.
If an event $e_1$ precedes an event $e_2$ in a sequence $\mathcal{S}$, we write $e_1 \stackrel{\mathcal{S}}{\prec} e_2$.
% Note that, if $e_1 \stackrel{\beta_i}{\prec} e_2$ and $e_1$ occurs at some time $t_1$ and $e_2$ occurs at some time $t_2$, $t_1 \leq t_2$.

We denote by $h_i|_{\mathit{view}}$ (resp., $h_i|_{\mathit{enter}}$) a subsequence of $h_i$ associated with $\mathit{view\_timer}_i$ (resp., $\mathit{enter\_timer}_i$), where $h_i$ is a timer history of a process $p_i$.
If an expiration event $\mathit{Exp}$ of a timer is associated with an invocation $\mathit{Inv}$ of the $\mathsf{measure(\cdot)}$ method on the timer, we say that $\mathit{Inv}$ \emph{produces} $\mathit{Exp}$.
Note that a single invocation of the $\mathsf{measure}(\cdot)$ method produces at most one expiration event.
Moreover, any expiration event is produced by exactly one invocation of the $\mathsf{measure}(\cdot)$ method.

Given an execution, we denote by $\beta_i$ and $h_i$ the behavior and the timer history of the process $p_i$, respectively.

\paragraph{Proof of correctness.}
To prove the correctness of \sync, we need to prove that \sync satisfies the eventual synchronization property.
First, we prove that, between any expiration event of the $\mathit{enter\_timer}_i$ of a correct process $p_i$ and the corresponding invocation of the $\mathsf{measure}(\cdot)$ method, only internal events associated with $\mathit{help\_timer}_i$ can exist in $h_i$.

\begin{lemma} \label{lemma:enter_invocation_expiration}
Let $p_i$ be any correct process
Let $\mathit{Exp}_e$ be any expiration event of the $\mathit{enter\_view}_i$ timer that belongs to $h_i$, and let $\mathit{Inv}_e$ be the invocation of the $\mathsf{measure}(\cdot)$ method (on $\mathit{enter\_view}_i$) that produces $\mathit{Exp}_e$.
Then, $\mathit{Exp}_e$ immediately follows $\mathit{Inv}_e$ in $h_i|_{enter}$.
\end{lemma}
\begin{proof}
By contradiction, suppose that $\mathit{Exp}_e$ does not immediately follow $\mathit{Inv}_e$ in $h_i|_{\mathit{enter}}$.
We consider three possibilities:
\begin{compactitem}
    \item Let an invocation $\mathit{Inv}_e'$ of the $\mathsf{measure}(\cdot)$ method immediately follow $\mathit{Inv}_e$ in $h_i|_{\mathit{enter}}$:
    Invocation $\mathit{Inv}_e'$ is invoked at line~\ref{line:measure_enter}.
    However, it is immediately preceded by an invocation of the $\mathsf{cancel}()$ method (line~\ref{line:cancel_enter}).
    Therefore, this case is impossible.

    \item Let an invocation $\mathit{Inv}_e'$ of the $\mathsf{cancel}()$ method immediately follow $\mathit{Inv}_e$ in $h_i|_{\mathit{enter}}$:
    This case is impossible as $\mathit{Inv}_e$ does produce $\mathit{Exp}_e$.

    \item Let an expiration event $\mathit{Exp}_d' \neq \mathit{Exp}_d$ immediately follow $\mathit{Inv}_e$ in $h_i|_{\mathit{enter}}$:
    As $\mathit{Inv}_e$ is invoked at line~\ref{line:measure_enter}, it is immediately preceded by an invocation of the $\mathsf{cancel}()$ method (line~\ref{line:cancel_enter}).
    Hence, $\mathit{Exp}_d'$ cannot be produced, which renders this case impossible as well.
\end{compactitem}
As neither of three other possibilities can happen, $\mathit{Exp}_d$ indeed immediately follows $\mathit{Inv}_e$ in $h_i|_{\mathit{enter}}$.
\end{proof}

\begin{lemma} \label{lemma:enter_between}
Let $p_i$ be any correct process.
Let $\mathit{Exp}_e$ be any expiration event of $\mathit{enter\_view}_i$ that belongs to $h_i$, and let $\mathit{Inv}_e$ be the invocation of the $\mathsf{measure}(\cdot)$ method (on $\mathit{enter\_view}_i$) that produces $\mathit{Exp}_e$.
If there exists an internal event $e \in h_i$ such that $\mathit{Inv}_e \stackrel{h_i}{\prec} e \stackrel{h_i}{\prec} \mathit{Exp}_e$, then $e$ is associated with $\mathit{help\_timer}_i$.
\end{lemma}
\begin{proof}
To prove the lemma, we consider all possibilities:
\begin{compactitem}
    \item Let $e$ be associated with $\mathit{enter\_timer}_i$.
    In this case, we further distinguish three scenarios:
    \begin{compactitem}
        \item Let $e$ be an invocation of the $\mathsf{measure}(\cdot)$ method:
        Hence, $e$ is invoked at line~\ref{line:measure_enter}.
        Therefore, $e$ is immediately preceded in $h_i$ by an invocation of the $\mathsf{cancel}()$ method on $\mathit{enter\_timer}_i$ (line~\ref{line:cancel_enter}).
        However, this is impossible as $\mathit{Inv}_e$ produces $\mathit{Exp}_e$.

        \item Let $e$ be an invocation of the $\mathsf{cancel}()$ method:
        This case is impossible as $\mathit{Inv}_e$ produces $\mathit{Exp}_e$.

        \item Let $e$ be an expiration event:
        Let $\mathit{Inv}_e'$ be the invocation of the $\mathsf{measure}(\cdot)$ method that produces $e$.
        Crucially, $\mathit{Inv}_e \stackrel{h_i}{\prec} \mathit{Inv}_e'$; otherwise, as $\mathit{Inv}_e$ is immediately preceded in $h_i$ by an invocation of the $\mathsf{cancel}()$ method on $\mathit{enter\_timer}_i$ (line~\ref{line:cancel_enter}), $\mathit{Inv}_e'$ would not produce $e$.
        Since an invocation of the $\mathsf{cancel}()$ method on $\mathit{enter\_timer}_i$ (line~\ref{line:cancel_enter}) immediately precedes $\mathit{Inv}_e'$ in $h_i$, $\mathit{Inv}_e$ could not have produced $\mathit{Exp}_e$, thus rendering this case impossible as well.
    \end{compactitem}

    \item Let $e$ be associated with $\mathit{view\_timer}_i$.
    We further separate three cases:
    \begin{compactitem}
        \item Let $e$ be an invocation of the $\mathsf{measure}(\cdot)$ method:
        As $\mathit{Inv}_e \stackrel{h_i}{\prec} e$, $e$ is invoked at line~\ref{line:measure_view}.
        However, as $e$ is preceded by an expiration event of the $\mathit{enter\_timer}_i$ (line~\ref{line:enter_expires}), \Cref{lemma:enter_invocation_expiration} shows that $\mathit{Exp}_e \stackrel{h_i}{\prec}$, this is impossible.

        \item Let $e$ be an invocation of the $\mathsf{cancel}()$ method:
        As $e$ is immediately followed by an invocation of the $\mathsf{cancel}()$ method on the $\mathit{enter\_view}_i$ timer (line~\ref{line:cancel_enter}), this case contradicts \Cref{lemma:enter_invocation_expiration}.
        Therefore, this case is impossible.

        \item Let $e$ be an expiration event:
        Let $\mathit{Inv}_v$ be the invocation of the $\mathsf{measure}(\cdot)$ method that produces $e$.
        Importantly, $\mathit{Inv}_e \stackrel{h_i}{\prec} \mathit{Inv}_v$; otherwise, $\mathit{Inv}_v$ would be cancelled at line~\ref{line:cancel_view}.
        Therefore, $\mathit{Inv}_v$ is invoked at line~\ref{line:measure_view}.
        Due to \Cref{lemma:enter_invocation_expiration}, $\mathit{Exp}_e \stackrel{h_i}{\prec} \mathit{Inv}_v \stackrel{h_i}{\prec} e$, which is impossible.
    \end{compactitem}
\end{compactitem}
The lemma holds as all other possibilities are shown to be impossible.
\end{proof}

Next, we prove that views entered by a correct process are monotonically increasing.

\begin{lemma} [Monotonically increasing views] \label{lemma:monotonically_increasing_views}
Let $p_i$ be a correct process.
Let $e_1 = \mathsf{advance}(v_1)$, $e_2 = \mathsf{advance}(v_2)$ and $e_1 \stackrel{\beta_i}{\prec} e_2$.
Then, $v_1 < v_2$.
\end{lemma}
\begin{proof}
Throughout the execution, the value of the $\mathit{view}_i$ variable only increases (ensured by the check at line~\ref{line:receive_quorum} and the assignment at line~\ref{line:update_view_2}).
Hence, $v_1 \leq v_2$.

By contradiction, let $v_1 = v_2$.
Importantly, $\mathsf{advance}(v_2)$ is triggered at line~\ref{line:enter_v}; it is impossible for $\mathsf{advance}(v_2)$ to be triggered at line~\ref{line:enter_1} as the $\mathsf{init}$ block is executed at most once.
Hence, there exists an event $e_2' \in \beta_i$ that is an expiration event of the $\mathit{enter\_view}_i$ timer (line~\ref{line:enter_expires}).
Moreover, $e_1 \stackrel{\beta_i}{\prec} e_2'$ and $e_2' \stackrel{\beta_i}{\prec} e_2$.
Let $e_1'$ denote the invocation of the $\mathsf{measure}(\cdot)$ method on $\mathit{enter\_view}_i$ that produces $e_2'$; note that $e_1' \stackrel{\beta_i}{\prec} e_2'$.
We now consider two possibilities:
\begin{compactitem}
    \item Let $e_1$ be triggered at line~\ref{line:enter_1}.
    In this case, $e_1 \stackrel{\beta_i}{\prec} e_1'$.
    Hence, when $e_1'$ is triggered (line~\ref{line:measure_enter}), $\mathit{view}_i$ takes a value greater than $v_1$ (by the check at line~\ref{line:receive_quorum} and the assignment at line~\ref{line:update_view_2}).
    As the value of the $\mathit{view}_i$ variable only increases, $v_1 < v_2$ in this case.

    \item Let $e_1$ be triggered at line~\ref{line:enter_v}.
    Let $\mathit{Exp}_e$ denote the expiration event of the $\mathit{enter\_timer}_i$ which leads to $e_1$ (line~\ref{line:enter_expires}).
    By \Cref{lemma:enter_invocation_expiration}, $\mathit{Exp}_e \stackrel{\beta_i}{\prec} e_1'$.
    Hence, $e_1 \stackrel{\beta_i}{\prec} e_1'$ in this case as well.
    Therefore, when $e_1'$ is triggered (line~\ref{line:measure_enter}), $\mathit{view}_i$ takes a value greater than $v_1$ (by the check at line~\ref{line:receive_quorum} and the assignment at line~\ref{line:update_view_2}).
    As the value of the $\mathit{view}_i$ variable only increases, $v_1 < v_2$.
\end{compactitem}
As $v_1 < v_2$ holds for any possible scenario, the proof is concluded.
\end{proof}

\begin{lemma} \label{lemma:view_invocation_invocation}
Let $p_i$ be any correct process.
Let $\mathit{Inv}_v$ be any invocation of the $\mathsf{measure}(\cdot)$ method on $\mathit{view\_timer}_i$ that belongs to $h_i$.
Invocation $\mathit{Inv}_v$ is not immediately followed by another invocation of the $\mathsf{measure}(\cdot)$ method in $h_i|_{\mathit{view}}$.
\end{lemma}
\begin{proof}
By contradiction, suppose that $\mathit{Inv}_v$ is immediately followed by another invocation $\mathit{Inv}_v'$ of the $\mathsf{measure}(\cdot)$ method in $h_i|_{\mathit{view}}$.
Invocation $\mathit{Inv}_v'$ is invoked at line~\ref{line:measure_enter}.
Hence, $\mathit{Inv}_v'$ is immediately preceded by an expiration event $\mathit{Exp}_e$ in $h_i$ (line~\ref{line:enter_expires}).
Let $\mathit{Inv}_e$ denote the invocation of the $\mathsf{measure}(\cdot)$ method that produces $\mathit{Exp}_e$.
By \Cref{lemma:enter_between}, $\mathit{Inv}_v \stackrel{h_i}{\prec} \mathit{Inv}_e$.
As $\mathit{Inv}_e$ is invoked at line~\ref{line:measure_enter}, there exists an invocation of the $\mathsf{cancel}()$ method on $\mathit{view\_timer}_i$ (line~\ref{line:cancel_view}) between $\mathit{Inv}_v$ and $\mathit{Inv}_v'$, which contradicts the fact that $\mathit{Inv}_v'$ immediately follows $\mathit{Inv}_v$ in $h_i|_{\mathit{view}}$.
\end{proof}

\begin{lemma}
Let $p_i$ be any correct process.
Let $\mathit{Exp}_v$ be any expiration event of $\mathit{view\_timer}_i$ that belongs to $h_i$, and let $\mathit{Inv}_v$ be the invocation of the $\mathsf{measure}(\cdot)$ method (on $\mathit{view\_timer}_i$) that produces $\mathit{Exp}_v$.
Then, $\mathit{Exp}_v$ immediately follows $\mathit{Inv}_v$ in $h_i|_{\mathit{view}}$.
\end{lemma}
\begin{proof}
By \Cref{lemma:view_invocation_invocation}, an invocation of the $\mathsf{measure}(\cdot)$ method cannot immediately follow $\mathit{Inv}_v$ in $h_i|_{\mathit{view}}$.
Moreover, an invocation of the $\mathsf{cancel}()$ method cannot immediately follow $\mathit{Inv}_v$ as $\mathit{Inv}_v$ produces $\mathit{Exp}_v$.
Finally, another expiration event of $\mathit{view\_timer}_i$ cannot immediately follow $\mathit{Inv}_v$ due to an induction argument.
\end{proof}
