# Supplementary material for: Partial Synchrony for Free? New Upper Bounds for Byzantine Agreement
Source: arXiv:2402.10059 source file (2024-10-23)
Supplement: Supplementary file 16 [file echo_validation_broadcast_new.tex]

\section{Validation Broadcast: Concrete Implementations to be Employed in \name} \label{section:validation_broadcast}

In this section, we present concrete implementations of the validation broadcast primitive that we employ in \name to obtain Byzantine agreement algorithms with different bit complexities introduced in \Cref{subsection:concrete_algorithms}. 
We start by recalling the definition of validation broadcast (\Cref{app:validation-broadcast-definition}).
We then present three implementations of the primitive with different trade-offs between resilience, bit complexity and adversary power. These trade-offs are summarized in \Cref{tab:validation-broadcast-summary}.
% that tolerates up to $t$ Byzantine failures among $n = 3t+1$ processes and achieves $O(n^2L)$ bit complexity.

\begin{table}[ht]
\centering
\begin{tabular}{ |p{2.4cm}|p{2.7cm}|p{1.3cm}|p{2cm}|p{2cm}|  }
 \hline
 \centering Algorithm & \centering Exchanged bits & \centering Resilience & 
\centering Cryptography \tabularnewline
 \hline
 \hline

\centering \textbf{\textsc{\Cref{algorithm:echo_basic}}} (\Cref{subsection:validation_broadcast_basic_implementation})     & \centering $O(n^2L)$ & \centering $3t+1$ & \centering None \tabularnewline

 \hline

  \centering \textbf{\textsc{\Cref{algorithm:validation_broadcast_long_3_4}}} (\Cref{subsection:validation_bcast_long_3_4})     & \centering $O(nL + n^2\kappa)$ & \centering $3t+1$ & \centering Hash \tabularnewline

 % \hline

 % \centering \textbf{\textsc{\Cref{algorithm:validation_broadcast_long_3_4}}} (\Cref{subsection:validation_bcast_long_3_4})     & \centering $O(nL + n^2\kappa)$ & \centering $4t+1$ & \centering Hash \tabularnewline

 \hline

 \centering \textbf{\textsc{\Cref{algorithm:its_validation_broadcast}}} (\Cref{subsection:its_validation_broadcast})                 & \centering $O(nL + n^2\log n)$ & \centering $5t+1$ & \centering None \tabularnewline
 \hline
\end{tabular}
    \caption{Relevant aspects of the  asynchronous validating broadcast algorithms we propose.
    \\($L$ denotes the bit-size of a value, whereas $\kappa$ denotes the bit-size of a hash value.)}
\label{tab:validation-broadcast-summary}
\end{table}

\subsection{Validation Broadcast: Definition and Properties}\label{app:validation-broadcast-definition}
Validation broadcast is a primitive in which processes broadcast their input value and eventually validate some value.
The validation broadcast primitive exposes the following interface:
\begin{compactitem}
    \item \textbf{request} $\mathsf{broadcast}(v \in \mathsf{Value})$: a process broadcasts value $v$.

    \item \textbf{request} $\mathsf{abandon}$: a process stops participating in validation broadcast.

    \item \textbf{indication} $\mathsf{validate}(v' \in \mathsf{Value})$: a process validates value $v'$.

    \item \textbf{indication} $\mathsf{completed}$: a process is notified that validation broadcast has completed.
\end{compactitem}
Every correct process broadcasts at most once and it does so with a valid value.
Not all correct processes are guaranteed to broadcast their value.
The validation broadcast primitive guarantees the following properties:
\begin{compactitem}
    \item \emph{Strong validity:} If all correct processes that broadcast do so with the same value $v$, then no correct process validates any value $v' \neq v$.

    \item \emph{External validity:} If any correct process validates a value $v'$, then $\mathsf{valid}(v') = \mathit{true}$.

    \item \emph{Integrity:} No correct process receives a $\mathsf{completed}$ indication unless it has previously broadcast a value.

    \item \emph{Termination:} If all correct processes broadcast their value and no correct process abandons validation broadcast, then every correct process eventually receives a $\mathsf{completed}$ indication.

    \item \emph{Totality:} If any correct process receives a $\mathsf{completed}$ indication at time $\tau$, then every correct process validates a value by time $\max(\text{GST},\tau) + 2\delta$.
\end{compactitem}
We underline that a correct process might validate a value even if (1) it has not previously broadcast its input value, or (2) it has previously abandoned the primitive, or (3) it has previously received a $\mathsf{completed}$ indication. Moreover, a correct process may validate multiple values, and two correct processes may validate different values. In our implementations, we assume the primitive to be tied with a Byzantine agreement instance.
%\ayaz{I am not sure how to properly explain this, basically we need access to some value which is valid as we may validate before broadcasting}

% This section introduces the ECHO validation broadcast algorithm.
% We start by introducing the reducing broadcast problem ().
% We start by providing the pseudocode of the ECHO algorithm (\Cref{subsection:echo_pseudocode}).
% Then, we prove its correctness and complexity (\Cref{subsection:echo_proof}).

\subsection{Implementation for $n = 3t + 1$ Without Any Cryptography} \label{subsection:validation_broadcast_basic_implementation}

This subsection presents the pseudocode (\Cref{algorithm:echo_basic}) of our implementation that (1) tolerates up to $t$ Byzantine failures among $n = 3t+1$ processes, (2) is secure against a computationally unbounded adversary (i.e., uses no cryptography), and (3) achieves $O(n^2L)$ bit complexity.
Our implementation internally relies on the reducing broadcast primitive~\cite{DBLP:journals/acta/MostefaouiR17} that we introduce below.

\paragraph{Reducing broadcast.}
The reducing broadcast problem is a problem proposed and solved in~\cite{DBLP:journals/acta/MostefaouiR17} that allows each process to broadcast its input value and eventually delivers a value.
Importantly, the goal of reducing broadcast is to reduce the number of different values held by correct processes to a constant.
The specification of the problem is associated with the default value $\bot_{rd} \notin \mathsf{Value}$.
Reducing broadcast exposes the following interface:
\begin{compactitem}
    \item \textbf{request} $\mathsf{broadcast}(\mathit{val} \in \mathsf{Value})$: a process starts participating by broadcasting value $\mathit{val}$.

    \item \textbf{request} $\mathsf{abandon}$: a process stops participating in reducing broadcast.

    \item \textbf{indication} $\mathsf{deliver}(\mathit{val}' \in \mathsf{Value} \cup \{\bot_{rd}\})$: a process delivers value $\mathit{val}'$ ($\mathit{val}'$ can be $\bot_{rd}$).
\end{compactitem}
We assume that every correct process broadcasts at most once.
The following properties are ensured:
\begin{compactitem}
    \item \emph{Validity:} If all correct processes that broadcast do broadcast the same value, no correct process delivers $\bot_{rd}$.

    \item \emph{Safety:} If a correct process delivers a value $\mathit{val}' \in \mathsf{Value}$ ($\mathit{val}' \neq \bot_{rd}$), then a correct process has broadcast $\mathit{val}'$.

    \item \emph{Reduction:} The number of values (including $\bot_{rd}$) that are delivered by correct processes is at most $6$.

    \item \emph{Termination:} If all correct processes broadcast and no correct process abandons reducing broadcast, then every correct process eventually delivers a value.
\end{compactitem}

\begin{algorithm}
\caption{Implementation for $n = 3t + 1$ without any cryptography: Pseudocode (for process $p_i$)}
\label{algorithm:echo_basic}
\footnotesize
\begin{algorithmic} [1]
\State \textbf{Uses:}
\State \hskip2em Reducing broadcast~\cite{DBLP:journals/acta/MostefaouiR17}, \textbf{instance} $\mathcal{RB}$

\medskip
\State \textbf{Local variables:}
% \State \hskip2em $\mathsf{Value}$ $\mathit{broadcast\_value}_i \gets \bot$
% \State \hskip2em $\mathsf{Boolean}$ $\mathit{reduced}_i \gets \mathit{false}$
\State \hskip2em $\mathsf{Map}(\mathsf{Value} \cup \{\bot_{rd}\} \to \mathsf{Boolean})$ $\mathit{echo}_i \gets \{\mathit{false}, \mathit{false}, ..., \mathit{false}\}$

\medskip
\State \textbf{Local functions:}
\State \hskip2em $\mathsf{echo}(\mathit{val}) \gets $ the number of processes that sent $\langle \textsc{echo}, \mathit{val} \rangle$ messages received by process $p_i$

% \State \hskip2em $\mathsf{num\_echo}(\mathit{val} \in \mathsf{Value} \cup \{\bot_{rd}\}) \gets $ the total number of $\langle \textsc{echo}, \mathit{val} \rangle$ messages received from \emph{different} processes
\State \hskip2em $\mathsf{total\_echo} \gets$ the number of processes that sent \textsc{echo} messages received by process $p_i$
% \sum\limits_{\mathit{val} \in \mathsf{Value} \cup \{\bot_{rd}\}} \mathsf{echo}(\mathit{val})$ 
\State \hskip2em $\mathsf{most\_frequent} \gets \mathit{val} \in \mathsf{Value} \cup \{\bot_{rd}\}$ such that $\mathsf{echo}(\mathit{val}) \geq \mathsf{echo}(\mathit{val}')$, for every $\mathit{val}' \in \mathsf{Value} \cup \{\bot_{rd}\}$

\medskip
\State \textbf{upon} $\mathsf{broadcast}(\mathit{val}_i \in \mathsf{Value})$: \label{line:echo_broadcast}
% \State \hskip2em $\mathit{broadcast\_value}_i \gets \mathit{val}_i$
\State \hskip2em \textbf{invoke} $\mathcal{RB}.\mathsf{broadcast}(\mathit{val}_i)$ \label{line:echo_reducing_broadcast}

\medskip
\State \textbf{upon} $\mathcal{RB}.\mathsf{deliver}(\mathit{val} \in \mathsf{Value} \cup \{ \bot_{rd} \})$: \label{line:echo_reducing_deliver}
\State \hskip2em \textbf{if} $\mathit{echo}_i[\mathit{val}] = \mathit{false}$:
\State \hskip4em $\mathit{echo}_i[\mathit{val}] \gets \mathit{true}$
\State \hskip4em \textbf{broadcast} $\langle \textsc{echo}, \mathit{val} \rangle$ \label{line:echo_broadcast_1}

\medskip
\State \textbf{upon} exists $\mathsf{val} \in \mathsf{Value} \cup \{\bot_{rd}\}$ such that $\mathsf{echo}(\mathit{val}) \geq t + 1$ and $\mathit{echo}_i[\mathit{val}] = \mathit{false}$: \label{line:echo_receive_plurality}
\State \hskip2em $\mathit{echo}_i[\mathit{val}] \gets \mathit{true}$
\State \hskip2em \textbf{broadcast} $\langle \textsc{echo}, \mathit{val} \rangle$ \label{line:echo_broadcast_2}

\medskip
\State \textbf{upon} $\mathsf{total\_echo} - \mathsf{echo}(\mathsf{most\_frequent}) \geq t + 1$ and $\mathit{echo}_i[\bot_{rd}] = \mathit{false}$: \label{line:echo_most_frequent}
\State \hskip2em $\mathit{echo}_i[\bot_{rd}] \gets \mathit{true}$
\State \hskip2em \textbf{broadcast} $\langle \textsc{echo}, \bot_{rd} \rangle$ \label{line:echo_broadcast_3}

\medskip
\State \textbf{upon} exists $\mathsf{val} \in \mathsf{Value} \cup \{\bot_{rd}\}$ such that $\mathsf{echo}(\mathit{val}) \geq 2t + 1$ for the first time:
\BlueComment{only if $p_i$ has previously broadcast}
\label{line:echo_receive_quorum}
\State \hskip2em \textbf{trigger} $\mathsf{completed}$ \label{line:echo_trigger_completed}

\medskip
\State \textbf{upon} exists $\mathit{val} \in \mathsf{Value} \cup \{\bot_{rd}\}$ such that $\mathsf{echo}(\mathit{val}) \geq t + 1$ for the first time: \label{echo_receive_plurality_2}\BlueComment{can be triggered anytime}
\State \hskip2em \textbf{if} $\mathit{val} = \bot_{rd}$:
\State \hskip4em $\mathit{val} \gets p_i$'s proposal to the Byzantine agreement \label{line:echo_validate_broadcast}
\State \hskip2em \textbf{trigger} $\mathsf{validate}(\mathit{val})$ \label{line:echo_trigger_validate}

\end{algorithmic}
\end{algorithm}

\paragraph{Proof of correctness.}
We start by proving strong validity.

\begin{theorem} [Strong validity]
\Cref{algorithm:echo_basic} satisfies strong validity.
\end{theorem}
\begin{proof}
Suppose that all correct processes that broadcast do so with the same value $\mathit{val}$.
Hence, due to the validity and safety properties of reducing broadcast, all correct processes that deliver a value from it deliver $\mathit{val}$.
Therefore, no correct process ever sends an \textsc{echo} message for any other value or $\bot_{rd}$, which proves that a correct process can only validate $\mathit{val}$.
\end{proof}

Next, we prove external validity.

\begin{theorem} [External validity]
\Cref{algorithm:echo_basic} satisfies external validity.
\end{theorem}
\begin{proof}
Consider any correct process $p_i$.
Let $p_i$ receive $t + 1$ $\langle \textsc{echo}, \mathit{val} \rangle$ messages, for some $\mathit{val} \in \mathsf{Value} \cup \{\bot_{rd}\}$.
We now consider two possibilities:
\begin{compactitem}
    \item Let $\mathit{val} = \bot_{rd}$.
    In this case, $p_i$ indeed validates a valid value as its own proposal to the Byzantine agreement is valid.\footnote{Here, we use $p_i$'s proposal to the Byzantine Agreement as $p_i$ may have not broadcast through the Validation Broadcast.}

    \item Let $\mathit{val} \neq \bot_{rd}$.
    In this case, there exists a correct process that has previously delivered $\mathit{val}$ from reducing broadcast.
    Due to the safety property of reducing broadcast, a correct process has broadcast $\mathit{val}$.
    Therefore, $\mathit{val}$ is valid as no correct process broadcasts an invalid value using \Cref{algorithm:echo_basic}.
\end{compactitem}
External validity is satisfied.
\end{proof}

The following theorem proves integrity.

\begin{theorem} [Integrity]
\Cref{algorithm:echo_basic} satisfies integrity.
\end{theorem}

\begin{proof}
    Follows immediately from the fact that the check at line~\ref{line:echo_receive_quorum} is only performed if $p_i$ has previously broadcast a value.
\end{proof}

Next, we prove termination.

\begin{theorem} [Termination]
\Cref{algorithm:echo_basic} satisfies termination.
\end{theorem}
\begin{proof}
Assuming that all correct processes propose and no correct process ever abandons \Cref{algorithm:echo_basic}, all correct processes eventually deliver a value from reducing broadcast (due to its termination property).
At this point, we separate two possibilities:
\begin{compactitem}
    \item Let there exist a value $\mathit{val} \in \mathsf{Value} \cup \{\bot_{rd}\}$ such that at least $t + 1$ correct processes deliver $\mathit{val}$ from reducing broadcast.
    In this case, all correct processes eventually broadcast an \textsc{echo} message for $\mathit{val}$ (line~\ref{line:echo_broadcast_2}), which means that all correct processes eventually receive $2t + 1$ \textsc{echo} messages for $\mathit{val}$ and complete \Cref{algorithm:echo_basic}.

    \item Otherwise, every correct processes eventually sends an \textsc{echo} message for $\bot_{rd}$ (line~\ref{line:echo_broadcast_3}).
    Thus, all correct processes receive $2t + 1$ \textsc{echo} messages for $\bot_{rd}$ in this case.
\end{compactitem}
Termination is satisfied.
\end{proof}

Finally, we prove totality.

\begin{theorem} [Totality]\label{thm:echo-basic-totality}
\Cref{algorithm:echo_basic} satisfies totality.
Concretely, if a correct process receives a $\mathsf{completed}$ indication at time $\tau$, then every correct process validates a value by time $\max(\tau, \text{GST}) + \delta$.
\end{theorem}

\begin{proof}
    Let $p_i$ be a correct process that receives a \textsf{completed} indication at time $\tau$. Then $p_i$ must have received $2t+1$ matching \textsc{echo} messages for some value $val \in \mathsf{Value}\cup\{\bot_{rd}\}$ by time $\tau$. At least $t+1$ of those messages are from correct processes and thus are received by all correct processes by $\max(\text{GST},\tau) + \delta$. Thus, every correct process validates $val$ by $\max(\text{GST},\tau) + \delta$.
\end{proof}

\paragraph{Proof of complexity.}

We now prove that the bit complexity of \Cref{algorithm:echo_basic} is $O(n^2L)$.

\begin{theorem} [Complexity]
Correct processes send $O(n^2L)$ bits while executing \Cref{algorithm:echo_basic}.
\end{theorem}
\begin{proof}
Each correct process broadcasts $O(1)$ \textsc{echo} messages (ensured by the reduction property of reducing broadcast), each with $O(L)$ bits.
Therefore, correct processes send $O(n^2L)$ bits via \textsc{echo} messages.
As $O(n^2L)$ bits are sent while executing the reducing broadcast primitive (see~\cite{DBLP:journals/acta/MostefaouiR17}), correct processes do send $O(n^2L) + O(n^2L) = O(n^2L)$ bits while executing \Cref{algorithm:echo_basic}.
\end{proof}

\subsection{Hash-Based Implementation for $n = 3t + 1$ for Long Values}
\label{subsection:validation_bcast_long_3_4}

This subsection presents the pseudocode (\Cref{algorithm:validation_broadcast_long_3_4}) of our implementation that (1) solves the problem among $n=3t+1$,
%or $n=4t+1$ processes (depending on the specific implementation of the internal building blocks), 
 out of which $t$ can be Byzantine, (2) internally utilizes a collision-resistant hash function, and (3) exchanges $O(nL + n^2 \kappa)$ bits,
 %$O(nL + n^2 \log(n) \kappa)$ bits when $n=3t+1$ and $O(nL + n^2 \kappa)$ bits when $n=4t+1$, 
  where $\kappa$ is the size of a hash value (see \Cref{subsection:longreb_crypto_primitives}). Our implementation internally utilizes (1) the rebuilding broadcast primitive (see \Cref{section:rebuilding_broadccast}) and (2) the validation broadcast primitive for small input (see \Cref{subsection:validation_broadcast_basic_implementation}). Note that, by abuse of notation, in \Cref{algorithm:validation_broadcast_long_3_4}, we use $\bot$ to denote both $\bot_{\mathit{reb}}$ (the default value of rebuilding broadcast) and $\bot_{\mathit{rd}}$ (the default value of reducing broadcast).

\begin{algorithm}
\caption{Validation broadcast for long values assuming $n = 3t + 1$: Pseudocode (for process $p_i$)}
\label{algorithm:validation_broadcast_long_3_4}
\footnotesize
\begin{algorithmic} [1] 
\State \textbf{Uses:}
\State \hskip2em Rebuilding broadcast, \textbf{instance} $\mathcal{RB}$ \BlueComment{see \Cref{section:rebuilding_broadccast}}
\State \hskip2em Validation broadcast, \textbf{instance} $\mathcal{VB}$ \BlueComment{see \Cref{subsection:validation_broadcast_basic_implementation}; hash values are broadcast}

\medskip
% \State \textbf{Local variables:}
% \State \hskip2em $\mathsf{Hash\_Value}$ $\mathcal{H}_i \gets \bot$
% \State \hskip2em $\mathsf{Boolean}$ $\mathit{delivered}_i \gets \mathit{false}$
% \State \hskip2em $\mathsf{Map}(\mathsf{Hash\_Value} \to \mathsf{Boolean})$ $\mathit{rebuilt}_i \gets \{\mathit{false}, \mathit{false}, ..., \mathit{false} \}$

\medskip
\State \textbf{upon} $\mathsf{broadcast}(\mathit{val}_i \in \mathsf{Value})$: \label{line:validation_broadcast_long_propose}

\State \hskip2em \textbf{invoke} $\mathcal{RB}.\mathsf{broadcast}(\mathit{val}_i)$ \label{line:validation_broadcast_long_broadcast}

\medskip
\State \textbf{upon} $\mathcal{RB}.\mathsf{deliver}(\mathit{val}' \in \mathsf{Value} \cup \{\bot\})$: \label{line:validation_broadcast_long_deliver_rb}
\State \hskip2em \textbf{if} $\mathit{val}' \neq \bot$:
\State \hskip4em \textbf{invoke} $\mathcal{VB}.\mathsf{broadcast}(\mathsf{hash}(\mathit{val}'))$ \label{line:validation_broadcast_long_propose_aw}
\State \hskip2em \textbf{else:}
\State \hskip4em \textbf{invoke} $\mathcal{VB}.\mathsf{broadcast}(\bot)$

\medskip
\State \textbf{upon} $\mathcal{VB}.\mathsf{completed}$:
\State \hskip2em \textbf{trigger} $\mathsf{completed}$

\medskip
\State \textbf{upon} exists $\mathcal{H} \in \mathsf{Hash\_Value} \cup \{\bot\}$ such that $\mathsf{echo}(\mathit{val}) \geq t + 1$ for the first time:\BlueComment{echoes inside $\mathcal{VB}$ instance. can be triggered anytime}\label{line:echos-from-VB}
\State \hskip2em \textbf{if} $\mathcal{H} = \bot$:
\State \hskip4em \textbf{trigger} $\mathsf{validate}(p_i$'s proposal to the Byzantine agreement$)$\label{line:validate-proposal}
\State \hskip2em \textbf{else:}
\State \hskip4em \textbf{wait for} $\mathcal{RB}.\mathsf{rebuild}(\mathit{val}' \in \mathsf{Value})$ such that $\mathsf{hash}(\mathit{val}') = \mathcal{H}$\label{line:wait-for-hash}
\State \hskip4em \textbf{trigger} $\mathsf{validate}(\mathit{val}')$\label{line:validate-after-hash}
\end{algorithmic} 
\end{algorithm}

\paragraph{Proof of correctness}
In this section, we rely on the following lemmas.

\begin{lemma}\label{lem:validate-non-bottom}
In \Cref{algorithm:validation_broadcast_long_3_4}, if the check at line~\ref{line:echos-from-VB} is triggered at a correct process for a non-$\bot_{rd}$ value $val$, then $val$ was previously $\mathcal{VB}$-broadcast by a correct process.
\end{lemma}

\begin{proof}
Examine \Cref{algorithm:echo_basic}. Let $p$ be a correct process for which the check at line~\ref{echo_receive_plurality_2} is triggered for a non-$\bot_{rd}$ value $val$. Then $p$ received at least $t+1$ matching \textsc{echo} messages for $val$, at least one of which is from a correct process. Therefore, at least one correct process has $\mathcal{RB}$-delivered $val$. By $\mathcal{RB}$'s validity and safety properties, some correct process has $\mathcal{RB}$-broadcast $val$, which means that some correct process has invoked $\mathsf{broadcast}(val)$ in \Cref{algorithm:echo_basic}.
\end{proof}

% \jovan{I am not sure I unders}

\begin{lemma}\label{lem:validate-thus-trigger}
In \Cref{algorithm:validation_broadcast_long_3_4}, the inner $\mathcal{VB}$ instance validates $\mathcal{H}$ only if the check at line~\ref{line:echos-from-VB} is triggered for $\mathcal{H}$.
\end{lemma}
\begin{proof}
Follows immediately from \Cref{algorithm:echo_basic}.
\end{proof}

\begin{lemma}\label{lem:trigger-thus-validate}
In \Cref{algorithm:validation_broadcast_long_3_4}, if the check at line~\ref{line:echos-from-VB} is triggered for $\mathcal{H}$, then $\mathcal{VB}$ validates a hash value. Furthermore, if $\mathcal{H} \ne \bot_{rd}$, then $\mathcal{VB}$ validates $\mathcal{H}$.
\end{lemma}
\begin{proof}
Follows immediately from \Cref{algorithm:echo_basic}.
\end{proof}

\begin{theorem}[Strong Validity]
    \Cref{algorithm:validation_broadcast_long_3_4} satisfies strong validity.
\end{theorem}

\begin{proof}
Suppose that all correct processes that broadcast do so with the same value $v$. By the strong validity and safety properties of rebuilding broadcast, any correct process that delivers from rebuilding broadcast, delivers $v$ and thus proposes $\mathsf{hash}(v)$ to the inner validation broadcast instance $\mathcal{VB}$. By the strong validity of the $\mathcal{VB}$ instance, all correct processes that validate some hash value from $\mathcal{VB}$, validate $\mathsf{hash}(v)$, and by \Cref{lem:validate-thus-trigger}, the check at line~\ref{line:echos-from-VB} is triggered for $\mathcal{H} = \mathsf{hash}(v)$. Finally, by the collision-resistance of the hash function, no correct process can rebuild some value $v' \ne v$ from $\mathcal{RB}$ such that $\mathsf{hash}(v') = \mathsf{hash}(v)$ at line~\ref{line:wait-for-hash}, so no correct process can validate $v' \ne v$ at line~\ref{line:validate-after-hash}.    
\end{proof}

\begin{theorem}[External Validity]
    \Cref{algorithm:validation_broadcast_long_3_4} satisfies external validity.
\end{theorem}

\begin{proof}
Let $p_i$ be a correct process that validates a value $v$. We distinguish two cases:
\begin{compactitem}
    \item $p_i$ validates $v$ at line~\ref{line:validate-proposal}. Then $v$ is $p_i$'s proposal to the Byzantine agreement, which is valid.
    \item $p_i$ validates $v$ at line~\ref{line:validate-after-hash}. 
    Hence, a correct process has previously delivered a value $v$ whose hash value is $\mathcal{H}$ from $\mathcal{RB}$.
    Therefore, due to the safety property of $\mathcal{RB}$, a correct process has previously broadcast $v$ using $\mathcal{RB}$ (and proposed to the validation broadcast primitive).
    As no correct process proposes an invalid value, $v$ is valid.

    % Then, the check at line~\ref{line:echos-from-VB} has triggered. By \Cref{lem:trigger-thus-validate}, $p_i$ $\mathcal{VB}$-validates $\mathsf{hash}(v)$. By the external validity of $\mathcal{VB}$, $\mathsf{hash}(v)$ must be the hash of a valid value, and thus $v$ is valid.
\end{compactitem}
Therefore, the theorem holds.
\end{proof}

\begin{theorem}[Integrity]
    \Cref{algorithm:validation_broadcast_long_3_4} satisfies integrity.
\end{theorem}

\begin{proof}
Let $p_i$ be a correct process that receives a \textsf{completed} indication. By the integrity of $\mathcal{VB}$, $p_i$ must have broadcast on $\mathcal{VB}$, and thus $p_i$ must have delivered from $\mathcal{RB}$. By the integrity of $\mathcal{RB}$, $p_i$ must have broadcast on $\mathcal{RB}$, and thus must have invoked \textsf{broadcast}.
\end{proof}

\begin{theorem}[Termination]
    \Cref{algorithm:validation_broadcast_long_3_4} satisfies termination.
\end{theorem}

\begin{proof}
    Follows immediately from the termination property of $\mathcal{RB}$ and $\mathcal{VB}$.
\end{proof}

\begin{theorem}[Totality]\label{thm:validation_broadcast_long_3_4-totality}
    \Cref{algorithm:validation_broadcast_long_3_4} satisfies totality.
\end{theorem}

\begin{proof}[Proof of \Cref{thm:validation_broadcast_long_3_4-totality}]
Suppose some correct process receives a \textsf{completed} indication at time $\tau$, then it must have received a \textsf{completed} indication from $\mathcal{VB}$ at $\tau$. By the totality property of $\mathcal{VB}$ and the proof of \Cref{thm:echo-basic-totality}, all correct processes validate some hash value from $\mathcal{VB}$ by time $\max(\text{GST},\tau) + \delta$. Thus, by \Cref{lem:validate-thus-trigger}, the check at line~\ref{line:echos-from-VB} triggers for some $\mathcal{H}_i$ at every correct process $p_i$ by time $\max(\text{GST},\tau) + \delta$.

If $\mathcal{H}_i = \bot_{rd}$, then $p_i$ validates its own proposal by time $\max(\text{GST},\tau) + \delta$. Otherwise, by \Cref{lem:validate-non-bottom}, $\mathcal{H}_i$ was $\mathcal{VB}$-broadcast by some correct process $p_j$ at time $\tau' \leq \max(\text{GST},\tau) + \delta$. Thus, $\mathcal{H}_i$ must be the hash of some value $v_i$, which $p_j$ $\mathcal{RB}$-delivered at time $\tau'$. By the rebuilding validity of $\mathcal{RB}$, $p_i$ must rebuild $v_i$ at line~\ref{line:wait-for-hash} by time $\max(\text{GST},\tau') + \delta \leq \max(\text{GST},\tau) + 2\delta$ and thus will  validate $v_i$ by $\max(\text{GST},\tau) + 2\delta$.
\end{proof}

\paragraph{Proof of complexity.}
We next prove the complexity of \Cref{algorithm:validation_broadcast_long_3_4}.

\begin{theorem}
\Cref{algorithm:validation_broadcast_long_3_4} exchanges $O(nL + n^2\kappa)$ bits.% (1) $O(nL + n^2\log(n)\kappa)$ bits when $n=3t+1$, or (2) $O(nL + n^2\kappa)$ bits when $n=4t+1$.
\end{theorem}
\begin{proof}
Correct processes only exchange bits as part of the $\mathcal{RB}$ and $\mathcal{VB}$ instances. Correct processes $\mathcal{RB}$-broadcast at most an $L$-sized value, and $\mathcal{VB}$-broadcast at most a $\kappa$-sized value (where $\kappa$ is the length of a hash). Thus, correct processes exchange $O(nL + n^2\kappa + n^2\kappa) = O(nL + n^2\kappa)$ bits 
%(1) $O(nL + n^2\log(n)\kappa + n^2\kappa) = O(nL + n^2\log(n)\kappa)$ bits when $n=3t+1$, and (2) $O(nL + n^2\kappa + n^2\kappa) = O(nL + n^2\kappa)$ bits when $n=4t+1$
(see \Cref{section:rebuilding_broadccast} and \Cref{subsection:validation_broadcast_basic_implementation}).
\end{proof}

\input{appendix/validation_broadcast_ITS}
