# Supplementary material for: Partial Synchrony for Free? New Upper Bounds for Byzantine Agreement
Source: arXiv:2402.10059 source file (2024-10-23)
Supplement: Supplementary file 17 [file graded_consensus_concrete_implementations.tex]

\section{Graded Consensus: Concrete Implementations to be Employed in \name}

This section provides concrete implementations of the graded consensus primitive that we employ in \name to yield Byzantine agreement algorithms with various bit complexity introduced in \Cref{subsection:concrete_algorithms}.
We start by recalling the definition of graded consensus (\Cref{app:graded-consensus-definition}).
We then briefly introduce a specific implementation of graded consensus proposed by Attiya and Welch~\cite{AttiyaWelch23} (\Cref{subsection:aw_graded_consensus_algorithm}).
Finally, we present two implementations that achieve improved bit complexity for long values. Details about these two implementations can be found in \Cref{tab:graded-consensus-summary} below.
% (1) the first one assumes $n = 3t + 1$ or $n = 4t + 1$ and is safe only against a computationally bounded adversary (\Cref{subsection:graded_consensus_bounded}), and (2) the second one assumes $n = 5t + 1$ and is safe against a computationally unbounded adversary (\Cref{subsection:its_graded_consensus}).

\begin{table}[ht]
\centering
\begin{tabular}{ |p{2.4cm}|p{2.7cm}|p{1.3cm}|p{1.4cm}|p{2.1cm}|p{1.6cm}|  }
 \hline
 \centering Algorithm & \centering Exchanged bits & \centering Async. rounds & \centering Resilience & 
\centering Cryptography \tabularnewline
 \hline
 \hline

\centering \textbf{\textsc{\Cref{algorithm:graded_consensus_long_3_4}}} (\Cref{subsection:graded_consensus_bounded})     & \centering $O(nL + n^2\log(n)\kappa)$ & \centering 11 & \centering $3t+1$ & \centering Hash \tabularnewline

 \hline

 \centering \textbf{\textsc{\Cref{algorithm:graded_consensus_long_3_4}}} (\Cref{subsection:graded_consensus_bounded})     & \centering $O(nL + n^2\kappa)$ & \centering 11 & \centering $4t+1$ & \centering Hash  \tabularnewline

 \hline

 \centering \textbf{\textsc{\Cref{algorithm:its_graded_consensus}}} (\Cref{subsection:its_graded_consensus})                 & \centering $O(nL + n^2\log(n))$ & \centering 14 & \centering $5t+1$ & \centering None  \tabularnewline
 \hline
\end{tabular}
    \caption{Relevant aspects of the two asynchronous graded consensus algorithms we propose.
    \\($L$ denotes the bit-size of a value, whereas $\kappa$ denotes the bit-size of a hash value.)}
\label{tab:graded-consensus-summary}
\end{table}

\subsection{Graded Consensus: Definition and Properties}\label{app:graded-consensus-definition}
First we recall the definition of graded consensus~\cite{AttiyaWelch23,DBLP:journals/siamcomp/FeldmanM97}, also known as Adopt-Commit~\cite{DBLP:journals/jpdc/Delporte-Gallet21,DBLP:journals/siamcomp/MostefaouiRRT08}. It is a problem in which processes propose their input value and then decide on some value with some binary grade.
Formally, graded consensus exposes the following interface:
\begin{compactitem}
    \item \textbf{request} $\mathsf{propose}(v \in \mathsf{Value})$: a process proposes value $v$.

    \item \textbf{request} $\mathsf{abandon}$: a process stops participating in graded consensus.

    \item \textbf{indication} $\mathsf{decide}(v' \in \mathsf{Value}, g' \in \{0, 1\})$: a process decides value $v'$ with grade $g'$.
\end{compactitem}
Every correct process proposes at most once and no correct process proposes an invalid value.
Importantly, not all correct processes are guaranteed to propose to graded consensus.
The graded consensus problem requires the following properties to hold:
\begin{compactitem}
    \item \emph{Strong validity:} If all correct processes that propose do so with the same value $v$ and a correct process decides a pair $(v', g')$, then $v' = v$ and $g' = 1$.

    \item \emph{External validity:} If any correct process decides a pair $(v', \cdot)$, then $\mathsf{valid}(v') = \mathit{true}$.

    \item \emph{Consistency:} If any correct process decides a pair $(v, 1)$, then no correct process decides a pair $(v' \neq v, \cdot)$.

    \item \emph{Integrity:} No correct process decides more than once.

    \item \emph{Termination:} If all correct processes propose and no correct process abandons graded consensus, then every correct process eventually decides.
\end{compactitem}

\subsection{Attiya-Welch Graded Consensus Algorithm} \label{subsection:aw_graded_consensus_algorithm}

The Attiya-Welch algorithm~\cite{AttiyaWelch23} is an asynchronous (tolerating unbounded message delays) graded consensus algorithm that (1) operates among $n = 3t + 1$ processes while tolerating up to $t$ Byzantine ones, (2) exchanges $O(n^2L)$ bits in the worst case (when each value consists of $L$ bits), and (3) terminates in $9$ asynchronous rounds.
Importantly, in addition to strong validity, external validity, consistency, integrity and termination (as defined in \Cref{app:graded-consensus-definition}), the Attiya-Welch implementation ensures the following:
\begin{compactitem}
    \item \emph{Safety:} If any correct process decides a pair $(\mathit{val}', \cdot)$, then $\mathit{val}'$ has been proposed by a correct process.
\end{compactitem} 

\subsection{Hash-Based Implementation for $n = 3t + 1$ and $n = 4t + 1$} \label{subsection:graded_consensus_bounded}

This subsection presents the pseudocode (\Cref{algorithm:graded_consensus_long_3_4}) of our graded consensus algorithm that (1) solves the problem among $n = 3t + 1$ or $n = 4t + 1$ processes (depending on the specific implementation of the internal building blocks), out of which $t$ can be Byzantine, (2) internally utilizes a collision-resistant hash function, and (3) exchanges $O(nL + n^2\log(n)\kappa)$ bits when $n = 3t + 1$ and $O(nL + n^2\kappa)$ bits when $n = 4t + 1$, where $\kappa$ is the size of a hash value (see \Cref{subsection:longreb_crypto_primitives}).
Our implementation internally utilizes (1) the rebuilding broadcast primitive (see \Cref{section:rebuilding_broadccast}), and (2) the Attiya-Welch graded consensus algorithm (see \Cref{subsection:aw_graded_consensus_algorithm}).

\begin{algorithm}
\caption{Graded consensus for long values assuming $n = 3t + 1$ or $n = 4t + 1$: Pseudocode (for process $p_i$)}
\label{algorithm:graded_consensus_long_3_4}
\footnotesize
\begin{algorithmic} [1] 
\State \textbf{Uses:}
\State \hskip2em Rebuilding broadcast, \textbf{instance} $\mathcal{RB}$ \BlueComment{see \Cref{section:rebuilding_broadccast}}
\State \hskip2em Attiya-Welch graded consensus~\cite{AttiyaWelch23}, \textbf{instance} $\mathcal{AW}$ \BlueComment{see \Cref{subsection:aw_graded_consensus_algorithm}; hash values are proposed and decided}

\medskip
\State \textbf{Local variables:}
\State \hskip2em $\mathsf{Value}$ $\mathit{proposal}_i \gets \bot$
% \State \hskip2em $\mathsf{Hash\_Value}$ $\mathcal{H}_i \gets \bot$
% \State \hskip2em $\mathsf{Boolean}$ $\mathit{delivered}_i \gets \mathit{false}$
% \State \hskip2em $\mathsf{Map}(\mathsf{Hash\_Value} \to \mathsf{Boolean})$ $\mathit{rebuilt}_i \gets \{\mathit{false}, \mathit{false}, ..., \mathit{false} \}$

\medskip
\State \textbf{upon} $\mathsf{propose}(\mathit{val}_i \in \mathsf{Value})$: \label{line:graded_consensus_long_propose}
\State \hskip2em $\mathit{proposal}_i \gets \mathit{val}_i$
\State \hskip2em \textbf{invoke} $\mathcal{RB}.\mathsf{broadcast}(\mathit{val}_i)$ \label{line:graded_consensus_long_broadcast}

\medskip
\State \textbf{upon} $\mathcal{RB}.\mathsf{deliver}(\mathit{val}' \in \mathsf{Value} \cup \{\bot_{\mathit{reb}}\})$: \label{line:graded_consensus_long_deliver_rb}
\State \hskip2em \textbf{if} $\mathit{val}' \neq \bot_{\mathit{reb}}$:
\State \hskip4em \textbf{invoke} $\mathcal{AW}.\mathsf{propose}(\mathsf{hash}(\mathit{val}'))$ \label{line:graded_consensus_long_propose_aw}
\State \hskip2em \textbf{else:}
\State \hskip4em \textbf{invoke} $\mathcal{AW}.\mathsf{propose}(\bot_{\mathit{reb}})$

\medskip
\State \textbf{upon} $\mathcal{AW}.\mathsf{decide}(\mathcal{H} \in \mathsf{Hash\_Value} \cup \{\bot_{\mathit{reb}}\}, g \in \{0, 1\})$: \label{line:graded_consensus_long_decide_aw}
\State \hskip2em \textbf{if} $\mathcal{H} = \bot_{\mathit{reb}}$:
\State \hskip4em \textbf{trigger} $\mathsf{decide}(\mathit{proposal}_i, 0)$ \label{line:graded_consensus_long_decide_1}
\State \hskip2em \textbf{else:}
\State \hskip4em \textbf{wait for} $\mathcal{RB}.\mathsf{rebuild}(\mathit{val}' \in \mathsf{Value})$ such that $\mathsf{hash}(\mathit{val}') = \mathcal{H}$
\State \hskip4em \textbf{trigger} $\mathsf{decide}(\mathit{val}', g)$ \label{line:graded_consensus_long_decide}
\end{algorithmic} 
\end{algorithm}

\paragraph{Proof of correctness.}
We start by proving the strong validity property.

\begin{theorem} [Strong validity]
\Cref{algorithm:graded_consensus_long_3_4} satisfies strong validity.
\end{theorem}
\begin{proof}
Suppose that all correct processes that propose to graded consensus do so with the same value $\mathit{val}$.
Hence, all correct processes that broadcast their proposal via the rebuilding broadcast primitive do so with value $\mathit{val}$ (line~\ref{line:graded_consensus_long_broadcast}).
Therefore, every correct process that delivers a value from the rebuilding broadcast primitive does deliver value $\mathit{val} \neq \bot_{\mathit{reb}}$ (due to the strong validity and safety properties of rebuilding broadcast primitive), which further implies that all correct processes that propose to the Attiya-Welch graded consensus algorithm do so with hash value $\mathcal{H} = \mathsf{hash}(\mathit{val})$ (line~\ref{line:graded_consensus_long_propose_aw}).
Due to the strong validity property of the Attiya-Welch graded consensus algorithm, any correct process $p_i$ that decides from it decides a pair $(\mathcal{H} \neq \bot_{\mathit{reb}}, 1)$ (line~\ref{line:graded_consensus_long_decide_aw}).
The safety property of the Attiya-Welch algorithm ensures that $\mathcal{H}$ has been proposed to the algorithm by a correct process, which implies that a correct process has delivered value $\mathit{val}$ from the rebuilding broadcast primitive (line~\ref{line:graded_consensus_long_deliver_rb}).
Finally, $p_i$ indeed eventually rebuilds $\mathit{val}$ (due to the rebuilding validity of rebuilding broadcast), and decides $(\mathit{val}, 1)$ (line~\ref{line:graded_consensus_long_decide}).
\end{proof}

The following theorem proves the external validity property.

\begin{theorem} [External validity]
\Cref{algorithm:graded_consensus_long_3_4} satisfies external validity.
\end{theorem}
\begin{proof}
Suppose that a correct process $p_i$ decides some value $\mathit{val}'$.
We consider two possibilities:
\begin{compactitem}
    \item Let $p_i$ decide $\mathit{val}'$ at line~\ref{line:graded_consensus_long_decide_1}.
    In this case, $\mathit{val}'$ is the proposal of $p_i$.
    As no correct process proposes an invalid value, $\mathit{val}'$ is a valid value.

    \item Let $p_i$ decide $\mathit{val}'$ at line~\ref{line:graded_consensus_long_decide}.
    Hence, $p_i$ has previously decided $\mathcal{H} = \mathsf{hash}(\mathit{val'})$ from the Attiya-Welch algorithm (line~\ref{line:graded_consensus_long_decide_aw}).
    Due to the safety property of the Attiya-Welch algorithm, a correct process has previously proposed $\mathcal{H}$, which implies that a correct process has delivered $\mathit{val}'$ from the rebuilding broadcast primitive (line~\ref{line:graded_consensus_long_deliver_rb}).
    The safety property of rebuilding broadcast proves that $\mathit{val}'$ has been broadcast via the primitive by a correct process (line~\ref{line:graded_consensus_long_broadcast}), which implies that a correct process has proposed $\mathit{val}'$ to graded consensus (line~\ref{line:graded_consensus_long_propose}).
    As no correct process proposes an invalid value, $\mathit{val}'$ is a valid value.
\end{compactitem}
As $\mathit{val}'$ is a valid value in both possible scenarios, the proof is concluded.
\end{proof}

Next, we prove consistency.

\begin{theorem} [Consistency]
\Cref{algorithm:graded_consensus_long_3_4} satisfies consistency.
\end{theorem}
\begin{proof}
Let $p_i$ be any correct process that decides a pair $(\mathit{val}, 1)$ (line~\ref{line:graded_consensus_long_decide}).
Hence, $p_i$ has previously decided a pair $(\mathcal{H} = \mathsf{hash}(\mathit{val}), 1)$ from the Attiya-Welch algorithm (line~\ref{line:graded_consensus_long_decide_aw}).
Due to the consistency property of the Attiya-Welch algorithm, any correct process that decides from it does decide $(\mathcal{H}, \cdot)$.
Therefore, any correct process that decides does decide $\mathit{val}$ at line~\ref{line:graded_consensus_long_decide}.
\end{proof}

Finally, we prove the termination property.

\begin{theorem} [Termination]
\Cref{algorithm:graded_consensus_long_3_4} satisfies termination.
\end{theorem}
\begin{proof}
Let us assume that all correct processes propose and no correct process ever abandons \Cref{algorithm:graded_consensus_long_3_4}.
In this case, the termination property of the rebuilding broadcast primitive ensures that every correct process eventually delivers a value from it (line~\ref{line:graded_consensus_long_deliver_rb}), and proposes to the Attiya-Welch algorithm (line~\ref{line:graded_consensus_long_propose_aw}).
Similarly, the termination property of the Attiya-Welch algorithm guarantees that every correct process eventually decides from it (line~\ref{line:graded_consensus_long_decide_aw}).
We now separate two cases that can occur at any correct process $p_i$:
\begin{compactitem}
    \item Let $p_i$ decide $\bot_{\mathit{reb}}$ from the Attiya-Welch algorithm.
    Process $p_i$ decides from \Cref{algorithm:graded_consensus_long_3_4} at line~\ref{line:graded_consensus_long_decide_1}, thus satisfying termination.

    \item Let $p_i$ decide $\mathcal{H} \neq \bot_{\mathit{reb}}$ from the Attiya-Welch algorithm.
    In this case, a correct process has previously delivered a value $\mathit{val}$ such that $\mathcal{H} = \mathsf{hash}(\mathit{val})$ from the rebuilding broadcast primitive (line~\ref{line:graded_consensus_long_deliver_rb}).
    Therefore, the rebuilding validity property of rebuilding broadcast ensures that $p_i$ eventually rebuilds $\mathit{val}$ and decides at line~\ref{line:graded_consensus_long_decide}.
\end{compactitem}
As termination is satisfied in both cases, the proof is concluded.
\end{proof}

\paragraph{Proof of complexity.}
We now prove the bit complexity of \Cref{algorithm:graded_consensus_long_3_4}.
Recall that $\kappa$ denotes the size of a hash value.

\begin{theorem} [Complexity]
\Cref{algorithm:graded_consensus_long_3_4} exchanges (1) $O(nL + n^2\log(n)\kappa)$ bits when $n = 3t + 1$, and (2) $O(nL + n^2\kappa)$ bits when $n = 4t + 1$.
\end{theorem}
\begin{proof}
The bit complexity of the Attiya-Welch algorithm is $O(n^2\kappa)$.
When $n = 3t + 1$ and $\textsc{RebLong3}$ (see \Cref{subsection:longreb_3}) is employed in \Cref{algorithm:graded_consensus_long_3_4}, the bit complexity is $O(nL + n^2\log(n)\kappa) + O(n^2\kappa) = O(nL + n^2\log(n)\kappa)$.
When $n = 4t + 1$ and $\textsc{RebLong4}$ (see \Cref{subsection:longreb_4}) is utilized in \Cref{algorithm:graded_consensus_long_3_4}, the bit complexity becomes $O(nL + n^2\kappa) + O(n^2\kappa) = O(nL + n^2\kappa)$.
\end{proof}

\begin{theorem}[Asynchronous rounds]
\Cref{algorithm:graded_consensus_long_3_4} incurs at most 11 asynchronous rounds. 
\end{theorem}
\begin{proof}
Each correct process that participates in \Cref{algorithm:graded_consensus_long_3_4} and does not abandon incurs 2 rounds from the $\mathcal{RB}$ instance (\Cref{theorem:async_rounds_rebuilding_3} and \Cref{theorem:async_rounds_rebuilding_4}), followed by 9 rounds from the $\mathcal{AW}$ instance (\cite{AttiyaWelch23}).
\end{proof}

\input{appendix/graded_consensus_ITS}
