# Supplementary material for: Partial Synchrony for Free? New Upper Bounds for Byzantine Agreement
Source: arXiv:2402.10059 source file (2024-10-23)
Supplement: Supplementary file 18 [file proof_lemma_1.tex]

\section{Formal Proof of Lemma~\ref{lemma:helper_main}} \label{section:proof_helper}

In this section, we formally prove \Cref{lemma:helper_main}.
Recall that \Cref{lemma:helper_main} plays a crucial role in our formalism.

\begin{lemma_helper} [restated formally]
Let $\mathit{val}$ be any solvable validity property and let $\mathcal{A}$ be a Byzantine consensus algorithm with $\mathit{val}$.
Let $\mathcal{E} = (\mathcal{A}, c, \mathcal{F}, \epsilon, \text{GST})$ be any canonical execution of $\mathcal{A}$ such that $\epsilon$ is infinite.
If $v \in \mathcal{V}_O$ is decided in $\mathcal{E}$, then $v \in \bigcap\limits_{c' \in \mathit{sim}(c)} \mathit{val}(c')$.
\end{lemma_helper}
\begin{proof}
By contradiction, suppose that $v \notin \bigcap\limits_{c' \in \mathit{sim}(c)} \mathit{val}(c')$.
Note that $\mathcal{F} \neq \emptyset$, as, otherwise, $v \in \bigcap\limits_{c' \in \mathit{sim}(c)} \mathit{val}(c')$ (given that $\mathit{sim}(c) = \{c\}$ in this case).

Let $c' \in \mathcal{I}$ be an input configuration such that (1) $c' \sim c$, and (2) $v \notin \mathit{val}(c')$.
We aim to construct an execution $\mathcal{E}'$ of $\mathcal{A}$ such that (1) $\mathcal{E}'$ corresponds to $c'$, and (2) $v \notin \mathit{val}(c')$ is decided in $\mathcal{E}'$.

Recall that $\process{c'} \cap \process{c} \neq \emptyset$ (by \Cref{definition:similarity_condition}); let $P$ be any process in $\process{c'} \cap \process{c}$.
We denote by $\epsilon_P$ the prefix of $\epsilon$ such that the last event of $\epsilon_P$ is $\big( P, \mathsf{decide}(v) \big)$ (given that $\epsilon$ is infinite and $\mathcal{A}$ solves the Byzantine consensus problem, $\big( P, \mathsf{decide}(v) \big) \in \epsilon$).
Let $T = \mathsf{time}((P, \mathsf{decide}(v)), \epsilon)$ be the time at which $P$ decides $v$ in $\epsilon$.
% We construct another sequence of events $\epsilon'$ in the following manner:
% \begin{compactenum}
%     \item $\epsilon' \gets \epsilon_P$.
    
%     \item For every process $Q \in \pi(c')$ such that $\big( Q, \mathsf{start} \big) \notin \epsilon_P$:
%     \begin{compactenum}
%         \item $\epsilon' \gets \epsilon' || \big( Q, \mathsf{start} \big)$.
%     \end{compactenum}
% \end{compactenum}
Finally, $\mathcal{E}' = (\mathcal{A}, c', \mathcal{F}' = \Pi \setminus{\process{c'}}, \epsilon' = \epsilon_P, \text{GST}' > T)$.
Moreover, for every event $e \in \epsilon'$, the following holds:
\begin{compactitem}
    \item If $e \in \epsilon_P$, then $\mathsf{time}(e, \epsilon') = \mathsf{time}(e, \epsilon)$.
    
    \item Otherwise, $\mathsf{time}(e, \epsilon') = T$.
\end{compactitem}

To conclude the proof, we show that $\mathcal{E}'$ satisfies the properties of an execution (see \Cref{section:full_model}):
\begin{compactenum}
    \item For every process $P \in \Pi$, $\epsilon'|_P$ is a behavior as (1) $\mathcal{E}$ satisfies this property, and (2) only the $\mathsf{start}$ events are appended to $\epsilon_P$.
    
    \item This property trivially holds as $\epsilon'$ is not infinite.
    
    \item For every process $P \in \pi(c) \cap \pi(c')$, the proposal of $P$ is identical in both $c$ and $c'$ (thus, in $\mathcal{E}$ and $\mathcal{E}'$).
    Moreover, for every process $Q \in \pi(c') \setminus{\pi(c)}$, only $\big( Q, \mathsf{start} \big)$ event belongs to $\epsilon'$.
    
    \item Due to the construction of $\mathcal{E}'$, $\mathsf{valid}(\mathcal{A}, P, \epsilon'|_P) = \mathit{true}$, for every process $P \in \Pi$.
    
    \item This property is satisfied since (1) it is satisfied by $\mathcal{E}$, and (2) only the $\mathsf{start}$ events are appended to $\epsilon_P$.
    
    \item This property is trivially satisfied as $\text{GST}' > \mathsf{time}( \epsilon'[|\epsilon'|], \epsilon')$.
    % by construction: every process $P \in \pi(c')$ starts by GST.
    
    \item This property trivially holds as $\epsilon'$ is not infinite.
    
    \item This property trivially holds for $\text{GST}' > T$ (i.e., GST is ``shifted'' to the future).
    
    \item This property trivially holds for $\text{GST}' > T$ (i.e., GST is ``shifted'' to the future).
\end{compactenum}
Hence, $\mathcal{E}'$ satisfies the properties introduced in \Cref{section:full_model}.
Therefore, $v \notin \mathit{val}(c')$ is decided in $\mathcal{E}'$.
We reach a contradiction with a fact that $\mathcal{A}$ solves the Byzantine consensus problem with $\mathit{val}$.
Thus, the lemma.
\end{proof}
