# Supplementary material for: Partial Synchrony for Free? New Upper Bounds for Byzantine Agreement
Source: arXiv:2402.10059 source file (2024-10-23)
Supplement: Supplementary file 19 [file sota_sync_and_async.tex]

\iffalse

\begin{table}[h!]
    \footnotesize
    \centering
    \begin{tabular}{|c|c|c|c|c|c|c|}
        \hline
        \textbf{Protocol} & \textbf{Relaxation to $\mathcal{M}_{\mathit{worst}}$} & \textbf{Security} & \textbf{Resiliency} & \textbf{Latency} & \textbf{Comm} & \textbf{Remarks} \\
        \hline
        HPZ \cite{huang2023byzantine} & None & Perfect & $< n/(3 + \epsilon)$ & $O(n^4/\epsilon^{8})$ & $O(n^6/\epsilon^{8})$ & binary \\
        \hline
        HPZ \cite{huang2023byzantine} & None & Perfect & $< n/3$ & $\tilde{O}(n^{12})$ & $\tilde{O}(n^{14})$ & binary \\
        \hline \hline
        KKKSS \cite{KKKSS08,KKKSS10} & Static Adv. & $1/\mathit{polylog}(n)$ & $< n/(3 + \epsilon)$ & $O(\log^{27}(n))$ & $\tilde{O}(n^2)$ & LE \\
        \hline
        KKKSS \cite{KKKSS08,KKKSS10} & Static Adv. &  $1/\mathit{poly}(n)$ & $< n/(3 + \epsilon)$ & $2^{\Theta(\log^8(n))}$ & $\tilde{O}(n^2)$ & LE \\
        \hline \hline
        AAKS \cite{AAKS14,AAKS18} & Crash Only & Perfect & $< n/2$ & $\tilde{\Omega}(n)$ & $\tilde{O}(n^2)$ & binary \\
        \hline
        AAKS \cite{AAKS14,AAKS18} & Crash Only & Perfect & $< n/2$ & $\tilde{\Omega}(n)$ & $\tilde{O}(n^3)$ & ACS \\
        \hline \hline
        CMS \cite{CMS85,CMS89} & Static Adv., Omission & Perfect & $< n/3$ & $O(1)$ & $O(n^2)$ & binary \\
        \hline \hline
        AAPS \cite{AAPS23} & Priv. Chan. & Perfect & $< n/4$ & $O(1)$ & $\tilde{O}(n^4)$ &  ACS \\
        \hline
        AAPS \cite{AAPS23} + \cite{ChoudhuryPatra23}'s AISS & Priv. Chan. & $\mathit{neg}(\lambda)$ & $< n/3$ & $O(1)$ & $O(n^6 + \lambda^2 n^5)$ & ACS \\
        \hline
        BCP \cite{BCP18} & Priv. Chan. & Perfect & $< n/3$ & $O(n)$ & $O(n^6)$ & binary \\
        \hline
        BCP \cite{BCP18} & Priv. Chan. & Perfect & $< n/(3+\epsilon)$ & $O(1/\epsilon)$ & $O(n^6)$ & binary \\
        \hline
    \end{tabular}
    \caption{Overview of State-of-the-Art Fully Asynchronous Protocols in Relaxed Models with unbounded adversary}
    \label{tab:state_of_the_art_protocols}
\end{table}

\begin{table}[h!]
    \footnotesize
    \centering
    \begin{tabular}{|c|c|c|c|c|c|}
        \hline
        \textbf{Protocol} & \textbf{Relaxation to $\mathcal{M}_{\mathit{worst}}$} & \textbf{Resiliency} & \textbf{Latency} & \textbf{Comm} & \textbf{Remarks} \\
        \hline
        CDGGKVZ \cite{errorFreeValidated} & None & $< n/3$ & $O(f)$ & $O(nL + n^2\log(n))$ & ES | MVBA \\
        \hline \hline
        GPV \cite{GPV06} & Static Adv. & $< n/(3 + \epsilon)$ & $O(\log(n)/\epsilon^2)$ & $O(n^3)$ &  LE \\
        \hline
        KSSV \cite{KSSV06} + \cite{Gelles23} & Static Adv. & $< n/(3 + \epsilon)$ & $\mathit{polylog}(n)$ & $o(n^2)$ & solves LE \\
        \hline \hline
        HKO \cite{hajiaghayi2024nearly} & Omission & $< n/30$ & $O(\sqrt{n}\log^2(n))$ & $O(n^2\log^3(n))$ & binary \\
        \hline
        HKO \cite{hajiaghayi2024nearly} & Omission & $< n/30$ & $O(\sqrt{n}\log^2(n))$ & $O(Ln^2 +n^3\log^3(n))$ & IC \\
        \hline
        BB \cite{Bar-JosephB98} & Crash & - & $\Omega(\sqrt{n/\log(n)})$ & - & lower bound \\

\hline \hline
        CMS \cite{CMS85,CMS89} & Static Adv., Omission & $< n/3$ & $O(1)$ & $O(n^2)$ & binary \\
        
        \hline \hline
        KS \cite{KingSaia10,King2011} & Priv. Chan. & $< n/(3+\epsilon)$ & $\mathit{polylog(n)}$ & $\tilde{O}(n^{3/2})$ & binary \\
        \hline
        KS \cite{KingSaia10,King2011} & Priv. Chan. & $< n/(3+\epsilon)$ & $\mathit{polylog(n)}$ & $\tilde{O}(Ln^2+n^{5/2})$ & IC \\
        \hline
        AC \cite{AsharovChandramouli24} & Priv. Chan. & $< n/3$ & $O(1)$ & $O(Ln^2+n^3 \log^2(n))$ & IC \\
        \hline
    \end{tabular}
    \caption{Overview of State-of-the-Art Synchronous Protocols in Relaxed Models}
    \label{tab:synchronous_protocols}
\end{table}

\fi

%%%%%%%%%%%%%%%%%%%%%%%%%
%%%%%%%%%%%%%%%%%%%%%%%%%
%%%%%%%%%%%%%%%%%%%%%%%%%
\iffalse
The simulation $\mathsf{CryptoSim}$ (\Cref{algorithm:simulation}) allows the simulation of any synchronous randomized protocol with per-process bit-complexity $\mathcal{B}$ in a partially synchronous environment, maintaining the same round complexity $\mathcal{R}$ and per-process bit-complexity $\max(O(n),\mathcal{B})$. We studied the per-process communication complexity of one flavor of consensus that is $\Omega(n)$ (thus $\Omega(n)$ total communication complexity) after GST in the partially synchronous model handling an unbounded adaptive adversary, even for randomized protocols. However, other problems can be considered such as latency complexity and other agreement problems, such as agreement on a core set (ACS).

For some corresponding problems that only differ on the synchrony assumption, there might be a significant gap between the synchronous and the asynchronous version.

As already said, in the full-information model with an adaptive adversary, the optimally resilient solution of \cite{huang2023byzantine} has a quite discouraging latency $\Omega(n^{12})$ expected latency.
However, in the synchronous counterpart of such a model, we are unaware of efficient protocols.
Let's investigate the possible relaxation. The most natural one is dealing with a static adversary.

Kapron et al. \cite{KKKSS08,KKKSS10} developed a Byzantine Agreement protocol in the asynchronous, full information model, in which the adversary corrupts $f < n/(3 + \epsilon)$ players non-adaptively. Their protocol has different parameterizations, and can achieve agreement in quasipolynomial latency with probability $1 - 1/poly(n)$, or polylogarithmic latency with probability $1 - 1/poly(\log n)$. When these protocols err, they do not satisfy the Agreement and Termination criteria, and may deadlock or terminate without agreement.

Classic asynchronous reductions (\cite{Chor1989,CR93,BenOr1993}) allow asynchronous agreement on a core set (ACS). More concretely, we can use the transformation of \cite{ben1994asynchronous} and the reliable broadcast of \cite{Alhaddad2022} to achieve ACS with communication complexity of $O(n^2 L_{\text{in}} + X_n)$ where $X_n$ denotes the communication complexity of $n$ parallel instances of binary BA with strong validity. Against an unbounded adversary, even assuming private channels, no existing solution does better than \cite{AAPS23} with $\tilde{O}(n^4)$ communication complexity (with a collision-resistant hash function, a cubic solution is possible \cite{das2024asynchronous}). Hence, a cubic information-theoretic partially synchronous ACS can represent a good alternative.

Such a cubic solution can be trivially obtained from any information-theoretic quadratic solutions. This includes solutions with or without private channels, with a static or an adaptive adversary, with arbitrary failures or omission failures only. In the full information model, achieving a satisfying latency against an adaptive adversary is particularly challenging because of the Bar-Joseph-Ben-Or lower bound \cite{Bar-JosephB98}. With omission failures only, \cite{hajiaghayi2024nearly} achieve a near-optimal solution.

In the full information model, achieving a satisfying latency has been more investigated against a static adversary. Goldwasser, Pavlov, and Vaikuntanathan \cite{GPV06} considered a synchronized, full information model in which the adversary corrupts up to $f$ players upfront, that is, it is non-adaptive. They proved that Byzantine Agreement can be solved with resiliency $f < n/(3+\epsilon)$ in $O(\log n/\epsilon^2)$ rounds. Consequently, it is possible to achieve a $O(1)$-round randomized BA protocol in a synchronous full-information network tolerating $t = O(n/(\log n)^{1.58})$ static corruptions.

Another research direction consists of extending the almost-everywhere protocol of King, Saia, Sanwalani, and Vee \cite{KSSV06,king2022corrigendum}. Specifically, their protocol succeeds with all but negligible probability of error and each party speaks to only $\tilde{O}(1)$ other parties (within $\tilde{O}(1)$ many rounds). It can tolerate a $1/3 - \epsilon$ fraction of statically corrupted parties for every constant $\epsilon > 0.3$. However, it fails to achieve correctness. It only achieves so-called almost-everywhere agreement, where $1 - O(\log^{-1} n)$ fraction of the parties reach agreement. Extending almost-everywhere to full agreement (while preserving the efficiency properties) has been a major challenge since then. Information-theoretic results include \cite{braud2013fast,Gelles23}.

Assuming secret channels, synchronous interactive consistency (resp., asynchronous agreement on a core set (ACS)) can be implemented with a constant expected number of rounds, and $O(n^2 L_{\text{in}}) + \tilde{O}(n^3)$ (resp., $\tilde{O}(n^4)$) communication against an unbounded adaptive adversary \cite{AsharovChandramouli24} \cite{AAPS23}.

Let $\mathcal{A}^S$ be a Monte Carlo (resp., (non-necessarily error-free) Las Vegas) synchronous randomized protocol with known round complexity $\mathcal{R}$ (resp., known expected round complexity $\mathcal{R}^e$) and known per-process bit-complexity $\mathcal{B}$ (resp., known expected per-process bit-complexity $\mathcal{B}^e$) that achieves safety with probability $\rho = \Omega(1)$.
Then, $\mathcal{A}^{PS} = \name(\mathcal{A}^S)$
 is an error-free Las Vegas partially synchronous protocol that solves consensus with $O(1)$ expected latency.
Let us note that if $\mathcal{A}^S$ is (non-necessarily error-free) Las Vegas, in the sense that its latency is not fixed, but has the expected value $\mathcal{R}^e$, then a trivial Markov inquality implies that $\Pr[\mathcal{A}^s \text{ terminates after } x\mathcal{R}^e \text{ rounds } ] \leq \frac{1}{x}$. Hence, such a protocol $\mathcal{A}^s$ can be turned into a Monte Carlo protocol $\tilde{\mathcal{A}}^S_x$ with a probability of success $\rho(1-\frac{1}{x})$. We can note that there is no obvious complexity-preserving black-box transformation to turn an asynchronous protocol with a non-zero probability of termination violation (e.g. \cite{KKKSS08,KKKSS10}) into a Las Vegas protocol with probability $1$ of correctness. 


 More concretely, the view sychronizer guarantees \emph{eventual synchronization}: there exists a time $\tau_{\mathit{sync}} \geq \text{GST}$ (\emph{synchronization time}) such that all correct processes are in the same view $V_{\mathit{sync}}$ (\emph{synchronization view}) from time $\tau_{\mathit{sync}}$ to (at least) time $\tau_{\mathit{sync}} + \Delta$, and entered this view within $2\delta$ time from each other.
We denote by $V_{\mathit{sync}}^*$ the smallest synchronization view, whereas $\tau_{\mathit{sync}}^*$ denotes the first synchronization time.
Similarly, $V_{\mathit{max}} \in \{V_{\mathit{sync}}^*, V_{\mathit{sync}}^* -1 \}$ denotes the greatest view entered by a correct process before GST.\footnote{When such a view does not exist, $V_{\mathit{max}}=0$}. We denote by $V_{\mathit{end}}$ the greatest view entered by a correct process before every correct process decides and halts. Finally, $X=1 + V_{\mathit{end}} - V_{\mathit{sync}}^*$ follows a geometric law, i.e. $\Pr[X=k] = \rho(1-\rho)^{k-1}$. Thus $\mathbb{E}(X) = \frac{1}{\rho}$, and $\mathbb{V}ar(X) = \frac{1-\rho}{\rho^2}$.

A remark for a reduction to $n$ instances (e.g., ACS): 
Given $n$ independent geometric random variables $(X_i)_{i \in n}$, each with probability parameter $\rho$, we can bound $E_n = \mathbb{E}(\mathsf{max}(X_i)_{i \in n}))$ by $1+\frac{1}{\lambda}H_n$, with $\lambda = -\log (1-\rho)$, $H_n = \sum_{k=1}\frac{1}{k}$. Moreover, $H_n \sim ln(n)$. 
Hence, if we have a synchronous protcol that solves binary consensus with per-process communication complexity $\mathcal{B}$ and round complexity $\mathcal{R}$, we can solve partially synchronous ACS with per-process communication complexity $\mathsf{max}(n,\mathcal{B})n\log(n)$ and round complexity $\mathcal{R}\log(n)$. My main question is: what about protocols with negligible probability (with $n$) of failure (e.g. \cite{Gelles23}) ? Can we do better ? I will adress this question at the very last moment.

My goal now is to classify all the known sublinear protocols according to their class (Las Vegas vs Monte Carlo), exact $\mathcal{B}$, exact $\mathcal{R}$, relaxation compare to the horrible model of strongly adaptive full information malicious adversary. According to \cite{hajiaghayi2024nearly}, in this too demanding setting, there is no randomized solution that achieves better than a linear latency.

In asynchrony:

\begin{itemize}
    \item \cite{huang2023byzantine}: no relaxation ; latency: $\mathsf{min}(O(n^4/\epsilon^{8}),\tilde{O}(12))$ ; communication $latency * n^2$ ; las vegas security perfect.

    \item \cite{KKKSS08,KKKSS10}: relaxation: static adversary ; Not Las Vegas ; 
    \begin{itemize}
        \item First algorithm: latency: $O(\log^{27}(n))$ ; communication $\tilde{O}(n^2)$ ; probability of correctness violation $1/ \mathit{polylog}(n)$.
        \item Second algorithm: latency: non polynomial ($2^{\Theta(\log^8(n))}$) ; probability of correctness violation $1/ \mathit{poly}(n)$.
    \end{itemize}

    \item relaxation: crash only \cite{AAKS14,AAKS18} $\tilde{\Omega}(n)$ latency and $\tilde{O}(n^2)$ communication complexity, Las Vegas, perfect security. Omission failure can be simulated atop crash failures at the cost of a certain mulitplicative message complexity overhad \cite{AW04}.

    \item relaxation: both static adversary and omission failures \cite{CMS85,CMS89}: Las Vegas, latency: $O(1)$ security: perfect, communication $O(n^2)$

    \item \cite{AAPS23}: relaxation: private channels, problem ACS, type: Las Vegas, latency: $O(1)$
    \begin{itemize}
        \item First algorithm: resiliency: $n/4$, communication $\tilde{O}(n^4)$ security: perfect
        \item Second algorithm: resiliency: $n/3$, security statistical with $\mathit{neg}(\kappa)$ probability of failure, might be possible to achieve something like $O(n^6 + n^5\kappa^2)$ expected communication complexity by plug in the AISS protocol of \cite{ChoudhuryPatra23} (called AVSS in \cite{AAPS23} and \cite{canetti1993fast}) in the tranformation of 
        \cite[Theorem 1.3]{AAPS23}. (The last state-of-the-art peer-reviewed protocol in the same setting achieves $O(n^6)$ complexity and $O(1/\epsilon)$ (resp., $O(n)$) expected latency and $n/(3+\epsilon)$ (resp., $n/3$) resiliency \cite{BCP18}) for binary agreement).
    \end{itemize}
    
\end{itemize}

In synchrony:

\begin{itemize}
    \item \cite{errorFreeValidated}: no relaxation ; latency: $O(f)$ (early stooping), communication $O(n \log(n))$ per process; optimal resiliency $n/3$ ; security: deterministic.

    \item  relaxation: static adversary
    
    \begin{itemize}
        \item \cite{GPV06}: ; latency: $O(\log(n)/\epsilon^2)$ ; resiliency $n/(3+\epsilon)$ ; (claimed ) communication $\tilde{O}(n^2)$ ; (believed) communication $O(n^3)$ ($O(n^2)$ per party) ; probability of correctness violation $1/ \mathit{poly}(n)$. \cite[Lemma 10, page 57]{Vaikuntanathan09} claims a total communication of communication $\tilde{O}(n^2)$, but the first step of protocol $\Pi_{\mathsf{Elect}\text{-}\mathsf{GPV}}$ uses $n$ parallel instances of gradecast (a.k.a. all-to-all gradecast \cite{BG12,ZLC23}) whose best implementation has a bit-complexity which is  quadratic per party, i.e. cubic in total (though a linear improvement for the message complexity counterpart is trivially achievable)\cite{BG12,ZLC23,AsharovChandramouli24}. The contribution of the first step to the communication complexity is ommitted in the proof of \cite[Lemma 10, page 57]{Vaikuntanathan09}.
        Remark: this construction can be used to solves committee election, which then can be used to solve MVBA via \cite{errorFreeValidated} with a quadratic balanced protocol via the committee broadcast of \cite{errorFreeValidated}.

        \item \cite{KSSV06} + \cite{Gelles23,braud2013fast}
        Remark 1: (the main goal of \cite{KSSV06} is to be subquadratic, but it can be trivially made to-everywhere with a all-to-all round (see \cite{Gelles23,braud2013fast} for a sub-quadratic almost-everywhere to everywhere protocol with constant latency)) 
        Remark 2: the construction of \cite{KSSV06} can be used to solves committee election, which then can be used to solve MVBA via \cite{errorFreeValidated} with a quadratic balanced protocol via the committee broadcast of \cite{errorFreeValidated}
        Remark 3: hard to obtain the exact complexity metrics. The almost-everywhere to everywhere protocol of \cite{Gelles23} offers $O(\sqrt{n}\log^14(n))$ communication complexity per party.
    \end{itemize}
    
   

    \item relaxation: omission failures: \cite{hajiaghayi2024nearly} resiliency $n/30$ latency $O(\sqrt{n}log^2(n))$ and communication $O(n^2\log^3(n))$ (balanced ? don't know). Let us note that the Bar-Joseph Ben-Or lower bound \cite{Bar-JosephB98} implies $O(\sqrt{n}/log(n))$ latency and the lower bound of \cite{AbrahamCDNP0S19} implies $n^2$ messages

    \item relaxation: both static adversary and omission failures \cite{CMS85,CMS89}: Las Vegas, latency: $O(1)$ security: perfect, communication $O(n)$ per process

    \item \cite{AsharovChandramouli24}: relaxation: private channels, problem IC, type: Las Vegas, latency: $O(1)$ ; resiliency: optimal $n/3$ ; communication (balanced) $O(n^3 \log^2(n))$ ; security: perfect
    
\end{itemize}
\fi
